# Supplementary material for: Regression Discontinuity Designs Under Interference
Source: arXiv:2410.02727 source file (2026-09-09)
Supplement: Supplementary file 1 [file appendix.tex]

\documentclass[main.tex]{subfiles}
\externaldocument{main}

\begin{document}
\appendix 
\renewcommand\thesection{S.\arabic{section}} % <-- new
\setcounter{theorem}{0}
\setcounter{assumption}{0}
\setcounter{lemma}{0}
\setcounter{corollary}{0}

\renewcommand{\thetheorem}{\thesection.\arabic{theorem}}
\renewcommand{\theassumption}{\thesection.\arabic{assumption}}
\renewcommand{\thelemma}{\thesection.\arabic{lemma}}
\renewcommand{\thecorollary}{\thesection.\arabic{corollary}}

\title{
\vspace{-3em}
Supplementary Material to \qq Regression Discontinuity Designs Under Interference"}
\date{}

\maketitle
\setcounter{page}{1}
\section{Effective Treatment Boundary Derivation}\label{appendix:mainresults}

We provide the derivation of the equality $\Frontier = %\bigcup h(d_i^{d,g}, \bm{d}_{\smallN_i}^{d,g}, d_i^{d',g'}, \bm{d}_{\smallN_i}^{d',g'})$
\bigcup_{\treatspace(d,g) \times \treatspace(d',g')} \ell(\bm{d}_{i\smallN_i}^{d,g}, \bm{d}_{i\smallN_i}^{d',g'})$ in Subsection~\ref{sec:etb}.  
%In the following, we assume that all interference sets have the same cardinality. 
The derivation uses the fact that given the individual treatment rule in Eq.~\eqref{eq:indrule}, each element $\ddpoint[d,g] \in \treatspace(d,g)$ can be mapped back to the set $\scorespace(\ddpoint[d,g]) = \{\ppoint \in \scorespace : \forall z \in (\{i\}\cup \mathcal{S}_i),\; x_z \geq c \; \text{if}\; d_z^{d,g} = 1,\; x_z < c\; \text{if}\; d_z^{d,g} = 0\}$, and that each treatment region is the union of such sets over $\treatspace(d,g)$, i.e.,
\begin{equation*}
\scorespace(d,g) = \bigcup_{\treatspace(d,g)}\scorespace(\ddpoint[d,g])    
\end{equation*}

\begin{proof}
Recall that the closure of a set is the union of its interior with its boundary. In addition, the closure of a union of sets is equal to the union of their closures. Therefore, denoting the closure of a set $A$ as $Cl(A)$, we have 
\begin{equation*}
    Cl\big(\scorespace(d,g)\big) = \bigcup_{\treatspace(d,g)}Cl\big(\scorespace(\ddpoint[d,g])\big)    
\end{equation*}
where clearly $Cl\big(\scorespace(\ddpoint[d,g])\big) = \{\ppoint \in \scorespace : \forall z \in (\{i\}\cup \mathcal{S}_i), x_z \geq c \; \text{if}\; d_z^{d,g} = 1,\; x_z \leq c\; \text{if}\; d_z^{d,g} = 0\}$ .

Now by definition $\Frontier = \bar{\mathcal{X}}_{i\smallN_i}(d,g) \cap \bar{\mathcal{X}}_{i\smallN_i}(d',g')$, where $\bar{\mathcal{X}}_{i\smallN_i}(d,g)$ and $\bar{\mathcal{X}}_{i\smallN_i}(d',g')$ denote the boundary of $\scorespace(d,g)$ and $\scorespace(d',g')$. Moreover, because $\scorespace(d,g)$ and $\scorespace(d',g')$ are disjoint, the intersection of their closure is equal to the intersection of their boundaries, $Cl\big(\scorespace(d,g)\big) \cap Cl\big(\scorespace(d',g')\big) = \bar{\mathcal{X}}_{i\smallN_i}(d,g) \cap \bar{\mathcal{X}}_{i\smallN_i}(d',g')$.
Note that $Cl\big(\scorespace(d,g)\big) \cap Cl\big(\scorespace(d',g')\big)$ is equal to 
\begin{equation*}
    \Big(\bigcup_{\treatspace(d,g)} Cl\big(\scorespace(\ddpoint[d,g])\big)\Big) \bigcap\Big( \bigcup_{\treatspace(d',g')} Cl\big(\scorespace(\ddpoint[d',g'])\big)\Big)
\end{equation*}
which in turn is equal to 
\begin{equation*}
    \bigcup_{\treatspace(d,g) \times \treatspace(d',g')} \Big(Cl\big(\scorespace(\ddpoint[d,g])\big)\bigcap Cl\big(\scorespace(\ddpoint[d',g'])\big)\Big)
\end{equation*}
\sloppy
Finally, we note that the intersection $Cl(\scorespace(\ddpoint[d,g])) \cap Cl(\scorespace(\ddpoint[d',g']))$ is equal to the set $ \{\ppoint \in \scorespace : \forall z \in (\{i\}\cup \mathcal{S}_i),\; x_z \geq c \; \text{if}\; d_z^{d,g} = d_z^{d',g'} = 1,\; x_z \leq c\; \text{if}\; d_z^{d,g} = d_z^{d',g'} = 0,\; x_z = c\; \text{if}\; d_z^{d,g} \neq d_z^{d',g'}\}$ which is the definition of $\ell(\ddpoint[d,g], \ddpoint[d',g'])$. 
\end{proof}

\section{Proofs of Main Results in Section \ref{sec:identification}}\label{appendix:boundformal}

Let us formally define the notion of $n-$rectifiable set. Let $\mathcal{H}^n$ denote the $n$-dimensional Hausdorff measure.
\begin{definition}[n-rectifiable set \citep{simon}]
A set $M \subset \mathbb{R}^{n+k}$ is said to be countably $n$-rectifiable if
$$
M \subset M_0 \cup\left(\cup_{j=1}^{\infty} F_j\left(\mathbb{R}^n\right)\right)
$$
where $\mathcal{H}^n\left(M_0\right)=0$ and $F_j: \mathbb{R}^n \rightarrow \mathbb{R}^{n+k}$ are Lipschitz functions for $j=1,2, \ldots $.
\end{definition}
An equivalent characterization is the following:  
a set $M$ is countably $n$-rectifiable if and only if $M \subset \bigcup_{j=0}^{\infty} N_j$, where $\mathcal{H}^n(N_0)=0$ and each $N_j$, $j \ge 1$, is an $n$-dimensional embedded $C^1$ submanifold of $\mathbb{R}^{n+k}$ \citep[Lemma~11.1]{simon}.

As discussed in Section 2.3, the effective treatment boundary $\Frontier$ is the union of finitely many linear pieces in the multiscore space $\scorespace$. Therefore, $\Frontier$ is $(|\mathcal{S}|_i + 1 - \bar{s}_i)-$rectifiable set, with dimension $|\mathcal{S}|_i + 1 - \bar{s}_i$, and codimension $\bar s_i$, where $\bar{s}_i$ is the minimum codimension across the linear pieces.

Thus, we can write the boundary average causal effect as 
\begin{equation}\label{eq:boundformal}
    \boundeff = \frac{\sum\limits_{\ddpoint[d,g],\ddpoint[d',g']}\int\limits_{\ell(\ddpoint[d,g], \ddpoint[d',g'])}\pointeff f\ppoint d\mathcal{H}^{|\mathcal{S}_i| + 1 - \bar{s}_i}}{\sum\limits_{\ddpoint[d,g],\ddpoint[d',g']}\int\limits_{\ell(\ddpoint[d,g], \ddpoint[d',g'])}f\ppoint d\mathcal{H}^{|\mathcal{S}_i| + 1 - \bar{s}_i}}
\end{equation}
where the summation ranges over all pairs $\ddpoint[d,g], \ddpoint[d',g']$ in $\treatspace(d,g)\times\treatspace(d',g')$.

Note that integrals over pieces $\hcurve$ with codimension $s_{\hcurve}$ larger than $\bar{s}_i$ vanish since their $\mathcal{H}^{|\mathcal{S}_i| + 1 - \bar{s}_i}$-dimensional Hausdorff measure is zero. Hence, the expression above is equivalent to summing over only those pieces $\hcurve$ with codimension $\bar{s}_i$.

For each $\hcurve$, define the following index sets:
\begin{itemize}
    \item $F_{\hcurve}$: the set of indices $z \in (\mathcal{S}_i \cup \{i\})$ such that $x_z = c$ on $\hcurve$ (i.e., the constrained components);
    \item $R_{\hcurve}$: the complement set of indices where $x_z$ is free to vary within some interval.
\end{itemize}
The codimension $s_{\hcurve}$ equals the cardinality $|F_{\hcurve}|$.

We henceforth drop the arguments $\bm d _{i\smallN_i}^{d,g}$ and $\bm d _{i\smallN_i}^{d',g'}$ and simply write $\curve$ for each piece. We also use $\sum_{\curve}$ and $\bigcup_{\curve}$ to denote summation and union over the relevant set of pieces $\hcurve$ indexed by $\bm d _{i\smallN_i}^{d,g}$ and $\bm d _{i\smallN_i}^{d',g'}$.

We partition each $\ppoint$ into $\bm{x}_{\cindex}$, where each component is fixed at $c$ on $\curve$, and $\bm{x}_{\findex}$, which ranges over the domain 
\[\mathcal{R}_{\curve} := \prod_{z \in R_{\curve}} I_z(\curve)\]
where $I_z(\curve)  = [a, c]$, if $x_z \le c$ on $\curve$, and $I_z(\curve)  = [c, b]$ if $x_z \geq c$ on $\curve$. 

The structure of each $\curve$ leads to the following simple parametrization of \eqref{eq:boundformal}:
\begin{equation}\label{eq:piecewiseintegral}
 \frac{\sum\limits_{\curve \, : \,\ccard = \bar{s}_i}\bigintsss\limits_{\freeregion}\tau_{d,g|d',g'}(\bm{c}_{\cindex},\bm{x}_{\findex}) f(\bm{c}_{\cindex},\bm{x}_{\findex}) d\bm{x}_{\findex}}
    {\sum\limits_{\curve \, : \, \ccard = \bar{s}_i}\bigintsss\limits_{\freeregion}f(\bm{c}_{\cindex},\bm{x}_{\findex}) d\bm{x}_{\findex}}
\end{equation}
Each integral is taken over the bounded rectangular domain corresponding to the \qq free" components of $\ppoint$ for a given piece $\curve$ of dimension $|\mathcal{S}_i| + 1 - \bar{s}_i$.

% \begin{lemma}\label{lem:stripconv}
% Let $M \subset \mathbb{R}^n$ be a manifold of the form
% \[
% M = \{ x \in \mathbb{R}^n : x_F = c_k,\ x_R \in \mathcal{R} \},
% \]
% where $F$ and $R$ are disjoint index sets with $|F| = k$, $x = (x_F, x_R)$, with $(x_F, x_R)$ a partition of $x$, $c_k$ is a vector of dimension $k$ with components equal to $c$, and $R \subset \mathbb{R}^{n -k}$ is a compact rectangle. Let $f: \mathbb{R}^n \to \mathbb{R}$ be continuous and bounded.

% Define the neighborhood around $M$ of radius $\varepsilon > 0$ as
% \[
% T_\varepsilon := \{ x \in \mathbb{R}^n : \min_{\bar{x} \in M}\|x - \bar{x}\| \leq \varepsilon,\ x_F \in S \},
% \]
% and $S \subset \mathbbm{R}^{k}$ is a product of intervals of the form $[c,b]$ or $[a,c]$. 
% \[
% \lim_{\varepsilon \to 0} \frac{1}{\operatorname{Vol}(T_\varepsilon)} \int_{T_\varepsilon} f(x)\, dx
% = \frac{1}{\operatorname{Vol}(R)} \int_{x_R \in R} f(c_F, x_R)\, dx_R.
% \]
% \end{lemma}

\begin{proof}[Proof of Theorem \ref{th:cont}]
We start by proving convergence of 
$$\CE{Y_i(d,g)}{(X_i,\pscore) \in \eballboundright}$$
Define the conditional mean function
$$m_{d,g}\ppoint = \CE{Y_i(d,g)}{(X_i, \pscore) = \ppoint}$$ 
The expectation $\CE{Y_i(d,g)}{(X_i,\pscore) \in \Frontier}$ can be written as 
\begin{equation}
    \frac{\sum\limits_{\curve \, : \,\ccard = \bar{s}_i}\int\limits_{\freeregion}m_{d,g}(\bm{c}_{\cindex},\bm{x}_{\findex})f(\bm{c}_{\cindex},\bm{x}_{\findex})d\bm{x}_{\findex}}
    {\sum\limits_{\curve \, : \, \ccard = \bar{s}_i}\bigintsss\limits_{\freeregion}f(\bm{c}_{\cindex},\bm{x}_{\findex})d\bm{x}_{\findex}}
\end{equation}
For a piece $\curve$ with constrained components $\cindex$ fixed at $\bm{c}_{\cindex}$ and free components $\findex$, denote by $\curveball$ the $\varepsilon$-neighborhood around $\curve$, restricted to the region
$$\scorespace(\bm d_{i\smallN_i}^{d,g}) = \big\{\ppoint \in \scorespace : \forall z \in (\{i\}\cup \mathcal{S}_i),\; x_z \geq c \; \text{if}\; d_z^{d,g} = 1,\; x_z < c\; \text{if}\; d_z^{d,g} = 0\big\}$$ 
Equivalently, 
$$
\curveball = \big\{ \ppoint \in \scorespace : \bm{x}_{\cindex} \in \disc, \; \bm{x}_{\findex} \in \freeregion \big\},
$$
where
$$
\disc := \Big\{ \bm{x}_{\cindex} : \|\bm{x}_{\cindex} - \bm{c}_{\cindex}\| \leq \varepsilon, \; x_z \geq c \text{ if } d_z^{d,g} = 1, \; x_z < c \text{ if } d_z^{d,g} = 0 \Big\}.
$$
Geometrically, $\disc$ is the intersection of a $\ccard$-dimensional ball of radius $\varepsilon$ centered at $\bm{c}_{\cindex}$ with the orthant determined by the threshold $c$ for each constrained coordinate. Hence its volume depends on $\curve$ only through the codimension $\ccard$. Denote
$$\operatorname{Vol}(\disc) = \ballvolume,
\qquad 
\ballvolume = \kappa_{\ccard} \, \varepsilon^{\ccard},$$
where $\kappa_{\ccard}>0$ is a constant depending only on the orthant fraction of the $\ccard$-dimensional ball. 

Since the neighborhood $\eballboundright$ is the union of $\curveball$, we can write $\CE{Y_i(d,g)}{(X_i,\pscore) \in \eballboundright}$ as   
\begin{equation}\label{eq:fibers}
    \frac{\sum\limits_{\curve }\int\limits_{\freeregion}\int\limits_{\disc}\hspace{-1em}m_{d,g}\partition f\partition d\bm{x}_{\cindex}d\bm{x}_{\findex} + I_\varepsilon}
{\sum\limits_{\curve }\int\limits_{\freeregion}\int\limits_{\disc}\hspace{-1em} f\partition d\bm{x}_{\cindex}d\bm{x}_{\findex} + I'_\varepsilon} 
\end{equation}
and the terms $I_\varepsilon$ and $I_{\varepsilon}'$ include the integrals over the intersections of the neighborhoods $\curveball$.

We first establish the limit of the average integral
\begin{equation}\label{eq:avgint}
\frac{1}{\ballvolume}\int_{\disc} f(\bm{x}_{\cindex}, \bm{x}_{\findex}) \, d\bm{x}_{\cindex},
\end{equation}
for fixed $\bm{x}_{\findex}$.

By Assumption~\ref{ass:densitycont}, the density $f$ is continuous. Hence, given $\bm{x}_{\findex}$ and any $\delta > 0$, there exists $r > 0$ such that whenever $\|\bm{x}_{\cindex} - \bm{c}_{\cindex}\| \leq r$,  
\[
\big| f(\bm{x}_{\cindex}, \bm{x}_{\findex}) - f(\bm{c}_{\cindex}, \bm{x}_{\findex}) \big| < \delta. 
\]
Therefore, for $\varepsilon < r$, 
\begin{equation*}
\begin{split}
\frac{1}{\ballvolume}\Bigg|\int_{\disc} 
   \big(f(\bm{x}_{\cindex}, \bm{x}_{\findex}) - f(\bm{c}_{\cindex}, \bm{x}_{\findex})\big)\, d\bm{x}_{\cindex}\Bigg| 
\leq \,& \frac{1}{\ballvolume}\int_{\disc} 
   \big| f(\bm{x}_{\cindex}, \bm{x}_{\findex}) - f(\bm{c}_{\cindex}, \bm{x}_{\findex}) \big|\, d\bm{x}_{\cindex} \\
< \, & \delta.
\end{split}
\end{equation*}
Thus, \eqref{eq:avgint} converges to $f(\bm{c}_{\cindex}, \bm{x}_{\findex})$ as $\varepsilon \to 0$. Moreover,
\begin{equation*}
\begin{split}
\lim_{\varepsilon \to 0} \frac{1}{\ballvolume}
   \int\limits_{\freeregion} \int\limits_{\disc}
   \kern-1em f(\bm{x}_{\cindex}, \bm{x}_{\findex}) \, d\bm{x}_{\cindex}\, d\bm{x}_{\findex}
&= \frac{1}{\ballvolume} \int\limits_{\freeregion} 
   \lim_{\varepsilon \to 0}\int\limits_{\disc}
   \kern-1em f(\bm{x}_{\cindex}, \bm{x}_{\findex}) \, d\bm{x}_{\cindex}\, d\bm{x}_{\findex} \\
&= \int\limits_{\freeregion} f(\bm{c}_{\cindex}, \bm{x}_{\findex})\, d\bm{x}_{\findex},
\end{split}
\end{equation*}
by the Dominated Convergence Theorem, since the score density is bounded by Assumption~\ref{ass:bounded}.

By the same argument, we also obtain convergence of
$$
\frac{1}{\ballvolume}
   \int\limits_{\freeregion}\int\limits_{\disc}
   m_{d,g}(\bm{x}_{\cindex}, \bm{x}_{\findex}) f(\bm{x}_{\cindex}, \bm{x}_{\findex}) \,
   d\bm{x}_{\cindex}\, d\bm{x}_{\findex}
$$
to
$$
\int_{\freeregion} m_{d,g}(\bm{c}_{\cindex}, \bm{x}_{\findex}) \,
   f(\bm{c}_{\cindex}, \bm{x}_{\findex})\, d\bm{x}_{\findex}.
$$
because $m_{d,g}$ and $f$ are continuous and bounded by Assumptions \ref{ass:cont}-\ref{ass:densitycont} and \ref{ass:bounded}.

Hence, each element of the numerator and denominator in \eqref{eq:fibers} is of order 
$O(\varepsilon^{\ccard})$, which implies that both summations are 
$O(\varepsilon^{\bar{s}_i})$. Moreover, since both the score density and the conditional mean of potential outcomes are bounded by Assumption \ref{ass:bounded}, and the region of integration of $I_\varepsilon$ and $I_\varepsilon'$ has volume $O(\varepsilon^{\bar{s}_i+1})$, we obtain 
$|I_\varepsilon| \lesssim \varepsilon^{\bar{s}_i+1}$ and 
$|I_\varepsilon'| \lesssim \varepsilon^{\bar{s}_i+1}$.
\footnote{To see this, note that each tubular neighborhood $\curveball$ is contained in a rectangular box 
$\cube = \{\ppoint \in \scorespace : \bm{x}_{\findex} \in \freeregion, \; |x_z - c|\leq \varepsilon \text{ for all } z \in \cindex\}$, with volume $O(\varepsilon^{\ccard})$. 
The intersection of tubes $\{\curveball : \curve \in \tilde{C}\}$ for any collection $\tilde{C}$ of pieces is then contained in the intersection of the corresponding boxes $\{\cube : \curve \in \tilde{C}\}$. 
This set is described as follows: $x_z \in [a,c]$ if $z \in \cap_{\tilde{C}}\negindex$, 
$x_z \in [c,b]$ if $z \in \cap_{\tilde{C}}\posindex$, where $\negindex$ and $\posindex$ are index sets collecting the indices of the components varying in $[a,c]$ and $[c,b]$, respectively, in each $\curve$, and $|x_z - c|\leq \varepsilon$ if $z \in \cap_{\tilde{C}}\cindex$ or if $z$ does not lie in all positive or all negative index sets. Hence, the intersection set is rectangular with volume $O(\varepsilon^{\bar{s}_i+1})$.}

By dividing numerator and denominator of \eqref{eq:fibers} by 
\(V_{\varepsilon}^{\bar{s}_i} = \kappa_{\bar{s}_i}\varepsilon^{\bar{s}_i}\), 
we obtain
\begin{equation*}
\begin{split}
\eqref{eq:fibers} &\to 
\frac{\sum\limits_{\curve}
\int_{\freeregion} m_{d,g}(\bm{c}_{\cindex},\bm{x}_{\findex}) 
f(\bm{c}_{\cindex},\bm{x}_{\findex}) \, d\bm{x}_{\findex}}
{\sum\limits_{\curve}
\int_{\freeregion} f(\bm{c}_{\cindex},\bm{x}_{\findex}) \, d\bm{x}_{\findex}},
\end{split}
\end{equation*}
where only terms with $\ccard = \bar{s}_i$ contribute in the limit, since $\varepsilon^{s_{\ccard}-\bar{s}_i}\to 0$ for $s_{\ccard} > \bar{s}_i$. Hence,
\begin{equation*}
\eqref{eq:fibers} \to
\CE{Y_i(d,g)}{(X_i, \pscore) \in \Frontier},
\end{equation*}
by the Dominated Convergence Theorem and Assumptions 
\ref{ass:cont}--\ref{ass:densitycont}, \ref{ass:bounded}.
Analogously, one can show
$\CE{Y_i(d',g')}{(X_i, \pscore) \in \eballboundleft}$ 
converges to 
$\CE{Y_i(d',g')}{(X_i, \pscore) \in \Frontier}$.

Therefore,
\begin{equation*}
\begin{split}
\boundeff 
&= \CE{Y_i(d,g) - Y_i(d',g')}{(X_i,\pscore) \in \Frontier} \\
&= \lim_{\varepsilon \to 0}\CE{Y_i(d,g)}{(X_i,\pscore) \in \eballboundright} \\
& -\; \lim_{\varepsilon \to 0}\CE{Y_i(d',g')}{(X_i,\pscore) \in \eballboundleft} \\
&= \lim_{\varepsilon \to 0}\CE{Y_i}{(X_i,\pscore) \in \eballboundright} \\
&-\; \lim_{\varepsilon \to 0}\CE{Y_i}{(X_i,\pscore) \in \eballboundleft},
\end{split}
\end{equation*}
where the last equality follows from Assumptions \ref{ass:consistency}-\ref{ass:interfence} and 
Property \ref{pr:unconf}.
\end{proof}

\begin{proof}[Proof of Theorem \ref{th:overall}]
Let us define $\mathcal{X}_{\smallN_i} \subseteq \mathbbm{R}^{|\smallN_i|}$ as the set of elements $ \bm{x}_{\smallN_i}$. Further, for all $g \in \mathcal{G}_i$ define $ \mathcal{X}_{\smallN_i}(g) = \{\bm{x}_{\smallN_i} \in \mathcal{X}_{\smallN_i} : e(\bm{x}_{\smallN_i}) = g\}$. 

Note that $\bar{\mathcal{X}}_{i\smallN_i}(1,g\,|\,0,g) = 
 \{(x_i, \bm{x}_{\smallN_i}) \in \scorespace : x_i = c,\, \bm{x}_{\smallN_i}\in \mathcal{X}_{\smallN_i}(g)\}$ for all $g \in \mathcal{G}_i$. By Assumption \ref{ass:densitycont} we have that $\lim_{x_i \to c} f(x_i,\bm{x}_{\smallN_i}) =  f(c,\bm{x}_{\smallN_i})$. Moreover, $$ \lim_{x_i \to c} \int\limits_{\mathcal{X}_{\smallN_i}} f(x_i,\bm{x}_{\smallN_i})d\bm{x}_{\smallN_i} = \int\limits_{\mathcal{X}_{\smallN_i}} f(c,\bm{x}_{\smallN_i})d\bm{x}_{\smallN_i}$$ by the Dominated Convergence Theorem following from Assumption \ref{ass:densitycont} and \ref{ass:bounded}. Therefore, because $f(x_i) = \int_{\mathcal{X}_{\smallN_i}}f(x_i,\bm{x}_{\smallN_i})d\bm{x}_{\smallN_i} $ it follows that  $\lim_{x_i \to c}f(x_i) = f(c)$.

We have 
\begin{equation*}\label{eq:bo}
\begin{split}
    \lim_{x_i \downarrow c}\CE{Y_i}{X_i = x_i} &=  \lim_{x_i \downarrow c}\sum_{g \in \mathcal{G}_i} \int_{\mathcal{X}_{\smallN_i}(g)}\CE{Y_i}{X_i = x_i, \pscore = \bm{x}_{\smallN_i}}\cdot\frac{f(x_i, \bm{x}_{\smallN_i})}{f(x_i)}d\bm{x}_{\smallN_i}\\
    & = \lim_{x_i \downarrow c}\sum_{g \in \mathcal{G}_i} \int_{\mathcal{X}_{\smallN_i}(g)}\CE{Y_i(1,g)}{X_i = x_i, \pscore = \bm{x}_{\smallN_i}}\cdot\frac{f(x_i, \bm{x}_{\smallN_i})}{f(x_i)}d\bm{x}_{\smallN_i} \\
    & = \sum_{g \in \mathcal{G}_i} \int_{\mathcal{X}_{\smallN_i}(g)}\CE{Y_i(1,g)}{X_i = c, \pscore = \bm{x}_{\smallN_i}}\cdot\frac{f(c, \bm{x}_{\smallN_i})}{f(c)}d\bm{x}_{\smallN_i} \\
     %&= \sum_{g \in \mathcal{G}_i} \int_{\mathcal{X}_{\smallN_i}(g)}\CE{Y_i(1,g)}{X_i = x_i, \pscore = \bm{x}_{\smallN_i}}\cdot\frac{f(\bm{x}_{\smallN_i})f(x_i|\bm{x}_{\smallN_i})}{f(x_i)}d\bm{x}_{\smallN_i}
    \end{split}
\end{equation*}
where the first equality come from the Law of Iterated expectations, the second equality from Assumptions \ref{ass:consistency}-\ref{ass:interfence}, and the third equality follows from the Dominated Convergence Theorem, since $\frac{f(x_i, \bm{x}_{\smallN_i})}{f(x_i)}$ is continuous, and $\CE{Y_i(1,g)}{X_i = x_i, \pscore = \bm{x}_{\smallN_i}}$ is continuous and bounded by Assumption \ref{ass:cont}  and \ref{ass:bounded}.

Note that $\CPrr{\pscore\in \mathcal{X}_{\smallN_i}(g)}{X_i = c} = \CPrr{G_i = g}{X_i = c} =  \bigintsss\limits_{\mathcal{X}_{\smallN_i}(g)}\frac{f(c, \bm{x}_{\smallN_i})}{f(c)}d\bm{x}_{\smallN_i}$, and
\begin{equation*}
\int\limits_{\mathcal{X}_{\smallN_i}(g)}\CE{Y_i(1,g)}{X_i = c, \pscore = \bm{x}_{\smallN_i}}\cdot\frac{f(c, \bm{x}_{\smallN_i})}{\int\limits_{\mathcal{X}_{\smallN_i}(g)}f(c, \bm{x}_{\smallN_i})}d\bm{x}_{\smallN_i} = \CE{Y_i(1,g)}{(X_i, \bm{x}_{\smallN_i}) \in  \bar{\mathcal{X}}_{i\smallN_i}(1,g,|0,g)}
\end{equation*} 
Hence, by multiplying and dividing each element of the summation in the last line of \eqref{eq:bo} by $\int\limits_{\mathcal{X}_{\smallN_i}(g)}f(c, \bm{x}_{\smallN_i})d\bm{x}_{\smallN_i}$, we obtain
\begin{equation*}
  \lim_{x_i\downarrow c}\CE{Y_i}{X_i = x_i} =   \CE{Y_i(1,g)}{(X_i, \bm{x}_{\smallN_i}) \in  \bar{\mathcal{X}}_{i\smallN_i}(1,g,|0,g)}\cdot \CPrr{G_i = g}{X_i = c}
\end{equation*}
 By analogous arguments 
\begin{equation*}
    \begin{split}
    \lim_{x_i\uparrow c}\CE{Y_i}{X_i = x_i} & = \sum_{g \in \mathcal{G}_i}\CE{Y_i(0,g)}{(X_i, \bm{x}_{\smallN_i}) \in  \bar{\mathcal{X}}_{i\smallN_i}(1,g,|0,g)}\cdot \CPrr{G_i = g}{X_i = c} \\
\end{split}
\end{equation*}
from which the conclusion follows.
\end{proof}

\section{Proofs of Main Results in Section \ref{sec:estimation}}\label{appendix:estimator}

This section provides the asymptotic theory for $\estimator$. Recall the expression for the observed outcome  
\begin{equation*}
    Y_i = \mu(\distvar) + \error, \quad i= 1,...,n
\end{equation*}
with $\mu(\distvar) = \CE{Y_i}{\distvar, D_i, G_i}$, $\error = m(X_i, \pscore) - \mu(\distvar) + \epsilon_i$, where $m(X_i, \pscore) =\sum_{d,g}\mathbbm{1}((X_i, \pscore) \in \scorespace(d,g))\cdot m_{d,g}(X_i, \pscore)$, and $\epsilon_i = \sum_{d,g}\mathbbm{1}((X_i, \pscore) \in \scorespace(d,g))\cdot \epsilon_{i,d,g}$.
We denote $\distvar$, and $\error$ by $\distvari$ and $\errori$ for convenience. 

The outcome regression functions of interest are
\begin{equation*}
    \muplus = \CE{Y_i}{\distvari = \tilde{x}_i, D_i = d, G_i = g}, \quad
    \muminus  = \CE{Y_i}{\distvari = \tilde{x}_i, D_i = d', G_i = g'}
\end{equation*} 
In what follows, results are stated for $\estimatorapp$, the distance-based $p-$order local polynomial estimator for $\boundeff$. Here, we assume that all units have equally-sized interference sets $|\mathcal{S}_i|$ and common codimension $\bar{s}$.
The data are identically, although non independently, distributed, so that $\CE{Y_i(d,g)}{(X_i, \pscore) = \ppoint}$ and $f\ppoint$, and thus the boundary average causal effects, are homogeneous for all $i$. The case with heterogeneous interference sets and data distributions is treated in Section \ref{appendix:heterogeneous}.

\subsection{Notation}\label{subsec:notation}

\noindent Let $p,q \in \mathbb{Z}_{+}$. Define $\rp[u] = [1 , u, u^2, ...,u^p]$ and let $K_h^{\bar s}(u) = K(u/h)/h^{\bar s}$, where $K(\cdot)$ is a kernel function. The estimator $\estimatorapp$ is given by : 
\begin{align*}
    & \estimatorapp = e_1^T\betaplus\: - e_1^T\betaminus\\
    & \betaplus = \argmin\limits_{\bm{b} \in \mathbbm{R}^{p+1}}\sum_i\mathbbm{1}(D_i = d, G_i = g)(Y_i - \rp[\tilde{X}_{i}]^T\bm{b})^2\cdot K_{h_n^{\bar s}}(\tilde{X}_{i}) \\
    &\betaminus = \argmin\limits_{\bm{b}\in \mathbbm{R}^{p+1}}\sum_i\mathbbm{1}(D_i = d', G_i = g')(Y_i - \rp[\tilde{X}_{i}]^T\bm{b})^2\cdot K_{h_n^{\bar s}}(\tilde{X}_{i})
\end{align*}
where $h_n$ is a positive bandwidth and $e_1$ is the $(p+1)$-dimensional vector with the first entry equal to 1 and 0 elsewhere. We set $\Iplus = \mathbbm{1}(D_i = d, G_i = g)$ and $\Iminus = \mathbbm{1}(D_i = d', G_i = g')$, and $\bm{Y} = [Y_1,..., Y_n]^T$. In addition, we define 
\begin{align*}
        & \tilde{X}_p(h) = [\rp[\tilde{X}_1/h],..., \rp[\tilde{X}_n/h]]^T, \\
        %& S_p(h) = [(\tilde{X}_1/h)^p,...,(\tilde{X}_n/h)^p]^T, \\
        & W_{d,g}(h)= \text{diag}(\Iplus[1]\cdot K_{h^{\bar s}}(\distvari[1]),...,\Iplus[n] \cdot K_{h^{\bar s}}(\distvari[n])),\\
        &W_{d',g'}(h)= \text{diag}(\Iminus[1]\cdot K_{h^{\bar s}}(\distvari[1]),..., \Iminus[n] \cdot K_{h^{\bar s}}(\distvari[n])).
\end{align*}
and the following sample quantities: 
\[
\begin{aligned}
  \begin{aligned}[t]
  &\Gamma_{d,g,p}(h) = \tilde{X}_p(h)^T W_{d,g}(h)\tilde{X}_p(h)/n,\\
  &t_{d,g,p}(h) = \tilde{X}_p(h)^T W_{d,g}(h)\bm{Y}/n,\\
  &\theta_{d,g,p,q}(h) = \tilde{X}_p(h_n)^T W_{d,g}(h_n) S_q(h_n)/n,
  \end{aligned}
  \qquad
  \begin{aligned}[t]
  &\Gamma_{d',g',p}(h) = \tilde{X}_p(h)^T W_{d',g'}(h)\tilde{X}_p(h)/n,\\
  &t_{d',g',p}(h) = \tilde{X}_p(h)^T W_{d',g'}(h)\bm{Y}/n,\\
  &\theta_{d',g',p,q}(h_n) = \tilde{X}_p(h)^T W_{d',g'}(h_n) S_q(h_n)/n,
  \end{aligned}
\end{aligned}
\]
with $S_q(h) = [(\distvari[1]/h)^q,...,(\distvari[n]/h)^q]$.
Denote by $\Gammaplusbc{,p}{h}{}$, $\Gammaminusbc{,p}{h}{}$, $\bar{t}_{d,g,p}(h)$, $\bar t_{d',g',p}(h)$, $\bar{\theta}_{d,g,p,q}(h_n)$, $\bar{\theta}_{d',g',p,q}(h_n)$ their respective expectations. Let $H(h_n) = \text{diag}(1, h^{-1}, ..., h^{-p})$. Then:
\begin{align*}
&\betaplus = H(h_n)\Gammaplus[-1]\tplus, \quad 
\betaminus = H(h_n)\Gammaminus[-1]\tminus
\end{align*}
Next, we define the population linear projection coefficients:
\begin{equation}\label{eq:linearprojection}
\begin{split}
\beta_{d,g,p}(h_n) =& H(h_n)\Gammaplusbc{,p}{h_n}{-1}\bar{t}_{d,g,p}(h_n), \quad
\beta_{d',g',p}(h_n) = H(h_n)\Gammaminusbc{,p}{h_n}{-1}\bar{t}_{d',g',p}(h_n)
\end{split}
\end{equation}
where 
\begin{align*}
\beta_{d,g,p}(h_n) =& \argmin\limits_{\bm{b} \in \mathbbm{R}^{p+1}}\E\Big[\sum_i\mathbbm{1}(D_i = d, G_i = g)(Y_i - \rp[\distvari]^T\bm{b})^2\cdot K_{h_n^{\bar{s}}}(\distvari)\Big] \\
\beta_{d',g',p}(h_n) =& \argmin\limits_{\bm{b} \in \mathbbm{R}^{p+1}}\E\Big[\sum_i\mathbbm{1}(D_i = d', G_i = g')(Y_i - \rp[\distvari]^T\bm{b})^2\cdot K_{h_n^{\bar{s}}}(\distvari)\Big]
\end{align*}
and introduce the following centered quantities:
\begin{equation}\label{eq:centerest}
\begin{aligned}
\begin{aligned}[t]
        &\tplus[*] = \Xp^T \Wplus \bm {\nu}_{d,g} /n, \\    &\betaplus[*] = H(h_n)\Gammaplus[-1] \tplus[*], \\
        &t^*_{d,g,d',g',p}(h_n) =  \tplus[*] - \tminus[*], \\
        &\hat{\tau}^{*}_{d,g,d',g',p}(h_n) = e_1^T\betaplus[*] - e_1^T\betaminus[*].
    \end{aligned}
    \quad
    \begin{aligned}[t]
        &\tminus[*] = \Xp^T \Wminus \bm \nu_{d',g'}/n \\
        &\betaminus[*] = H(h_n)\Gammaminus[-1] \tminus[*] \\
    \end{aligned}
\end{aligned}
\end{equation}
with $\bm\nu_{d,g} = [\nu_{1,d,g}, ..., \nu_{n,d,g}]$ and $\bm\nu_{d',g'} = [\nu_{1,d',g'}, ..., \nu_{n,d',g'}]$ where for each $i$: 
\begin{equation*}
    \nu_{i,\bullet} = Y_i - \rp[\distvari]^T\beta_{\bullet,p}(h_n), \quad \bullet \in \{(d,g), (d',g')\}
\end{equation*}
We denote the scaled variance and covariance of $\tplus[*]$ and $\tminus[*]$ by
\[
\begin{aligned}
\Psiplusbc{p}{}{h_n} &= n h_n^{\bar{s}} \V[\tplus[*]], \quad
\Psiminusbc{p}{}{h_n} = n h_n^{\bar{s}} \V[\tminus[*]], \\[-2pt]
\Psiplusminusbc{p}{}{h_n} &= n h_n^{\bar{s}} \C[\tplus[*], \tminus[*]]
\end{aligned}
\]
We further define the kernel-weighted subgraph for units with $(D_i = d, G_i = g)$, $\bm{W}^{d,g}(h_n)$ with entry $W^{d,g}_{ij}(h_n) = W_{ij}\Iplus\Iplus[j]\Kh\Kh[j]$. Let $\bar{\bm{D}}^{d,g}(h_n)$ denote the expected sum of its diagonal elements and let $\bar{\bm{N}}^{d,g}(h_n)$ be its expected average degree without the diagonal terms. Similarly, define $\bm{W}^{d',g'}(h_n)$, $\bar{\bm{D}}^{d',g'}(h_n)$ and $\bar{\bm{N}}^{d',g'}(h_n)$.  Finally, let  $\bm{W}^{d,g,d',g'}(h_n)$ with entry 
$W^{d,g,d',g'}_{ij}(h_n) = W_{ij}\Iplus\Iminus[j]\Kh\Kh[j]$, and expected degree $\bar{\bm{N}}^{d,g,d',g'}(h_n)$.

Lastly, let $\unitdisc$ be the intersection of the $s$-dimensional unit ball centered at zero $\bm{0}_s$ with a generic orthant in $\mathbbm{R}^{s}$ and let: 
\begin{align*}
    &\Gamma_p^s = \int_{\unitdisc}K(||\bm{u}_s||)\rp[||\bm{u}_s||]\rp[||\bm{u}_s||]^Td\bm{u}_s \\
    &\theta_{p,q}^s =  \int_{\unitdisc}K(||\bm{u}_s||)(||\bm{u}_s||)^q\rp[||\bm{u}_s||]d\bm{u}_s \\
    &\Psi_p^s =  \int_{\unitdisc}K(||\bm{u}_s||)^2\rp[||\bm{u}_s||]\rp[||\bm{u}_s||]^Td\bm{u}_s
\end{align*}
For short, we will denote by $\limdensity = \int_{\Frontier}f\ppoint d\mathcal{H}^{|\mathcal{S}_i| + 1 - \bar{s}}$. 

\noindent\textbf{Note.} In the main text, we report our results for $p = 1$ and therefore drop the subscript $p$ indexing the polynomial order to simplify notation 
(e.g., we write $\Gamma^{s}$ instead of $\Gamma^{s}_{p}$ and $\hat{\beta}_{d,g}(h_n)$ instead of $\hat{\beta}_{d,g,p}(h_n)$). 
In this appendix, we retain the full notation with $p$.

%as well as
% \begin{equation*}
%     \sigmaplus[0] = \int\limits_{\Frontier}\sigmaplus[x_i, \bm x_{\mathcal{S}_i}] f\ppoint d\ppoint, \quad \sigmaminus[0] = \int\limits_{\Frontier}\sigmaminus[x_i, \bm x_{\mathcal{S}_i}] f\ppoint d\ppoint
% \end{equation*}

\subsection{Assumptions}

In addition to Assumptions \ref{ass:consistency}-\ref{ass:identification}, we make the following assumptions. 

% Regularity assumptions: densities and variance  
\begin{assumption}\label{ass:regularity}
For some positive $\kappa$ the following
holds for $\ppoint \in \eballbound[\kappa]$ for all $i$:

\begin{enumerate}[label= \alph*), ref={\theassumption.\alph*}]
    \item $\CE{Y_i^4}{ X_i = x_i, \pscore = \bm{x}_{\smallN_i}}$ is bounded.\label{ass:fourthmoment}
    %\item $f\ppoint$ is bounded away from zero and continuous.\label{ass:densities}
    \item $\sigmapluseps = \V[Y_i(d,g) | X_i = x_i, \pscore = \bm{x}_{\smallN_i}]$ and $\sigmaminuseps=\V[Y_i(d',g') |  X_i = x_i, \pscore = \bm{x}_{\smallN_i}]$ are bounded away from zero and continuous. \label{ass:variances}.
    \item 
    %$m_{d,g}\ppoint$ and $m_{d'g'}\ppoint$ are homogeneous across $i$ and continuous, and  
    $\muplus$ and $\muminus$ are $S$-times continuously differentiable with $S\geq p+2$. 
    \label{ass:smoothness}% Smoothness of distance-based outcome regression function 
\end{enumerate}
\end{assumption}

% No common distance variable assumption
\begin{assumption}\label{ass:commonpieces}
For all $i$, $j \in \bm{N}_{i}$ , $|\cindex\cup F_{\curve[j]}|> \min\{\bar s_i, \bar{s}_j\} = \bar s$ for any piece $\curve$, $\curve[j]$, where $\bar s_i$ and $\bar s_j$ are the codimension of $\Frontier$ and $\bar{\mathcal{X}}_{j\smallN_j}(d,g|d',g')$.
\end{assumption}

\begin{assumption}\label{ass:kernel}
The kernel function $K:\mathbbm{R} \to \mathbbm{R}$ has support $\text{supp}(K) = [-1,1]$, is bounded and non-negative on $[-1,1]$, and is positive, symmetric and continuous on $(-1,1)$. 
\end{assumption}

\subsection{Asymptotic Theory}\label{subsec:asytheory}

In this section we establish the asymptotic distribution of our estimator.  
Recall that the boundary $\Frontier$ is the union of pieces $\curve$ (Section~\ref{sec:framework}, Appendix~\ref{appendix:mainresults}), and that each neighborhood $\eballboundright$ decomposes into tubular neighborhoods $\curveball$, with
\[
\operatorname{Vol}(\curveball)=O(\varepsilon^{\ccard}), 
\qquad 
\operatorname{Vol}(\eballboundright)=O(\varepsilon^{\bar s_i}),
\]
and analogously for $\eballboundleft$ (see proof of Theorem~\ref{th:cont}).

%Following \citet{masry}, we study the centered estimator $\estimatorapp[*]$.  
We decompose $\betaplus$ as follows:
\begin{equation}\label{eq:expansionbeta}
    \begin{split}
        \betaplus = & \beta_{d,g,p}(h_n) + H(h_n)\Gammaplus[-1]\Xp\Wplus\bm \nu_{d,g} \\
        = &  \beta_{d,g,p}(h_n) + \betaplus[*]
    \end{split}
\end{equation}
%
% For generic integer $q$ and $\bullet \in \{(d,g), (d',g')\}$ define
% \[
% \bar{\theta}_{\bullet,p,q}(h_n) = \E\big[\tilde{X}_p(h_n)^TW_{\bullet}(h_n)\,S_q(h)/n\big], \quad S_q(h_n) = [(\distvari[1]/h_n)^q,...,(\distvari[n]/h_n)^q] 
% \]
%
Under Assumption \ref{ass:smoothness} a $(p+1)$-order Taylor expansion of $\muplus[\distvari]$ to the right of the cutoff yields
\begin{equation*}
\begin{split}
    \beta_{d,g,p}(h_n) = & \betaestimandplus + h_n^{p+1}\frac{\mu_{d,g}^{(p+1)}(0)}{(p+1)!}H(h_n)\Gammaplusbc{,p}{h_n}{-1}\thetaplusbc{p}{p+1}{h_n} + T_{d,g}(h_n)    
\end{split}
\end{equation*}
where $\betaestimandplus = [\mu_{d,g}(0), \;\mu^{(1)}_{d,g}(0),\,...,\, \mu_{d,g}^{(p)}(0)/p!]^T$ and 
\[
T_{d,g}(h_n) = H(h_n)\Gammaplusbc{,p}{h_n}{-1}\E\big[\Xp\Wplus T_{d,g,p}/n\big], \quad T_{d,g,p}=[T_{d,g,1},\dots,T_{d,g,n}]
\]
with each Taylor reminder component satisfying $|T_{d,g,i}|\leq \sup_{\tilde x}|\mu_{d,g}^{(p+2)}(\tilde x)|\cdot|\tilde X_i^{p+2}|/(p+2)!$. An analogous expansion holds for $\beta_{d',g',p}(h_n)$. Combining the two, we obtain
\begin{equation}\label{eq:decompositiontau}
    \begin{split}
        \estimatorapp = & \boundeff + h_n^{p+1}\bias + T_{d,g,d'g'}(h_n)\\
        + & \estimatorapp[*]
    \end{split}
\end{equation}
where $\bias = \frac{\muplusderiv[(p+1)]}{(p+1)!}\biasplus - \frac{\muminusderiv[(p+1)]}{(p+1)!}\biasminus$, with
\[
\biasplus= e_1^T\Gammaplusbc{,p}{h_n}{-1}\thetaplusbc{p}{p+1}{h_n}, \quad \biasminus=e_1^T\Gammaminusbc{,p}{h_n}{-1}\thetaminusbc{p}{p+1}{h_n},
\]
and $T_{d,g,d'g'}(h_n) = e_1^T\big(T_{d,g}(h_n) - T_{d',g'}(h_n)\big)$. 

\medskip
\noindent The proof proceeds as follows.
For effective treatment $\bullet \in \{(d,g), (d',g')\}$ Lemma~\ref{lemma:convergencematricesgamma} establishes convergence in probability of $\Gamma_{\bullet,p}(h_n)$ to $\bar{\Gamma}_{\bullet,p}(h_n)$, and shows that $\bar{\Gamma}_{\bullet,p}(h_n)$ has deterministic limit $ \limdensity \Gamma_p^{\bar s}$ as $h_n \to 0$. Lemma~\ref{lemma:convergencematricest} establishes convergence in probability of $t_{\bullet,p}(h_n)$ to $\bar{t}_{\bullet,p}(h_n)$, and that $\bar{t}_{\bullet,p}(h_n) \to \theta_{p,0}^{\bar{s}} \int_{\Frontier} m_{\bullet}\ppoint f\ppoint$. Lemma~\ref{lemma:convergencematricestheta} that $\theta_{\bullet,p,q}(h_n)$ converges in probability to $\bar{\theta}_{\bullet,p,q}(h_n)$, and that $\bar{\theta}_{\bullet,p,q}(h_n)$ converges to $\limdensity \theta^{\bar{s}}_{p,p+1}$.
Combining Lemmas~\ref{lemma:convergencematricesgamma} and~\ref{lemma:convergencematricestheta} implies that the bias term $\bias \to (\Gamma_p^{\bar{s}})^{-1}\theta^{\bar{s}}_{p,q}$ as $h_n \to 0$. Lemma~\ref{lemma:subgraph} shows that the kernel-weighted dependency subgraphs has vanishing average degree, and Lemma~\ref{lemma:variances} derives the limiting variance of $t^*_{d,g,d',g',p}(h_n)$. Finally, Theorem~\ref{th:asynormaltau} establishes the asymptotic normality of the rescaled and recentered estimator $\estimatorapp$ using Stein’s method and the dependency graph bounds of \citet[Theorem A.4]{leung20}.

%=========================================================
% Lemma: convergence of sample matrices%=========================================================

\begin{lemma}[Convergence of $\Gammaplus$ and $\Gammaminus$]\label{lemma:convergencematricesgamma}

Suppose Assumptions \ref{ass:consistency}--\ref{ass:indrule}, \ref{ass:pos}, \ref{ass:densitycont}, \ref{ass:dependencyneighborhood}--\ref{ass:localdependence} and \ref{ass:kernel} hold. 
If $n h_n^{\bar{s}} \to \infty$ and $h_n < \kappa$
then
\[
\Gammaplus = \Gammaplusbc{,p}{h_n}{} + o_p(1), \quad  \Gammaminus = \Gammaminusbc{,p}{h_n}{} + o_p(1)
\]. 
where $\Gammaplusbc{,p}{h_n}{}$ and $\Gammaminusbc{,p}{h_n}{}$ are bounded and bounded away from zero.

Moreover, if $h_n \to 0$ 
    \[
    \Gammaplusbc{}{h_n}{}  = \limdensity \Gamma_p^{\bar{s}} + o(1),
    \qquad 
    \Gammaminusbc{}{h_n}{} = \limdensity \Gamma_p^{\bar{s}} + o(1).
    \]
\end{lemma}

\begin{proof}

\noindent\textbf{Expectation of $\Gammaplus$}. The generic element of $\Gammaplus$ is 
\[
F_{d,g,k}(h_n) = \frac{1}{n h_n^{\bar{s}}}\sum_i \Iplus\, K\!\left(\Xh\right)\left(\Xh\right)^k, \quad k = 0,...,2p
\]
We expand $\Gammaplusbc{,p}{h_n}{} = \E[\Gammaplus]$
\begin{equation*}
\begin{split}
&= \frac{1}{h_n^{\bar{s}}} \int_{\eballboundright[h_n]} 
   K\left(\XXh\right)r_p\left(\XXh\right)r_p\left(\XXh\right)^T f\ppoint\, d\ppoint \\
&= \frac{1}{h_n^{\bar{s}}} \sum_{\curve}\int_{\curveball[h_n]} 
   K\left(\XXh\right)r_p\left(\XXh\right)r_p\left(\XXh\right)^T f\ppoint\, d\ppoint 
   + \frac{1}{h_n^{\bar{s}}} I_{ih_n} \\
&= \frac{1}{h_n^{\bar{s}}} \sum_{\curve}
   \int_{\freeregion}\int_{\discest}
   K\!\left(\tfrac{\|\bm{x}_{\cindex}\|}{h_n}\right)
   \!r_p\left(\tfrac{\|\bm{x}_{\cindex}\|}{h_n}\right)r_p\left(\tfrac{\|\bm{x}_{\cindex}\|}{h_n}\right)^T
   f(\bm{x}_{\cindex},\bm{x}_{\findex})\,
   d\bm{x}_{\cindex}\, d\bm{x}_{\findex}
   + \frac{1}{h_n^{\bar{s}}}I_{ih_n} \\
&=  \sum_{\curve}  h_n^{\ccard - \bar s}\int_{\freeregion}\int_{N^{\ccard}}
   K(\|\bm u\|)r_p(\|\bm u\|)r_p(\|\bm u\|)^T f(h_n\bm u,\bm x_{\findex})\,
   d\bm u\, d\bm x_{\findex}
   + \frac{1}{h_n^{\bar{s}}}I_{ih_n}
\end{split}
\end{equation*}
where the second equality comes from decomposing $\eballboundright[h_n]$ as the union of $\curveball[h_n]$, with $I_{ih_n}$ collecting overlap terms;  
the third equality follows from $\curveball = \freeregion \times N^{\ccard} $ and $\distvari=\|\bm X_{\cindex}\|$ on $\curveball[h_n]$; the last equality follows by the change of variables $\bm{x}_{\cindex}=h_n\bm u$, which maps $\discest$ to the normalized domain $N^{\ccard}$.  

% Heterogeneous part
% Averaging over $i$ gives
% \begin{equation*}
% \begin{split}
% \E[F_{k,d,g}(h_n)]
% & = \frac{1}{n}\sum_i  \sum_{\curve}
%    h_n^{\ccard - \bar s}\int_{\freeregion}\int_{N^{\ccard}}
%    K(\|\bm u\|)\|\bm u\|^k f(\bm u h_n,\bm x_{\findex})\,
%    d\bm u\, d\bm x_{\findex} + \frac{1}{n h_n^{\bar{s}}}I_{ih_n}.
% \end{split}
% \end{equation*}
%
Hence, $\Gammaplusbc{,p}{h_n}{}$ is bounded and bounded away from zero by Assumptions \ref{ass:pos}, \ref{ass:densitycont} and \ref{ass:kernel}.

%and the fact that $\sum_{\curve}\operatorname{Vol}(\cup\freeregion)$ is bounded since $|\mathcal{S}_i| = S$ for all $i$.

\medskip
\noindent\textbf{Variance concentration}
We now show that the variance of $F_{k,d,g}(h_n)$ converges to zero:
\begin{equation*}
\begin{split}
\V[F_{k,d,g}(h_n)] 
&= \frac{1}{n^2h_n^{2\bar{s}}}\sum_i 
   \V\!\left[ \Iplus K\!\left(\Xh\right)\left(\Xh\right)^k\right] \\
&\quad + \frac{1}{n^2h_n^{2\bar{s}}}\sum_i\sum_{j \in \bm{N}_i\setminus\{i\}}
   \C\!\left[ \Iplus K\!\left(\Xh\right)\!\left(\Xh\right)^k,\,
     \Iplus[j]K\!\left(\Xh\right)\left(\Xh\right)^k \right].
\end{split}
\end{equation*}
Expanding,
\begin{equation*}
\begin{split}
\V[F_{k,d,g}(h_n)] 
&= \frac{1}{n^2h_n^{2\bar{s}}}\sum_i 
    \E\!\left[ \Iplus K\!\left(\Xh\right)^2\left(\Xh\right)^{2k}\right] \\
&\quad + \frac{1}{n^2h_n^{2\bar{s}}}\sum_i\sum_{j \in \bm{N}_i\setminus\{i\}} 
   \E\!\left[ \Iplus K\!\left(\Xh\right)\!\left(\Xh\right)^k\;
      \Iplus[j]K\!\left(\Xh\right)\left(\Xh\right)^k\right] \\
&\quad - \frac{1}{n^2h_n^{2\bar{s}}}\sum_i 
   \E\!\left[ \Iplus K\!\left(\Xh\right)\left(\Xh\right)^k\right]^2 \\
&\quad - \frac{1}{n^2h_n^{2\bar{s}}}\sum_i\sum_{j \in \bm{N}_i\setminus\{i\}} 
   \E\!\left[ \Iplus K\!\left(\Xh\right)\left(\Xh\right)^k\right] \,
   \E\!\left[  \Iplus[j] K\!\left(\Xh[k]\right)\left(\Xh[j]\right)^k\right].
\end{split}
\end{equation*}
The first term is $O((nh_n^{\bar{s}})^{-1}) = o(1)$, by the same arguments used in computing the expectation.
The second term is also $O((nh_n^{\bar{s}})^{-1})$: by the arithmetic–geometric inequality it is bounded by
\[
\frac{1}{nh_n^{2\bar{s}}} \max_i \E\!\left[\Iplus K\!\left(\frac{\tilde{X}_i}{h_n}\right)\left(\Xh\right)^k\right] 
\cdot \frac{1}{n}\sum_i |\bm{N}_i| 
= O((nh_n^{\bar{s}})^{-1}),
\]
since $\frac{1}{n}\sum_i |\bm{N}_i| = O(1)$ by Assumption \ref{ass:localdependence}. The last two terms are $O(n^{-1})$ by Assumption \ref{ass:localdependence}, since each expectation term is $O(h_n^{\bar{s}})$. Hence, the component-wise variance of $\Gammaplus$ converges to zero, which yields the first conclusion.  

\medskip
\noindent\textbf{Limiting expectation computation} 
We show the limit of $\Gammaplusbc{,p}{h_n}{}$ for $h_n \to 0$ by the following decomposition
\begin{equation*}
\begin{split}
\Gammaplusbc{,p}{h_n}{} = \sum_{\curve : \ccard = \bar s}
   \int_{\freeregion}\int_{N^{\bar{s}}}
   K(\|\bm u\|)r_p(\|\bm u\|)r_p(\|\bm u\|)^T f(\bm u h_n,\bm x_{\findex})\,
   d\bm u\, d\bm x_{\findex} + \frac{1}{n h_n^{\bar s}}I_{ih_n} + I(\ccard > \bar s)    
\end{split}
\end{equation*}
with 
\begin{equation*}
\begin{split}
I(\ccard > \bar{s})
& = \sum_{\curve : \ccard > \bar s}
   h_n^{\ccard - \bar s}\int_{\freeregion}\int_{N^{\ccard}}
   K(\|\bm u\|)r_p(\|\bm u\|)r_p(\|\bm u\|)^T f(\bm u h_n,\bm x_{\findex})\,
   d\bm u\, d\bm x_{\findex} 
   \end{split}
\end{equation*}
Both $I(\ccard > \bar{s})$ and the overlap terms are $O(h_n)$ ($I_{ih_n}$ are $O(h_n^{\bar s + 1})$, as shown in Theorem \ref{th:cont}). Moreover, by Assumption~\ref{ass:densitycont} and the Dominated Convergence theorem we have 
\begin{equation*}
    \sum_{\curve : \ccard = \bar s}
   \int_{\freeregion}\int_{\unitdisc[\bar s]}
   K(\|\bm u\|)r_p(\|\bm u\|)r_p(\|\bm u\|)^T f(\bm u h_n,\bm x_{\findex})\,
   d\bm u\, d\bm x_{\findex} = \limdensity \Gamma_p^{\bar{s}} + o(1)
\end{equation*}
Hence, $\Gammaplusbc{,p}{h_n}{} = \limdensity\cdot\Gamma_p^{\bar{s}} + o(1)$. The conclusions for $\Gammaminus$ follows by analogous arguments.
\end{proof}

\begin{lemma}[Convergence of $\tplus$ and $\tminus$]\label{lemma:convergencematricest}

Suppose Assumptions \ref{ass:consistency}--\ref{ass:localdependence}, \ref{ass:variances} and \ref{ass:kernel} hold. 
% For any nonnegative integer $k$, define
% \begin{equation*}
% \begin{split}
%     F_{k,d,g}(h_n) & = \frac{1}{n h_n^{\bar{s}}}\sum_i   
%     \Iplus\, K\!\left(\Xh\right)\left(\Xh\right)^k, \\
%     F_{k,d',g'}(h_n) & = \frac{1}{n h_n^{\bar{s}}}\sum_i  
%     \Iminus\, K\!\left(\Xh\right)\left(\Xh\right)^k,
% \end{split}
% \end{equation*}
% and let $\tilde{F}_{k,d,g}(h_n)$ and $\tilde{F}_{k,d',g'}(h_n)$ denote their expectations.  
If $n h_n^{\bar{s}} \to \infty$ and $h_n < \kappa$
then
\[
\tplus = \bar{t}_{d,g,p}(h_n) + o_p(1), \quad  \tminus = \bar{t}_{d',g',p}(h_n) + o_p(1)
\] 
where $\bar{t}_{d,g,p}(h_n)$ and $\bar{t}_{d',g',p}(h_n)$ are bounded.

Moreover, if $h_n \to 0$ 
    \[
    \bar{t}_{d,g,p}(h_n)  = \theta_{p,0}^{\bar{s}} \hspace{-1em} \int\limits_{\Frontier} \hspace{-1em}m_{d,g}\ppoint f\ppoint + o(1),
    \qquad 
    \bar{t}_{d',g',p}(h_n)  = \theta_{p,0}^{\bar{s}}\hspace{-1em}\int\limits_{\Frontier}\hspace{-1em}m_{d',g'}\ppoint f\ppoint + o(1).
    \]
\end{lemma}

% Proof: first compute expectation. Then show variance goes to zero. Finally, establish expectation limit. 
\begin{proof}

\noindent Since the procedure is analogous to Lemma \ref{lemma:convergencematricesgamma} we only sketch the proof. 

We first compute the limiting expectation of $\tplus$: 
\begin{equation*}
\begin{split}
    \E[\tplus] = & \sum_{\curve}  h_n^{\ccard - \bar s}\int_{\freeregion}\int_{N^{\ccard}}
   K(\|\bm u\|)r_p(\|\bm u\|) m_{d,g}(h_n\bm u,\bm x_{\findex}) f(h_n\bm u,\bm x_{\findex})\,
   d\bm u\, d\bm x_{\findex}
   + \frac{1}{h_n^{\bar{s}}}I_{ih_n} \\
   = & \theta^{\bar{s}}_{p,0} \int_{\Frontier}m_{d,g}\ppoint f\ppoint + o(1)
\end{split} 
\end{equation*}
by Assumption \ref{ass:cont}, \ref{ass:densitycont} and \ref{ass:kernel} and the Dominated Convergence Theorem. Similarly, one obtains the limiting expectation for $\tminus$.

Convergence to zero of the component-wise variance of $\tplus$ and $\tminus$ can also be shown similarly to Lemma~\ref{lemma:convergencematricesgamma} using boundedness of the conditional variance (Assumption \ref{ass:variances}).
\end{proof}

\begin{lemma}[Convergence of $\theta_{d,g,p,q}(h_n)$ and $\theta_{d',g', p, q}({h_n})$]\label{lemma:convergencematricestheta}

Suppose Assumptions \ref{ass:consistency}--\ref{ass:indrule}, \ref{ass:pos}, \ref{ass:densitycont}, \ref{ass:dependencyneighborhood}--\ref{ass:localdependence} and \ref{ass:kernel} hold. 
If $n h_n^{\bar{s}} \to \infty$ and $h_n < \kappa$
then
\[
\theta_{d,g,p,q}(h_n) = \thetaplusbc{p}{q}{h_n} + o_p(1), \quad  \theta_{d',g', p, q}({h_n}) = \thetaminusbc{p}{q}{h_n} + o_p(1)
\]. 
where $\thetaplusbc{p}{q}{h_n}$ and $\thetaminusbc{p}{q}{h_n}$ are bounded and bounded away from zero.

Moreover, if $h_n \to 0$ 
    \[
    \thetaplusbc{p}{q}{h_n}  = \limdensity \theta_{p,q}^{\bar{s}} + o(1),
    \qquad 
    \thetaminusbc{p}{q}{h_n} = \limdensity \theta_{p,q}^{\bar{s}} + o(1).
    \]
\end{lemma}

\begin{proof}
Since the procedure is again analogous to Lemma \ref{lemma:convergencematricesgamma} we only sketch the proof. We first compute the limiting expectation of $\theta_{d,g,p,q}(h_n)$ by a similar decomposition as in Lemma~\ref{lemma:convergencematricesgamma}:
\begin{equation*}
\begin{split}
\thetaplusbc{p}{q}{h_n} = \sum_{\curve : \ccard = \bar s}
   \int_{\freeregion}\int_{N^{\bar{s}}}
   K(\|\bm u\|)r_p(\|\bm u\|)\|\bm u \|^q f(\bm u h_n,\bm x_{\findex})\,
   d\bm u\, d\bm x_{\findex} + \frac{1}{n h_n^{\bar s}}I_{ih_n} + I(\ccard > \bar s)    
\end{split}
\end{equation*}
where $I(\ccard > \bar{s})$ collects the sum  of the integral terms over the pieces $\curve : \ccard > \bar s$, and $I_{ih_n}$ contains the overlap terms.
Hence, since $I(\ccard > \bar{s})$ and $I_{ih_n}$ are $O(h_n)$, Assumption~\ref{ass:densitycont} and the Dominated Convergence theorem yield  
\begin{equation*}
    \sum_{\curve : \ccard = \bar s}
   \int_{\freeregion}\int_{\unitdisc[\bar s]}
   K(\|\bm u\|)r_p(\|\bm u\|)\|\bm u\|^q f(\bm u h_n,\bm x_{\findex})\,
   d\bm u\, d\bm x_{\findex} = \limdensity \theta_{p,q}^{\bar{s}} + o(1)
\end{equation*}
Hence, $\thetaplusbc{p}{q}{h_n} = \limdensity \theta_{p,q}^{\bar{s}} +  o(1)$. Similarly, one obtains the limiting expectation of $\theta_{d',g',p,q}(h_n)$.
Convergence to zero of the component-wise variance of $\theta_{d,g,p,q}(h_n)$ and $\theta_{d,g',p,q}(h_n)$ is shown analogously to Lemma~\ref{lemma:convergencematricesgamma}.
\end{proof}

\begin{lemma}\label{lemma:subgraph}
Suppose Assumptions \ref{ass:consistency}--\ref{ass:indrule}, \ref{ass:pos}, \ref{ass:densitycont}, \ref{ass:dependencyneighborhood}--\ref{ass:localdependence}, \ref{ass:commonpieces}, and \ref{ass:kernel} hold. If $n h_n^{\bar s}\to\infty$ and $h_n < \kappa$, then for each $\bullet\in\{(d,g), (d',g')\}$,
\[
\frac{1}{n h_n^{\bar s}}\sum_{i=1}^n\sum_{j\in \bm N_i} W^{\bullet}_{ij}(h_n)
\;=\; \bar{\bm D}^{\bullet}(h_n) + \bar{\bm N}^{\bullet}(h_n) + o_p(1).
\]
where $\bar{\bm D}^{\bullet}(h_n)$ is bounded and bounded away from zero and $\bar{\bm N}^{\bullet}(h_n)$ is bounded.

\noindent Moreover, if $h_n\to 0$,
\[
\bar{\bm D}^{\bullet}(h_n)
= \limdensity \int_{\unitdisc[\bar s]} K(\|\bm u\|)^2\, d\bm u + o(1),
\qquad
\bar{\bm N}^{\bullet}(h_n)=o(1),
\]
and for the cross-side case $\bullet=(d,g;d',g')$,
\[
\bar{\bm D}^{d,g;d',g'}(h_n)=0,
\qquad
\bar{\bm N}^{d,g;d',g'}(h_n)=o(1).
\]
\end{lemma}

% Proof 
\begin{proof}
\medskip
\noindent\textbf{Expectation calculation.}
We start with $\bm W^{d,g}(h_n)$. 
\begin{equation}\label{eq:avgdegreeexpansion}
\begin{split}
\frac{1}{nh_n^{\bar s}} \sum_i \E\!\left[\sum_{j\in \bm N_i} W^{d,g}_{ij}(h_n)\right] 
=& \underbrace{\frac{1}{nh_n^{\bar s}} \sum_i \E\left[\Iplus \Kh^2\right]}_{\bm{\bar{D}}^{d,g}(h_n)}\\
+ &\underbrace{\frac{1}{nh_n^{\bar s}} \sum_i \sum_{j\in \bm N_i\setminus\{i\}} \E\left[\Iplus\Iplus[j]\Kh\Kh[j]\right]}_{\bm{\bar N}^{d,g}(h_n)}\\
\end{split}
\end{equation}
where $\bm{\bar{D}}^{d,g}(h_n)$ is bounded away from zero and bounded by Assumption \ref{ass:densitycont} and \ref{ass:kernel}, and $\bm{\bar{N}}^{d,g}(h_n)$ is bounded by Assumption \ref{ass:localdependence} and \ref{ass:kernel}.

\medskip
\noindent\textbf{Variance bound.}
We now show concentration of variance of $
\tfrac{1}{n h_n^{\bar s}}\sum_{i}\sum_{j\in \bm N_i} W^{d,g}_{ij}(h_n)$.

\noindent Expanding the second moment:
\begin{equation}\label{eq:secondmomentsubgraph}
\begin{split}
   \E\Bigg[\Bigg(\frac{1}{n h_n^{\bar{s}}}
   \sum_i \sum_{j \in \bm{N}_i} W_{ij}^{d,g}(h_n)\Bigg)^2\Bigg]
   &= \frac{1}{n^2 h_n^{2\bar{s}}}
      \sum_{i\neq j}\sum_{k \in \bm{N}_i}\sum_{l \in \bm{N}_j}
      \E\!\left[\Kh \Kh[j] \Kh[k] \Kh[l]\right] \\
   &\quad + \frac{1}{n^2 h_n^{2\bar{s}}}
      \sum_i \sum_{j \in \bm{N}_i}
      \E\!\left[\Kh^2 \Kh[j]^2\right] \\
   &\quad + \frac{1}{n^2 h_n^{2\bar{s}}}
      \sum_i \sum_{j \in \bm{N}_i}\sum_{k \in \bm{N}_i\setminus\{j\}}
      \E\!\left[\Kh^2 \Kh[j]\Kh[k]\right]
\end{split}
\end{equation}
The last two terms in \eqref{eq:secondmomentsubgraph} can be bounded by
\[
\frac{1}{n^2 h_n^{2\bar{s}}}\,
   \max_i \E\left[\Kh^4\right]\,
   \sum_i \big(|\bm{N}_{i,n}| + |\bm{N}_{i,n}|^2\big),
\]
which is $O((nh_n^{\bar{s}})^{-1})$ by Assumption~\ref{ass:localdependence} and since $\E\left[\Kh^4\right] = O(h_n^{\bar{s}})$.

The first term is bounded by 
\small{
\begin{equation}\label{eq:bigeqsubgraph}
    \begin{split}
        \E\Big[\Big(\frac{1}{nh_n^{\bar{s}}}\sum_i\sum_{j \in \bm{N}_i}W^{d,g}_{ij}(h_n)\Big)\Big]^2 +& \frac{1}{n^2h_n^{2\bar{s}}}\sum_i\sum_{j \in \bm{N}_i}\sum_{k \in \bm{N}_i\cup\bm{N}_j}\sum_{l \in \bm{N}_i\cup\bm{N}_j\cup \bm{N}_k}\hspace{-0.5em}\E\left[\Kh\Kh[j]\Kh[k]\Kh[l]\right] \\
        -& \E\left[\Kh\Kh[k]\right]\E\left[\Kh[j]\Kh[l]\right]\\
    \end{split}
\end{equation}}
By the arithmetic-geometric mean inequality, \eqref{eq:bigeqsubgraph} is bounded by  
\small{
\begin{equation*}
\begin{split}
        &\E\Big[\Big(\frac{1}{nh_n^{\bar{s}}}\sum_i\sum_{j \in \bm{N}_i}W_{ij}^{d,g}(h_n)\Big)\Big]^2 +  \frac{1}{n^2h_n^{2\bar{s}}}\max_i\E\left[\Kh^4\right]\sum_i\sum_{j \in \bm{N}_i}\sum_{k \in \bm{N}_i\cup\bm{N}_j}|\bm{N}_i \cup \bm{N}_j| + |\bm{N}_k| \\
        \leq & \E\Big[\Big(\frac{1}{nh_n^{\bar{s}}}\sum_i\sum_{j \in \bm{N}_i}W_{ij}^{d,g}(h_n)\Big)\Big]^2 + \frac{1}{nh_n^{2\bar{s}}}\max_i\E\left[\Kh^4\right]\frac{\sum_i|\bm{N}_i|^3 + 3\sum_{i,j}(\bm{W}^3)_{ij}}{n}\\
        \end{split}
\end{equation*}}
where the second summand is $O((nh_n^{\bar{s}})^{-1})$ by Assumption \ref{ass:localdependence}.
Hence, because 
\begin{equation*}
\V\Big[\frac{1}{nh_n^{\bar{s}}}\sum_i\sum_{j \in \bm{N}_i}W_{ij}^{d,g}(h_n)\Big] = \E\Big[\Big(\frac{1}{nh_n}\sum_i\sum_{j \in \bm{N}_i}W_{ij}^{d,g}(h_n)\Big)^2\Big] - \E\Big[\frac{1}{nh_n}\sum_i\sum_{j \in \bm{N}_i}W_{ij}^{d,g}(h_n)\Big]^2 
\end{equation*}

we obtain
\begin{equation*}
\begin{split}
    \V\Big[\frac{1}{nh_n^{\bar{s}}}\sum_i\sum_{j \in \bm{N}_i}W_{ij}^{d,g}(h_n)\Big] & \leq \frac{1}{n^2h_n^{2\bar{s}}} \max_i\E\left[\Kh^4\right]\Big(\sum_i(|\bm{N}_{i,n}| + |\bm{N}_{i,n}|^2) + \sum_i|\bm{N}_{i,n}|^3 + 3\sum_{i,j}(\bm{W}_n^3)_{ij}\Big) \\
    & = O((nh_n^{\bar{s}})^{-1}) \to 0
    \end{split}
\end{equation*}

\medskip
\noindent\textbf{Diagonal limiting contribution.} We now establish limit of \eqref{eq:avgdegreeexpansion} as $h_n \to 0$. The first summand limit in \eqref{eq:avgdegreeexpansion} is established using analgous arguments as in Lemma~\ref{lemma:convergencematricesgamma}, yielding
\[
\bm{\bar{D}}^{d,g}(h_n)
= \limdensity \int_{\unitdisc[\bar s]} K(\|\bm u\|)^2 \, d\bm u + o(1).
\]

\medskip
\noindent\textbf{Average degree limiting contribution.}
Consider 
\[
\E\!\left[\Iplus \Iplus[j]\Kh \Kh[j]\right], \qquad i\neq j.
\]
The domain of integration of this expectation is the intersection of the two neighborhoods
\[
\mathcal{B}^{d,g}_{h_n}(\Frontier) \cap \mathcal{B}^{d,g}_{h_n}(\mathcal{X}_{j\smallN_j}(d,g|d',g'))
=\bigcup_{\curve,\curve[j]}
\big(\mathcal{B}_{h_n}^{d,g}(\curve)\cap \mathcal{B}_{h_n}^{d,g}(\curve[j])\big).
\]

Moreover,  the functions $\distvari = \distvari(X_i,\pscore)$ and $\distvari[j] = \distvari[j](X_j,\bm{X}_{\smallN_j})$ may have common arguments if the index sets  $\tilde{\mathcal{S}_i} = (\mathcal{S}_i\cup \{i\})$ and $\tilde{\mathcal{S}_j}=(\mathcal{S}_j\cup \{j\})$ overlap. Let $\bm{X}_{\tilde{\smallN}_i\cup \tilde{\smallN}_j}$ be the random vector collecting the scores of units in $\tilde{\mathcal{S}}_i \cup \tilde{\mathcal{S}}_j$.

We can bound
\[
\E\!\left[\left|\Iplus \Iplus[j]\Kh \Kh[j]\right|\right]
\leq \sum_{\curve,\curve[j]}
\int_{\mathcal{B}_{h_n}^{d,g}(\curve)\cap \mathcal{B}_{h_n}^{d,g}(\curve[j])}
\left|K\!\left(\tfrac{\tilde X_i}{h_n}\right)
K\!\left(\tfrac{\tilde X_j}{h_n}\right)\right|
f(\bm{x}_{\tilde{\smallN}_i\cup\tilde{\smallN}_j})\,d\bm{x}_{\tilde{\smallN}_i\cup\tilde{\smallN}_j}.
\]
where $f(\bm{x}_{\tilde{\smallN}_i\cup\tilde{\smallN}_j})$ is the joint density of $\bm{X}_{\tilde{\smallN}_i\cup \tilde{\smallN}_j}$. Thus the intersection domain $\mathcal{B}_{h_n}^{d,g}(\curve)\cap \mathcal{B}_{h_n}^{d,g}(\curve[j])$ is contained in a hyper-rectangle of the form
\[
\prod_{z\in \cindex\cup F_{\curve[j]}} I_z(\curve)\;\times\;
\prod_{z\in \findex\cup R_{\curve[j]}} I_z(\curve, h_n),
\]
where the interval $I_z(\curve) = O(1)$ and the interval $I_z(\curve, h_n) = O(h_n)$.

The total volume of this rectangular set is $O(h_n^{|\cindex\cup F_{\curve[j]}|})$. Therefore, we obtain the uniform bound
\[
\E\!\left[\left|\Iplus \Iplus[j]\Kh \Kh[j]\right|\right]
\leq C\sum_{\curve,\curve[j]} h_n^{|\cindex\cup F_{\curve[j]}|} = O(h_n^{\bar s + 1}).
\]
since $|\cindex\cup F_{\curve[j]}|\geq \bar s+1$ by Assumption \ref{ass:commonpieces}. Hence, the second term in \eqref{eq:avgdegreeexpansion} is 
\[
\bm{\bar{N}}^{d,g}(h_n)=O(h_n),
\]
using the fact that $\frac{1}{n}\sum_i |\bm N_i|=O(1)$ by Assumption~\ref{ass:localdependence}.

The proof for the convergence of $\frac{1}{n h_n^{\bar s}}\sum_{i}\sum_{j\in \bm N_i} W^{d',g'}_{ij}(h_n)$ and $\frac{1}{n h_n^{\bar s}}\sum_{i}\sum_{j\in \bm N_i} W^{d,g,d',g'}_{ij}(h_n)$ can be shown analogously.
\end{proof}

%=======================================================
% Convergence of sample matrices
%=======================================================

% \medskip
% \begin{lemma}\label{lemma:convergencematrices}
% Suppose Assumptions \ref{ass:identification}--\ref{ass:localdependence} and \ref{ass:regularity}--\ref{ass:kernel} hold, and let $\Frontier$ be of dimension $|\mathcal{S}_i| + 1 - \bar{s}_i$, with $\sup_i |S_i| < \infty$. Let $\bar{s} = \inf_i \bar{s}_i$
% If $n h_n^{\bar{s}} \to \infty$ and $h_n < \kappa$, then
% $\Gammaplus = \Gammaplusbc{,p}{h_n}{} + o_p(1)$ and $\Gammaminus = \Gammaminusbc{,p}{h_n}{} + o_p(1)$. Moreover, if $h_n \to 0$ 
%     \[
%     \Gammaplusbc{}{h_n}{}  = \limdensity \Gamma_p^{\bar{s}} + o(1),
%     \qquad 
%     \Gammaminusbc{}{h_n}{} = \limdensity \Gamma_p^{\bar{s}} + o(1).
%     \]
% \end{lemma}

% % Proof
%  \begin{proof}
% \item The conclusion follows from Lemma \ref{lemma:kernelconvergence} by noting that the generic element of $\Gammaplus$ is $\Big[\frac{1}{nh_n^{\bar{s}}}\sum_i^n\Iplus\Kh \Big(\Xh\Big)^k\Big] = F_{k,d,g}(h_n)$, and the generic element of $\Gammaminus$ is $\Big[\frac{1}{nh_n^{\bar{s}}}\sum_i^n\Iminus\Kh \Big(\Xh\Big)^k\Big] = F_{k,d',g'}(h_n)$, for $k = 0,...,2p$. 
% \end{proof}

%=========================================================%% Lemma: Variance of the centered estimator
%=========================================================

\begin{lemma}[Variance of $t_{d,g,d',g'}^*(h_n)$]\label{lemma:variances}
Suppose Assumptions \ref{ass:consistency}--\ref{ass:localdependence},
\ref{ass:variances}, \ref{ass:commonpieces}, and \ref{ass:kernel} hold. If $h_n < \kappa$,
\[
n h_n^{\bar{s}}\V[t_{d,g,d',g'}^*(h_n)]
= \Psiplusbc{p}{}{h_n} + \Psiminusbc{p}{}{h_n} - \Psiplusminusbc{p}{}{h_n},
\]
is bounded and bounded away from zero. Moreover, if $nh_n^{\bar{s}}\to \infty$ and $h_n \to 0$
\[
\Psiplusbc{p}{}{h_n} + \Psiminusbc{p}{}{h_n} - \Psiplusminusbc{p}{}{h_n}
= (\omegaplus+\omegaminus)\Psi_p^{\bar{s}} + o(1).
\]
where for $\bullet\in \{(d,g), (d',g')\}$
where 
\[
\bar{\omega}_{\bullet}(0) = \int\limits_{\Frontier}
\hspace{-1em}\Big(\sigma_{\bullet}\ppoint+\Big(m_{\bullet}\ppoint - \frac{\int_{\Frontier}m_{\bullet}\ppoint f\ppoint}{\int_{\Frontier}f\ppoint}\Big)^2\Big) f\ppoint d\ppoint
\]

\end{lemma}

\begin{proof}
We start from
\[
\V[t_{d,g,d',g'}^*(h_n)]
= \V[\tplus[*]] + \V[\tminus[*]] - \C[\tplus[*], \tminus[*]].
\]
We establish the result for $\V[\tplus[*]]$; the arguments for $\V[\tminus[*]]$ and $\C[\tplus[*], \tminus[*])$ are analogous.

\medskip
\noindent\textbf{Decomposition of the variance}
Expanding the variance yields
\begin{equation}\label{eq:variancetstar}
\begin{split}
n h_n^{\bar{s}} \V[\tplus[*]]
&= \underbrace{\frac{1}{n h_n^{\bar{s}}}\sum_i
\E\!\big[\Iplus \Kh^2\, \rr\rr^T\, \nu_{i,d,g}^2\big]}_{T_1}\\
&\quad+ \underbrace{\frac{1}{n h_n^{\bar{s}}}\sum_i \sum_{j\in\bm N_i\setminus\{i\}}
\E\!\big[\Iplus \Iplus[j]\, \Kh \Kh[j]\, \rr\, r_p(\Xh[j])^T\, \nu_{i,d,g} \nu_{j,d,'g'}\big]}_{T_2}.
\end{split}
\end{equation}
Both terms are bounded and bounded away from zero under
Assumptions~\ref{ass:densitycont} and \ref{ass:kernel}.  
Moreover, by Assumption \ref{ass:variances} $|T_2| \le C\, {\bar{\bm N}}^{d,g}(h_n) $ for some constant $C>0$, and ${\bar{\bm N}}^{d,g}(h_n) = o(1)$ by Lemma~\ref{lemma:subgraph}.

\medskip
\noindent\textbf{Limit of $T_1$.}
Expanding $\nu_{i,d,g}^2$ gives
\begin{align*}
T_1
=& h_n^{-\bar{s}}\hspace{-1em}
\int\limits_{\eballboundright[h_n]}\!
K\left(\XXh\right)^2\, r_p\left(\XXh\right) r_p\left(\XXh\right)^T
\big[
\sigmaplus[x_i,\bm{x}_{\smallN_i}] + m_{d,g}\ppoint^2 \\  
& + \hspace{1em} 
(r_p(\tilde{X}\ppoint)^T\beta_{d,g,p}(h_n))^2
- 2\, m_{d,g}\ppoint\, r_p(\tilde{X}\ppoint)^T\beta_{d,g,p}(h_n)
\big]
\, f\ppoint\, d\ppoint.
\end{align*}
Using the boundary neighborhood decomposition and change of variable $\bm u = \bm x_{\cindex}/h_n$, we obtain
\begin{align*}
T_1
&= \sum_{h_i} h_n^{s_{\curve}-\bar{s}}
\!\int_{\freeregion}\!\int_{\unitdisc[s_{\curve}]}
K(\|\bm u\|)^2 r_p(\|\bm u\|) r_p(\|\bm u\|)^T
\big[
m_{d,g}(\bm u h_n, \bm x_{\findex})^2
+ \sigmaplus[\bm u h_n, \bm x_{\findex}]\\
&\quad
+ (r_p(\|\bm u\|h_n)^T\beta_{d,g,p}(h_n))^2
- 2\, m_{d,g}(\bm u h_n, \bm x_{\findex})\, r_p(\|\bm u\|h_n)^T \beta_{d,g,p}(h_n)
\big]
f(\bm u h_n, \bm x_{\findex})\, d\bm u\, d\bm x_{\findex}.
\end{align*}
As $h_n \to 0$
\[
r_p(\|\bm u\| h_n)\beta_{d,g,p}(h_n)
\;\to\;
\frac{\int_{\Frontier} m_{d,g}\ppoint f\ppoint}
     {\int_{\Frontier} f\ppoint},
\]
since $r_p(\|\bm u\|h_n)^T \beta_{d,g,p}(h_n) = r_p(\|\bm u\|)\Gammaplusbc{}{h_n}{}\bar{t}_{d,g,p}(h_n)$ and 
\[
\Gammaplusbc{}{h_n}{}\bar{t}_{d,g,p}(h_n) = (\Gamma_p^{\bar s})^{-1}\theta_{p,0}^{\bar{s}}
\frac{\int_{\Frontier} m_{d,g}\ppoint f\ppoint}
     {\int_{\Frontier} f\ppoint} + o(1)
\] 
by Lemma~\ref{lemma:convergencematricesgamma} and \ref{lemma:convergencematricest}, and $(\Gamma_p^{\bar s})^{-1}\theta_{p,0}^{\bar{s}} = e_1$, where \(e_1\) is the \(p\)-dimensional unit vector with first entry equal to~1 and all others equal to~0.

\noindent Then by continuity of $m_{d,g}(\cdot)$, $f(\cdot)$, $\sigmaplus[\cdot]$, 
(Assumptions~\ref{ass:densitycont}-\ref{ass:cont} and \ref{ass:variances}), and by the Dominated Convergence Theorem, $T_1 = \omegaplus \Psi_p^{\bar s} + o(1)$.

By the same arguments we obtain
\[
n h_n^{\bar{s}}\V[\tminus[*]] = \omegaminus\Psi_p^{\bar{s}}+o(1),
\qquad
n h_n^{\bar{s}}\C[\tplus[*],\tminus[*]]=o(1).
\]
Combining the above yields the conclusion.
\end{proof}

% \begin{equation*}
% \begin{split}
% T_1    &= \frac{1}{nh_n^{\bar{s}}}\sum_i\int\limits_{\eballboundright[h_n]}\kern-1em\sigmaplus[x_i, \bm{x}_{\smallN_i}]K\left(\XXh \right)^2r_p\left(\XXh\right)r_p\left(\XXh\right)^Tf\ppoint d\ppoint\\
%    & = \omegaplus \int\limits_{\unitdisc[\bar s]}K(||\bm{u}||)^2r_p(||\bm{u}||)r_p(||\bm{u}||)^T d\bm{u} + o(1)
% \end{split}    
% \end{equation*}
% using uniform continuity and boundedness of $f(\cdot)$  and $\sigmaplus[\cdot]$ (Assumption \ref{ass:densities} and \ref{ass:variances}).
%

%=========================================================
%   Theorem: CLT for distance-based estimator
%==========================================================

\begin{theorem}\label{th:asynormaltau}
Suppose Assumptions~\ref{ass:consistency}--\ref{ass:localdependence},
\ref{ass:regularity}, \ref{ass:commonpieces}, and~\ref{ass:kernel} hold.
If $n h_n^{\bar{s}} \to \infty$, $h_n \to 0$, and 
$h_n = O\!\left(n^{-1/(2p + 2 + \bar{s})}\right)$, then
\[
\sqrt{n h_n^{\bar{s}}}\,
\frac{(\estimatorapp - \boundeff) - h_n^{p+1}\bias}
{\sqrt{V_{d,g,d',g',p}(h_n)}}
\xrightarrow{d} \mathcal{N}(0,1),
\]
where $\bias = B_{d,g,d',g',p, p+1} + o(1)$ and $V_{d,g,d',g'p}(h_n) = V_{d,g,d',g',p} + o(1)$,
\[
B_{d,g,d',g',p, p+ 1} 
= \Big(\frac{\muplusderiv[p+1]-\muminusderiv[p+1]}{(p+1)!}\Big)e_1^\top (\Gamma_p^{\bar{s}})^{-1}\theta_{p,p+1}^{\bar{s}},
\quad
V_{d,g,d',g',p}
= \frac{\omegaplus + \omegaminus}{\limdensity^2}e_1^\top (\Gamma_p^{\bar{s}})^{-1}\Psi_p^{\bar{s}}(\Gamma_p^{\bar{s}})^{-1} e_1.
\]
\end{theorem}

\begin{proof}[Proof of Theorem \ref{th:asynormaltau}]
Define
\begin{equation*}
\begin{split}
\Zplus &= e_1^T \Gammaplusbc{,p}{h_n}{-1}\;
           \tfrac{1}{n h_n^{\bar{s}}}\,\Iplus \Kh \rr \nu_{i,d,g},\\
\Zminus&= e_1^T \Gammaminusbc{,p}{h_n}{-1}\;
           \tfrac{1}{n h_n^{\bar{s}}}\,\Iminus \Kh \rr \nu_{i,d',g'},
\end{split}
\end{equation*}
and set $\Z = \Zplus - \Zminus$. Then
\[
\sum_i \Z = e_1^T\Gammaplusbc{p,}{h_n}{-1}\tplus[*] - e_1^T\Gammaminusbc{p,}{h_n}{-1}\tminus[*]
\]

\medskip
\noindent\textbf{Variance.}
Denote $nh_n^{\bar{s}}\,\V\!\Big[\sum_i \Z\Big] 
= V_{d,g,d',g',p}(h_n)$. By Lemmas~\ref{lemma:convergencematricesgamma} and \ref{lemma:variances},
\[
V_{d,g,d',g',p}(h_n) =  \tfrac{\omegaplus+\omegaminus}{\limdensity}\,
  (\Gamma_p^{\bar{s}})^{-1}\Psi_p^{\bar{s}}(\Gamma_p^{\bar{s}})^{-1} + o(1).
\]

\medskip
\noindent\textbf{CLT via dependency graph.}
By Assumption~\ref{ass:dependencyneighborhood}, the collection $\{\Z\}_i$ admits dependency graph 
$\bm W_n$. Let $\tilde\sigma_n^2 = V_{d,g,d',g',p}(h_n)/nh_n^{\bar s}$, the variance of $\Z$, and set 
$\xi_n = \sum_i \Z/ \tilde\sigma_n$.  
Applying the Wasserstein bound of \citet[Theorem A.4]{leung20},
\begin{equation}\label{eq:dist2}
\begin{split}
\Delta(\xi_n,\mathcal{N}(0,1)) 
&\leq \tfrac{1}{\tilde\sigma_n^3}\max_i\E[|\Z|^3]\sum_i|\bm N_i|^2 \\
&\quad+ \tfrac{1}{\tilde\sigma_n^2}
\Big(\tfrac{4}{\pi}\max_i\E[\Z^4]\Big)^{1/2}
\Big(4\sum_i|\bm N_i|^3 + 3\sum_{i,j}(\bm W^3)_{ij}\Big)^{1/2}.
\end{split}
\end{equation}

\medskip
\noindent\textbf{Moment bounds.}
Using the $c_r$-inequality,
\[
\E[|Z_i|^3] \leq 4(\E[|\Zplus|^3]+\E[|\Zminus|^3]) 
= O(n^{-3}h_n^{-2\bar{s}}),
\]
and similarly,
\[
\E[Z_i^4] \leq 8(\E[\Zplus^4]+\E[\Zminus^4]) 
= O(n^{-4}h_n^{-3\bar{s}}).
\]
using boundedness of the third and fourth conditional moment of the outcome (Assumption \ref{ass:fourthmoment}), Assumptions \ref{ass:cont} and the fact that the domain of integration has volume proportional to $h_n^{\bar{s}}$, as shown, for example, in Lemma \ref{lemma:convergencematricesgamma}.

\medskip
\noindent\textbf{Rate of convergence.}
Plugging these bounds into \eqref{eq:dist2} and using 
Assumption~\ref{ass:localdependence}, we obtain
\[
\Delta(\xi_n,\mathcal{N}(0,1)) = O((n h_n^{\bar{s}})^{-1/2}) = o(1).
\]
Hence $\xi_n \xrightarrow{d} \mathcal{N}(0,1)$. 
%which implies
% \[
% \sqrt{n h_n^{\bar{s}}} \sum_i \Z
% \xrightarrow{d} \mathcal{N}\!\Big(0,\, \tfrac{\omegaplus+\omegaminus}{\limdensity^2} V_{p}\Big).
% \]

\medskip
\noindent\textbf{Conclusion.}
By Lemma~\ref{lemma:convergencematricesgamma},
$
\sqrt{n h_n^{\bar{s}}}\cdot \tfrac{\estimatorapp[*]}{\sqrt{V_{d,g,d',g',p}(h_n)}} = \xi_n + o_p(1)
$, so $\estimatorapp[*]$ (rescaled) has the same asymptotic distribution as $\xi_n$. Moreover, by Lemmas~\ref{lemma:convergencematricesgamma} and \ref{lemma:convergencematricestheta}, $h_n^{p+1}\bias = O(h_n^{p+1})$ and $T_{d,g,d'g'}(h_n) = O(h_n^{p+2})$ since the term $\E\big|\Xp\Wplus T_{d,g,p}/n\big| \le h_n^{p+2}\tfrac{\sup_{\tilde x}|\mu_{d,g}^{(p+2)}(\tilde x)|}{(p+2)!}\thetaplusbc{p}{p+2}{h_n}$, and analogously for  the term $\E\big|\Xp\Wminus T_{d',g',p}/n\big|$. Then Eq.\eqref{eq:decompositiontau} and $h_n = O(n^{-1/(2p+2 + {\bar{s}})})$ yield the conclusion.
\end{proof}

\begin{proof}[Proof of Theorem \ref{th:asynormal}]
The result follows from Theorem~\ref{th:asynormaltau} by setting $p = 1$ and, for notational simplicity, writing $B = B_{d,g,d',g',1,2}$ and $V = V_{d,g,d',g',1}$.
\end{proof}

%%=============================================
%%           Variance Estimation               
%%=============================================
\subsection{Variance Estimation}

Define 
\begin{equation}\label{eq:varestimatorappendix}
\begin{split}
    \hat{\Psi}_{d,g,p}(h_n) &= \Mplus \bm{W} \Mplus^T / n, \\
    \hat{\Psi}_{d',g',p}(h_n) &= \Mminus \bm{W} \Mminus^T / n, \\
    \hat{\Psi}_{d,g,d',g',p}(h_n) &= \Mplus \bm{W} \Mminus^T / n,
\end{split}
\end{equation}
where $\bm{W}$ is the dependency graph and
\begin{equation*}
\begin{split}
    \Mplus^T &= \Big[\Iplus[1]\Kh[1]\rr[1]\hat{u}_{1,d,g} \;\; \cdots \;\; \Iplus[n]\Kh[n]\rr[n]\hat{u}_{n,d,g}\Big], \\
    \Mminus^T &= \Big[\Iminus[1]\Kh[1]\rr[1]\hat{u}_{1,d',g'} \;\; \cdots \;\; \Iminus[n]\Kh[n]\rr[n]\hat{u}_{n,d',g'}\Big],
\end{split}
\end{equation*}
with $\hat{u}_{i,d,g}$ and $\hat{u}_{i,d',g'}$ denoting the regression residuals.

\medskip
Let
\[
\varianceconstant = \frac{V_{d,g,d',g'}(h_n)}{nh_n^{\bar{s}}}
\]
where $V_{d,g,d',g',p}(h_n)$ is defined in Theorem \ref{th:asynormaltau}. $\varianceconstant$ can be seen as the \qq fixed-bandwidth" asymptotic variance of $\estimatorapp$. 

An estimator of $\varianceconstant$ is
\begin{equation}\label{eq:varestimator}
    \hat{\mathcal{V}}_{d,g,d',g',p}(h_n)
    = \frac{1}{n}\, e_1^T\!\left[
        \hat{V}_{d,g,p}(h_n) + \hat{V}_{d',g',p}(h_n) - 2\,\hat{V}_{d,g,d',g',p}(h_n)
      \right]e_1,
\end{equation}
where
\begin{equation*}
\begin{split}
    \hat{V}_{d,g,p}(h_n) &= \Gammaplus^{-1}\,\hat{\Psi}_{d,g}(h_n)\,\Gammaplus^{-1}, \\
    \hat{V}_{d',g',p}(h_n) &= \Gammaminus^{-1}\,\hat{\Psi}_{d',g'}(h_n)\,\Gammaminus^{-1}, \\
    \hat{V}_{d,g,d',g',p}(h_n) &= \Gammaplus^{-1}\,\hat{\Psi}_{d,g,d',g'}(h_n)\,\Gammaminus^{-1}.
\end{split}
\end{equation*}
We show that this estimator is consistent for $\varianceconstant$. Convergence of this estimator to h the asymptotic variance $(nh_n^{\bar{s}})^{-1}V_{d,g,d',g',p}$ follows since $V_{d,g,d',g',p}(h_n) = V_{d,g,d',g',p} + o(1)$ for $h_n \to 0$ by Lemma \ref{lemma:convergencematricesgamma} and \ref{lemma:variances}.

\begin{lemma}\label{lemma:psiconsistency}
Suppose Assumptions~\ref{ass:consistency}--\ref{ass:localdependence},
\ref{ass:regularity}, \ref{ass:commonpieces}, and~\ref{ass:kernel} hold.
If $n h_n^{\bar{s}} \to \infty$, 
\begin{equation*}
\begin{split}
    %h_n^{\bar{s}}
    \hat{\Psi}_{d,g,p}(h_n) = \Psiplusbc{p}{}{h_n}  + o_p(1)\\
    %h_n^{\bar{s}}
    \hat{\Psi}_{d',g',p}(h_n) = \Psiminusbc{p}{}{h_n}  + o_p(1)\\
    %h_n^{\bar{s}}
    \hat{\Psi}_{d,g,d',g',p}(h_n) = \bar{\Psi}_{d,g,d',g',p}(h_n) +  o_p(1)
\end{split}
\end{equation*}
where $\Psiplusbc{p}{}{h_n} =  \omegaplus\Psi_p^{\bar{s}} +o(1)$, $\Psiminusbc{p}{}{h_n} =  \omegaminus\Psi_p^{\bar{s}} +o(1)$, and $\hat{\Psi}_{d,g,d',g',p}(h_n) = o(1)$ if $h_n \to 0$.

\begin{proof}
The generic element of $\hat{\Psi}_{d,g,p}(h_n)$ is 
\begin{equation}\label{eq:varitem}
    \frac{1}{nh_n^{\bar{s}}}\sum_i\sum_{j \in \bm{N}_i}
    \hat{u}_{i,d,g}\hat{u}_{j,d,g}\,
    \Iplus[i]\Iplus[j]\Kh[i]\Kh[j]\,
    \left(\Xh[i]\right)^l\left(\Xh[j]\right)^v,
    \qquad l,v=0,\dots,p.
\end{equation}
We prove the claim for $l,v=0$. The proof for the other elements is analogous. We have
\[
\hat{u}_{i,d,g} = ({\beta}_{d,g,p}(h_n)-\hat{\beta}_{d,g,p}(h_n))^Tr_p(\tilde{X}_i) + \nu_{i,d,g}, \quad  i = 1,..., n
\]
Expanding the product $\hat{u}_{i,d,g}\hat{u}_{j,d,g}$, expression \eqref{eq:varitem} becomes
\begin{align}\label{eq:expansion_uiuj}
\eqref{eq:varitem} 
&= \frac{1}{nh_n^{\bar{s}}}\sum_i\sum_{j \in \bm{N}_i}\Big[ \nonumber\\
&\quad ({\beta}_{d,g,p}(h_n) - \betaplus)^Tr_p(\tilde{X}_i)({\beta}_{d,g,p}(h_n) - \betaplus)^Tr_p(\tilde{X}_j) \tag{I}\nonumber\\
%&\quad + (\betaestimandplus - \betaplus)^Tr_p(\tilde{X}_i)\betaestimandplus^{(p+1)}\tilde{X}_j^{p+1} \tag{II}\nonumber\\
%&\quad + (\betaestimandplus - \betaplus)^Tr_p(\tilde{X}_j)\betaestimandplus^{(p+1)}\tilde{X}_i^{p+1} \tag{III}\nonumber\\
&\quad + \nu_{j,d,g}({\beta}_{d,g,p}(h_n) - \betaplus)^Tr_p(\tilde{X}_i) \tag{II}\nonumber\\
&\quad + \nu_{i,d,g}({\beta}_{d,g,p}(h_n) - \betaplus)^Tr_p(\tilde{X}_j) \tag{III}\nonumber\\
%&\quad + u_i\betaestimandplus^{(p+1)}\tilde{X}_j^{p+1} \tag{VI}\nonumber\\
%&\quad + u_j\betaestimandplus^{(p+1)}\tilde{X}_i^{p+1} \tag{VII}\nonumber\\
%&\quad + \tilde{X}_i^{p+1}\betaestimandplus^{2(p+1)}\tilde{X}_j^{p+1} \tag{VIII}\nonumber\\
&\quad + \nu_{i,d,g} \nu_{j,d,g} \tag{IV}\Big]\Iplus[i]\Iplus[j]\Kh[i]\Kh[j].
\end{align}
\noindent\textbf{Leading term (IV).}
For (IX), we have $\E[(IX)] = e_1\V[\tplus[*]]e_1 =  e_1^T\Psiplusbc{p}{}{h_n} e_1$ by Lemma \ref{lemma:variances}. Moreover, using the same bounding arguments as in Lemma~\ref{lemma:subgraph},
\begin{equation*}
\begin{split}
\V\Big[(IX)\Big] & \leq \frac{1}{n^2h_n^{2\bar{s}}} \max_i\E\left[\nu_{i,d,g}^4\Kh^4\right]\Big(\sum_i(|\bm{N}_{i,n}| + |\bm{N}_{i,n}|^2) + \sum_i|\bm{N}_{i,n}|^3 + 3\sum_{i,j}(\bm{W}_n^3)_{ij}\Big) \\
    & = O((nh_n^{\bar{s}})^{-1}) \to 0
\end{split}
\end{equation*}
since $\E\left[\nu_{i,d,g}^4\Kh^4\right]$ is bounded by Assumption~\ref{ass:fourthmoment}, \ref{ass:cont}, \ref{ass:densitycont} and \ref{ass:kernel}. 
Hence
\[
(IX) =  e_1^T\Psiplusbc{p}{}{h_n}e_1  + o_p(1).
\]
where $e_1^T\Psiplusbc{p}{}{h_n}e_1 = \omegaplus e_1^T\Psi_p^{\bar{s}}e_1 + o(1)$ if $h_n \to 0$ by Lemma~\ref{lemma:variances}.

\noindent\textbf{Remaining terms (I)-(III)}
Define 
\[
M(h_n) = \left[\frac{1}{nh_n^{\bar{s}}}\sum_i\sum_{j\in\bm N_i}
\rr \rr[j]^T\,
\Iplus[i]\Iplus[j]\Kh[i]\Kh[j]\right]
\]
Term (I) is equal to 
\[
{(I)} = \big[H^{-1}(h_n) ({\beta}_{d,g,p}(h_n) - \betaplus)\big]^T
M(h_n)\big[H^{-1}(h_n)({\beta}_{d,g,p}(h_n) - \betaplus)\big]
\]
The term $M(h_n)$ is $O_p(1)$, since for some $C > 0$ it is bounded by $C \cdot \tfrac{1}{nh_n^{\bar s}}\sum_i\sum_{j\in \bm N_i} W^{d,g}_{ij}(h_n)$ which is $O_p(1)$ by Lemma~\ref{lemma:subgraph}.
%as the extra polynomial weights are bounded on the support of $K$.  
Furthermore, $H^{-1}(h_n) ({\beta}_{d,g,p}(h_n) - \betaplus) = o_p(1)$ by Lemma \ref{lemma:convergencematricesgamma} and \ref{lemma:convergencematricest} as $nh_n^{\bar s} \to \infty$. Thus, $(\text{I}) = o_p(1)$. Convergence in probability to zero of $(II)-(III)$ can be proved similarly by factorizing $H^{-1}(h_n) ({\beta}_{d,g,p}(h_n) - \betaplus)$, yielding the conclusion. The proofs for $\hat{\Psi}_{d',g',p}(h_n)$ and $\hat{\Psi}_{d,g,d',g',p}(h_n)$ are analogous.
\end{proof}
\end{lemma}

\begin{theorem}\label{th:variance}
Suppose Assumptions~\ref{ass:consistency}--\ref{ass:localdependence},
\ref{ass:regularity}, \ref{ass:commonpieces}, and~\ref{ass:kernel} hold.
If $n h_n^{\bar{s}} \to \infty$ and $h_n \to 0$ 
\begin{equation*}
    nh_n^{\bar{s}}\hat{\mathcal{V}}_{d,g,d',g',p}(h_n) \overset{p}{\to} V_{d,g,d',g',p}(h_n) 
\end{equation*}
where $V_{d,g,d',g',p}(h_n) =  V_{d,g,d',g',p} + o(1) $ if $h_n \to 0$.
\end{theorem}

\begin{proof}
The proof follows from Lemma \ref{lemma:convergencematricesgamma} and \ref{lemma:psiconsistency}.  
\end{proof}
%==========================================================% Common distance variable
%=========================================================

\subsection{Common Distance Variable}

We consider the case where a non negligible fraction of connected units can share the same distance variable. Define $\bm{K}_{i} \subseteq (\bm{N}_{i}\setminus \{i\})$ as the set of indices such that for $j \in \bm{K}_{i,n}$, $|\cindex\cup F_{\curve[j]}| = \min\{\bar s_i, \bar{s}_j\}$ for some pieces $\curve$, $\curve[j]$, forming $\Frontier$ and $\bar{\mathcal{X}}_{j\smallN_j}(d,g|d',g')$. 

%Define the conditional covariances $ \sigma_{d,g}(x_i, \bm{x}_{\smallN_i}, x_j, \bm{x}_{\smallN_j})= \CE{Y_i(d,g),Y_j(d,g)}{(X_i, \pscore) = \ppoint, (X_j, \pscore[\smallN_j]) = x_j, \bm{x}_{\smallN_j}}$ and $ \sigma_{d',g'}(x_i, \bm{x}_{\smallN_i}, x_j, \bm{x}_{\smallN_j})= \CE{Y_i(d',g'),Y_j(d',g')}{(X_i, \pscore) = \ppoint, (X_j, \pscore[\smallN_j]) = x_j, \bm{x}_{\smallN_j}}$ 

% Define  $\covplus[x_i, \bm{x}_{\smallN_i}, x_j, \bm{x}_{\smallN_j}]= \CE{u_i, u_j}{(X_i, \pscore) = \ppoint, (X_j, \pscore[\smallN_j]) = x_j, \bm{x}_{\smallN_j}}$, for $\ppoint$, $(x_j, \bm{x}_{\smallN_j}) \in \scorespace(d,g)$, and define $ \covminus[x_i, \bm{x}_{\smallN_i}, x_j, \bm{x}_{\smallN_j}]$ similarly for $(x_i, \bm{x}_{\smallN_i})$, $(x_j, \bm{x}_{\smallN_j}) \in \scorespace(d',g')$. 
 
\begin{lemma}\label{lemma:masspoints}
Suppose Assumptions~\ref{ass:consistency}--\ref{ass:localdependence},
\ref{ass:variances}, and~\ref{ass:kernel} hold.
If $n h_n^{\bar{s}} \to \infty$ and $h_n \to 0$ 
%Assume $\frac{1}{n}\sum_i\sum_{j \in \bm{K}_{i,n}}|\bm{K}_{i,n}| = O(1)$, and bounded away from zero.
 \begin{equation*}
     nh_n^{\bar s}\V[t_{d,g,d',g'}^*(h_n)] = (\omegaplus + \omegaminus)\Psi_p^{\bar{s}} + R_n + o(1)
 \end{equation*}
 where $R_n = O(1)$ collects the covariance contribution from $i,j$, with $j \in \bm{K}_i$.
\end{lemma}

\begin{proof}
Consider $\V[\tplus[*]]$. As in Lemma~\ref{lemma:variances}, we can write
\begin{equation}\label{eq:variancecommon}
\begin{split}
n h_n^{\bar{s}}\V[\tplus[*]]
&=\underbrace{\frac{1}{n h_n^{\bar{s}}}\sum_i\E\!\Big[\Iplus\Kh^2\,\rr\rr^T\,\errori^2\Big]}_{T_1}\\
&\quad+\underbrace{\frac{1}{n h_n^{\bar{s}}}\sum_i\sum_{j\in\bm N_i\setminus\{i\}}
\E\!\Big[\Iplus\Iplus[j]\Kh\Kh[j]\,\rr\,r_p\left(\Xh[j]\right)^T\,\errori u_j\Big]}_{T_2}.
\end{split}
\end{equation}
The first term $T_1$ is exactly as in Lemma~\ref{lemma:variances}, giving
\[
T_1 \;=\; \omegaplus \int_{\unitdisc[\bar s]}K(\|\bm u\|)^2 r_p(\bm u) r_p(\bm u)^T\, d\bm u + o(1).
\]
For $T_2$, decompose neighbors $j \in \bm{N}_i$ into those in $\bm K_i$ and the remainder:
\begin{equation}\label{eq:covcommondist}
\begin{split}
T_2 &= \frac{1}{n h_n^{\bar{s}}}\sum_i\sum_{j\in\bm K_i} \E[\cdots]
\;+\;\frac{1}{n h_n^{\bar{s}}}\sum_i\sum_{j\in\bm N_i\setminus(\{i\}\cup \bm K_i)} \E[\cdots].
\end{split}
\end{equation}
The second sum is $o(1)$ by the same arguments as in Lemma~\ref{lemma:variances}, since for such pairs  with 
$|\cindex\cup F_{\curve[j]}|\geq \bar s+1$ for all $\curve$, $\curve[j]$.  

For $j\in\bm K_i$, for some $\curve$, $\curve[j]$ $|\cindex \cup F_{\curve[j]}| = \bar{s}$. Thus
\[
\E[\cdots] \;=\; O(h_n^{\bar s}), \qquad
\frac{1}{n h_n^{\bar{s}}}\sum_i\sum_{j\in\bm K_i}\E[\cdots] \;=\; R_{d,g,n},
\]
since all terms in $\E[\cdots]$ are uniformly bounded. Moreover, $R_{d,g,n}$ is $O(1)$ because $\tfrac{1}{n}\sum_i|\bm K_i|\leq \tfrac{1}{n}\sum_i|\bm N_i|=O(1)$.  
Hence
\[
n h_n^{\bar{s}}\V[\tplus[*]]
\;=\;\omegaplus \Psi_p^{\bar s}\;+\;R_{d,g,n}\;+\;o(1).
\]
Analogous arguments yield $nh_n^{\bar{s}}\V[\tminus[*]] = \omegaminus \Psi_p^{\bar s} + R_{d',g',n} + o(1)$ and $
n h_n^{\bar{s}}\C[\tplus[*],\tminus[*]] = R_{d,g,d',g',n} + o(1)$ 
with each $R_{\cdot,n}=O(1)$. Assume $R_n \to R_p$.
Letting $R_n = R_{n, d,g} + R_{n, d,g} - 2R_{n, d,g, d',g'}$ yields the conclusion.
\end{proof}

\begin{theorem}\label{th:varmass}
Suppose Assumptions~\ref{ass:consistency}--\ref{ass:localdependence},
\ref{ass:regularity}, \ref{ass:commonpieces}, and~\ref{ass:kernel} hold.
If $n h_n^{\bar{s}} \to \infty$, $h_n \to 0$, and 
$h_n = O\!\left(n^{-1/(2p + 2 + \bar{s})}\right)$, then
\[
\sqrt{n h_n^{\bar{s}}}\,
\frac{(\estimatorapp - \boundeff) - h_n^{p+1}\bias}
{\sqrt{V_{d,g,d',g',p}(h_n)}}
\xrightarrow{d} \mathcal{N}(0,1),
\]
where $\bias$ is as in Theorem \ref{th:asynormaltau} and 
\[
V_{p}(h_n)
= \frac{\omegaplus + \omegaminus}{\limdensity}e_1^T(\Gamma_p^{\bar{s}})^{-1}(\Psi_p^{\bar{s}} + R_p^{\bar{s}})(\Gamma_p^{\bar{s}})^{-1}e_1+ o(1).
\]
\end{theorem}
\begin{proof}
The proof follows from analogous arguments as Theorem \ref{th:asynormaltau} and using Lemma \ref{lemma:convergencematricesgamma}, \ref{lemma:convergencematricestheta} and \ref{lemma:masspoints}.
\end{proof}

\subsection{Differentiability of $\muplus$ and $\muminus$}\label{appendix:differentiability}
The bias properties of $\estimatorapp$ hinge on Assumption~\ref{ass:smoothness}, which imposes smoothness of $\muplus$ and $\muminus$. Continuity of $m_{d,g}\ppoint$ and $m_{d',g'}\ppoint$ (or a stronger version continuity condition when causal effects are heterogeneous) is sufficient for consistency of the estimator, i.e.\ convergence to the estimand (see Theorem~\ref{th:heterogeneousconvergence}). However, obtaining the quadratic rate of bias decay, $h_n^{2+2p}$, requires differentiability of $\muplus$ and $\muminus$. Verifying this condition can be challenging. Here, we illustrate a simple case where this assumption is satisfied--namely, in the estimation of boundary direct effects.  

Consider
\[
\mu_{1,g}(\tilde{x}_i)
= \E\!\left[Y_i(1,g) \;\middle|\; \distvari=\tilde{x}_i,\; D_i=1,\; G_i=g\right].
\]
For direct boundary effects, the Euclidean distance to the effective treatment boundary is $\distvari = |X_i|$, so we may parametrize
\[
\mu_{1,g}(\epsilon)
= \frac{\int_{\mathcal{X}_{\smallN_i}(g)} m_{1,g}(\epsilon,\bm{x}_{\smallN_i})\, f(\epsilon,\bm{x}_{\smallN_i})\, d\bm{x}_{\smallN_i}}
       {\int_{\mathcal{X}_{\smallN_i}(g)} f(\epsilon,\bm{x}_{\smallN_i})\, d\bm{x}_{\smallN_i}}.
\]
where $\mathcal{X}_{\smallN_i}(g)$ is the set of $\bm_{\smallN_i}$ where $e(\bm{x}_{\smallN_i}) = g$.
Assume that, in a neighborhood $\mathcal{B}_{\kappa}(\mathcal{X}_{i\smallN_i}(1,g,|0,g))$ of $\mathcal{X}_{i\smallN_i}(1,g,|0,g)$, both $f$ and $m_{d,g}$ are $s$-times continuously differentiable in $\epsilon$ for all $d,g$. For $0 \le k \le s$, the map  
$
(\epsilon,\bm{x}_{\smallN_i}) \;\mapsto\; \partial_\epsilon^k m_{d,g}(\epsilon,\bm{x}_{\smallN_i})
$
is continuous and bounded on $\mathcal{B}_{\kappa}(\mathcal{X}_{i\smallN_i}(1,g,|0,g))$. Therefore, by differentiating under the integral sign we obtain for $\epsilon < \kappa$
\[
\partial_\epsilon^k \int_{\mathcal{X}_{\smallN_i}(g)} m_{1,g}(\epsilon,\bm{x}_{\smallN_i}) f(\epsilon,\bm{x}_{\smallN_i}) \, d\bm{x}_{\smallN_i}
= \int_{\mathcal{X}_{\smallN_i}(g)} \partial_\epsilon^k m_{1,g}(\epsilon,\bm{x}_{\smallN_i}) f(\epsilon,\bm{x}_{\smallN_i}) \, d\bm{x}_{\smallN_i},
\]
which is continuous as $\epsilon \to 0$ by the Dominated Convergence Theorem. Similarly,  
\[
\partial_\epsilon^k\int_{\mathcal{X}_{\smallN_i}(g)}  f(\epsilon,\bm{x}_{\smallN_i}) \, d\bm{x}_{\smallN_i}
= \int_{\mathcal{X}_{\smallN_i}(g)} \partial_\epsilon^k f(\epsilon,\bm{x}_{\smallN_i}) \, d\bm{x}_{\smallN_i}
\]
Hence, $\mu_{1,g}(\epsilon)$ is $s-$times continuously differentiable being the ratio of two continuously differentiable functions. Analogously, $\mu_{0,g}(\epsilon)$ is also $s$-times continuously differentiable.

\subsection{Bias Correction}\label{appendix3:biascorrection}

In this section, we establish the asymptotic normality of the bias-corrected estimator $\estimatorbcapp$ of $\boundeff$ \[
\estimatorbcapp = \estimatorapp - \biasbcapp,
\]
where $\biasbcapp$ is equal to
\[
h_n^{p+1}e_{p+1}^T\big[\betaminusbc \hat{B}_{d',g',p,p+1}(h_n) -\betaplusbc\hat{B}_{d,g,p,p+1}(h_n)\big],
\]
$\betaplusbc$ and $\betaminusbc$ are the $(p+1)$-order local polynomial estimators with bandwidth $b_n$, $e_{p+1}$ is the $p+2$ -dimensional vector with the $p+2$-th entry equal to 1 and all other zeros, and $\hat{B}_{\bullet,p,p+1}(h_n) = e_1^T{\Gamma}^{-1}_{\bullet, p}(h_n)\theta_{\bullet,p, p + 1}(h_n)$ (see Subsection \ref{subsec:notation} for the related definitions).

Since most passages are similar to the derivations for the asymptotic normality of $\estimator$ without bias correction, we only sketch the proof.

We consider the centered estimators. 
\[
\estimatorbcapp[*]= \estimatorapp[*] - \biasbcapp[*] 
\]
where $\estimatorapp[*]$ is defined in Subsection \ref{subsec:notation}, and $\biasbcapp[*]$ uses the centered versions of 
$\betaplusbc$ and $\betaminusbc$, obtained by replacing $Y_i$ in their expressions with 
\[
\nu_{i, \bullet, p+1}(b_n)
= Y_i - \mathbf r_{p+1}(\tilde X_i)^T\,\beta_{\bullet,p+1}(b_n),\quad \bullet \in \{(d,g), (d'g')\}
\] 
with $\beta_{\bullet,p+1}(b) = \argmin\limits_{\bm{b} \in \mathbbm{R}^{p+2}}\E\Big[\sum_iI_{i, \bullet} (Y_i - \bm r_{p+1}(\distvari)^T\bm{b})^2\cdot K_{b^{\bar{s}}}(\distvari)\Big]$.

Under Assumption \ref{ass:smoothness}, if $\max\{h_n,b_n\}<\kappa$, a Taylor expansion yields
\begin{equation}\label{eq:decompositiontaubc}
    \begin{split}
       \estimatorbcapp = & \boundeff + h_n^{p+1}\bias + T_{d,g,d'g'}(h_n)\\
       - & h_n^{p+1}\biasfinite{d,g,d',g'}{p}{p+1}{h_n} -  h_n^{p+1}b_n\bigbiasbc + T^{bc}_{d,g,d',g'}(h_n, b_n) \\
       + & \estimatorbcapp[*]
    \end{split}
\end{equation}
where $\bias$ and $T_{d,g,d'g'}(h_n)$ are defined in Subsection \ref{subsec:asytheory}, 
$\biasfinite{d,g,d',g'}{p}{p+1}{h_n} = \tfrac{\muplusderiv[(p+1)]}{(p+1)!}\hat{B}_{d,g,p,p+1}(h_n)- \tfrac{\muminusderiv[(p+1)]}{(p+1)!}\hat{B}_{d',g',p,p+1}(h_n)$, with $
\hat{B}_{\bullet, p,p+1}(h_n)= e_1^T\Gammaplus[-1]\thetaplus $, and $\bigbiasbc$ is equal to 
\begin{equation*}
    \frac{\muplusderiv[(p+2)]}{(p+2)!}\biasfinite{d,g}{p+1}{p+2}{b_n}\frac{\biasplus}{(p+1)!} - \frac{\muminusderiv[(p+2)]}{(p+2)!}\biasfinite{d',g'}{p+1}{p+2}{b_n}\frac{\biasminus}{(p+1)!}
\end{equation*}
with $\hat{B}_{\bullet, p+1,p+2}(h_n)= e_1^T{\Gamma}^{-1}_{\bullet, p+1}(h_n){\theta}_{\bullet, p+1, p+2}(h_n)$, and ${B}_{\bullet, p,p+1}(h_n)= e_1^T{\bar{\Gamma}}^{-1}_{\bullet, p+1}(h_n){\bar{\theta}}_{\bullet, p, p+1}(h_n)$.

\medskip
We denote the variance and covariance of $t_{d,g,p+1}^*(b_n)$ and $t_{d',g',p+1}^*(b_n)$, multiplied by $nb_n^{\bar s}$, by $\Psiplusbc{p+1}{}{b_n}$, $\Psiminusbc{p+1}{}{b_n}$ and $\Psiplusminusbc{p+1}{}{b_n}$,  and we let 
\begin{equation*}
\begin{split}
    \Psiplusbc{p,}{p+1}{h_n,b_n} & = \frac{n(h_nb_n)^{\bar{s}}}{m_n^{\bar{s}}}\C[t_{d,g,p}^*(h_n), t_{d,g,p+1}^*(b_n)] \\
    \Psiminusbc{p,}{p+1}{h_n,b_n} & = \frac{n(h_nb_n)^{\bar{s}}}{m_n^{\bar{s}}}\C[t_{d',g',r}^*(h_n), t_{d',g',p+1}^*(b_n)] \\
    \Psiplusminusbc{p,}{p+1}{h_n,b_n} &= \frac{n(h_nb_n)^{\bar{s}}}{m_n^{\bar{s}}}\C[t_{d,g,p}^*(h_n), t_{d',g',p+1}^*(b_n)]
\end{split}
\end{equation*}
where $m_n = \min\{h_n,b_n\}$. Further define $\variancebc = \variancebcplus + \variancebcminus - 2\covarbc$ where
\begin{equation*}
\begin{split}
    \variancebcplus
    & =  \frac{1}{nh_n^{\bar{s}}}e_1^T\Gammaplusbc{,p}{h_n}{-1}\Psiplus\Gammaplusbc{,p}{h_n}{-1}e_1 \\
    &+ \frac{1}{nb_n^{\bar{s}}}\frac{h_n^{2p + 2}}{b_n^{2+2p}}e_{p+1}^T\Gammaplusbc{,p+1}{b_n}{-1}\Psiplusbc{p+1}{}{b_n}\Gammaplusbc{,p+1}{b_n}{-1}e_{p+1}) \times(e_1^T\Gammaplusbc{,p+1}{b_n}{-1}\thetaplusbc{p}{p+1}{h_n})^2 \\
    &-2\frac{m_n^{\bar{s}}}{n(h_nb_n)^{\bar{s}}}\frac{h_n^{p+1}}{b_n^{p+1}}(e_1^T\Gammaplusbc{,p}{h_n}{-1}\Psiplusbc{p}{,p+1}{h_n, b_n}\Gammaplusbc{,p+1}{b_n}{-1}e_{p+1}) \\
    &\times(e_1^T\Gammaplusbc{,p+1}{h_n}{-1}\thetaplusbc{p}{p+1}{h_n})
     \\
    \variancebcminus 
    & =  \frac{1}{nh_n^{\bar{s}}}e_1^T\Gammaminusbc{,p}{h_n}{-1}\Psiminusbc{p}{}{h_n}\Gammaminusbc{,p}{h_n}{-1}e_1 \\
    & + \frac{1}{nb_n^{\bar{s}}}\frac{h_n^{2p + 2}}{b_n^{2+2p}}e_{p+1}^T\Gammaminusbc{,p+1}{b_n}{-1}\Psiminusbc{p+1}{}{b_n}\Gammaminusbc{,p+1}{b_n}{-1}e_{p+1} \times(e_1^T\Gammaminusbc{,p}{h_n}{-1}\thetaminusbc{p}{p+1}{h_n})^2 \\
    &-2\frac{m_n^{\bar{s}}}{n(h_nb_n)^{\bar{s}}}\frac{h_n^{p+1}}{b_n^{p+1}}(e_1^T\Gammaminusbc{,p}{h_n}{-1}\Psiminusbc{p}{,p+1}{h_n, b_n}\Gammaminusbc{,p+1}{b_n}{-1}e_{p+1} \\
    &\times(e_1^T\Gammaminusbc{,p}{h_n}{-1}\thetaminusbc{p}{p+1}{h_n})
\end{split}    
\end{equation*}
The first two terms represent the asymptotic variance, for $n \min\{h_n^{\bar s}, b_n^{\bar s}\} \to \infty$ of the (centered) bias-corrected estimator to the right and left of the cutoff respectively, which includes the variance of the original centered estimator, the variance of the centered bias correction, and their covariance.
\noindent$\covarbc$ is given by 
\begin{equation*}
    \begin{split}
        \covarbc &= \covarest{p}{h_n} + h_n^{2(p+1)}\covarest{p+1}{b_n}\biasplusbc\biasminusbc \\
    & - h_n^{p+1}\covarest{p+1, p,p+1}{h_n,b_n}B_{d,g,p,p+1}(b_n) \\
    & - h_n^{p+1}\covarest{p+1,p,p+1}{b_n,h_n}\biasplusbc 
    \end{split}
\end{equation*}
where 
\begin{equation*}
    \begin{split}
         \covarest{p}{h_n} &=  \frac{1}{nh_n^{\bar{s}}}e_1^T\Gammaplusbc{,p}{h_n}{-1}\Psiplusminusbc{p}{}{h_n}\Gammaminusbc{,p}{h_n}{-1}e_1 \\
         \covarest{p+1,p,p+1}{h_n,b_n} & =  \frac{m_n^{\bar{s}}}{n(h_nb_n)^{\bar{s}}}\frac{1}{b_n^{p+1}}(p+1)!e_1^T\Gammaplusbc{,p}{h_n}{-1}\Psiplusminusbc{p}{,p+1}{h_n,b_n} \Gammaplusbc{,p+1}{b_n}{-1}e_{p+1}\\
         \covarest{p+1,p,p+1}{b_n,h_n} & =  \frac{m_n^{\bar{s}}}{n(h_nb_n)^{\bar{s}}}\frac{1}{b_n^{p+1}}(p+1)!e_{p+1}^T\Gammaplusbc{,p+1}{b_n}{-1}\Psiplusminusbc{p}{,p+1}{b_n, h_n} \Gammaminusbc{,p}{h_n}{-1}e_{1}
    \end{split}
\end{equation*}

\medskip
\noindent By similar arguments as Lemma~\ref{lemma:variances}, for $n\min\{h_n^{\bar{s}},b_n^{\bar{s}}\}\to \infty$ and $\max\{h_n, b_n\} < \kappa $
\[
\Psiplus,\Psiminus = O\!\left(\frac{1}{nh_n^{\bar{s}}}\right), 
\qquad 
\Psiplus[b_n],\Psiminus[b_n] = O\!\left(\frac{1}{nb_n^{\bar{s}}}\right).
\]
and the cross–bandwidth terms satisfy
\[
\Psiplusbc{p}{,q}{h_n,b_n},\;\Psiminusbc{p}{,q}{h_n,b_n}
= O\!\left(\frac{m_n^{\bar{s}}}{n(h_nb_n)^{\bar{s}}}\right),
\qquad
\Psiplusminusbc{p}{,q}{h_n,b_n}
= O\!\left(\frac{m_n^{\bar{s} + 1}}{n(h_nb_n)^{\bar{s}}}\right),
\]

\begin{theorem}\label{th:asybiascorretiontau}
Suppose Assumptions~\ref{ass:consistency}--\ref{ass:localdependence},
\ref{ass:regularity}, \ref{ass:commonpieces}, and~\ref{ass:kernel} hold. If $n\min\{h_n^{\bar{s}},b_n^{\bar{s}}\}\to \infty$, $n\min\{h_n^{2p+2+\bar{s}},b_n^{2p+2+\bar{s}}\}\max\{h_n^2,b_n^{2}\} \to 0$ and $\max\{h_n, b_n\} < \kappa$:
\begin{equation*}
    \frac{\estimatorbcapp - \boundeff}{\sqrt{\variancebc}}\xrightarrow{d} \mathcal{N}(0, 1)
\end{equation*}
\end{theorem}

\begin{proof}
Consider $\Zbc = \Zplusbc - \Zminusbc$, where $\Zplus = \Zplusbcone -\Zplusbctwo$ with 
\begin{equation*}
\begin{split}
     \Zplusbcone =&  e_1^T\Gammaplusbc{,p}{h_n}{-1}\Iplus\Kh\rr\nu_{i,d,g,p}(h_n)/(nh_n^{\bar{s}}), \\
     \Zplusbctwo = & \frac{h_n^{p+1}b_n^{-p-1}}{nb_n^{\bar{s}}}\biasplus 
    \times e_{p+1}^T\bar{\Gamma}_{d,g,p+1}^{-1}(b_n)\Iplus K\Big(\frac{\tilde{X}_i}{b_n}\Big)r_{p+1}\Big(\frac{\tilde{X}_i}{b_n}\Big)\nu_{i,d,g,p+1}(b_n)
\end{split}  
\end{equation*}
and $\Zminusbc$ is defined analogously. Here we denote $\nu_{i,\bullet, r}(h) = Y_i - \bm r_r(\distvari)\beta_{\bullet,r}(h)$, the residual obtained from the outcome linear approximation using the population linear projection coefficient $\beta_{\bullet,r}(h)$. Then
\[
\V\!\Big[\sum_i \Zbc\Big] \;=\; \variancebc
= O_p\!\Big(\frac{1}{n h_n^{\bar{s}}}\Big)
+ O_p\!\Big(\frac{h_n^{2(p+1)}}{n b_n^{2(p+1)+\bar{s}}}\Big).
\]
Let $\xi_n = \sum_i \Zbc / \sigma_n$ with $\sigma_n^2 = \variancebc$.  
By Assumption~\ref{ass:dependencyneighborhood}, $\{\Zbc\}_{i=1}^n$ has dependency graph $\bm W_n$.  
Stein’s method and \citet[Theorem~A.4]{leung20} then yield
\begin{equation}\label{eq:distbc}
    \begin{split}
        \Delta({\xi}_{n}, \mathcal{N}(0,1)) & \leq \frac{1}{\sigma_{n}^3}\E[|\Zbc|^3]\sum_i|\bm{N}_{i,n}|^2 \\
  & + \frac{1}{\sigma_{n}^2}\Big(\frac{4}{\pi}\E[\Zbc^4]\Big)^{1/2}\Big(4\sum_i|\bm{N}_{i,n}|^3 + 3\sum_{i,j}(\bm{W}_n^3)_{ij}\Big)^{1/2}
    \end{split}
\end{equation}
\medskip
By the $c_r$-inequality,
\[
\E[|\Zbc|^3] \;\leq\; 4\big(\E[|\Zplusbc|^3]+\E[|\Zminusbc|^3]\big).
\]
where by decomposing $\Zplusbc$ 
\[
\E[|\Zplusbc|^3]
\;\leq\; 4\big(\E[|\Zplusbcone|^3]+\E[|\Zplusbctwo|^3]\big)
= O\!\Big(\tfrac{1}{n^3 h_n^{2\bar{s}}}\Big)
+ O\!\Big(\tfrac{h_n^{3(p+1)}}{n^3 b_n^{3(p+1)+2\bar{s}}}\Big),
\]
and $\E[|\Zminusbc|^3]$ has a bound of the same order.  
Similarly,
\[
\E[\Zbc^4]
= O\!\Big(\tfrac{1}{n^4 h_n^{3\bar{s}}}\Big)
+ O\!\Big(\tfrac{h_n^{4(p+1)}}{n^4 b_n^{4(p+1)+3\bar{s}}}\Big).
\]
Let $\rho_n=h_n/b_n$. Since $\sum_i|\bm N_{i,n}|^2=O(n)$ and
$\big(4\sum_i|\bm N_{i,n}|^3+3\sum_{i,j}(\bm W_n^3)_{ij}\big)^{1/2}=O(n^{1/2})$ by Assumption \ref{ass:localdependence}, the first and second terms in \eqref{eq:distbc} are
\[
O\!\Big((nh_n^{\bar{s}})^{-1/2}\min\{1,\rho_n^{-3(p+1)-\tfrac{3}{2}\bar{s}}\}\Big)
+ O\!\Big((nb_n^{\bar{s}})^{-1/2}\min\{1,\rho_n^{\,3(p+1)+\tfrac{3}{2}\bar{s}}\}\Big)
= o(1),
\]
and
\[
O_p\!\Big((nh_n^{\bar{s}})^{-1/2}\min\{1,\rho_n^{-2(p+1)-\bar{s}}\}\Big)
+ O_p\!\Big((nb_n^{\bar{s}})^{-1/2}\min\{1,\rho_n^{\,2(p+1)+\bar{s}}\}\Big)
= o(1).
\]
Hence $\xi_n \xrightarrow{d} \mathcal N(0,1)$.  
The condition $n \min\{h_n^{\bar{s}}, b_n^{\bar{s}}\} \to \infty$ combined with  Lemma~\ref{lemma:convergencematricesgamma} and Lemma~\ref{lemma:convergencematricestheta} gives
\(\tfrac{\estimatorbcapp[*]}{\sqrt{\variancebc}} = \xi_n + o_p(1)\),
so $\estimatorbcapp[*]$ (rescaled) has the same limiting distribution as $\xi_n$.  By $n \min\{h_n^{\bar{s}}, b_n^{\bar{s}}\} \to \infty$ and Lemmas~\ref{lemma:convergencematricesgamma}  \ref{lemma:convergencematricestheta} we have $T_{d,g,d'g'}(h_n) = O(h_n^{p+2})$, $h_n^{p+1}(\bias - \biasfinite{d,g,d',g'}{p}{p+1}{h_n}) = o_p(h_n^{p+1})$, $h_n^{p+1}b_n\bigbiasbc = O_p(h_n^{p+1}b_n)$ and $T^{bc}_{d,g,d',g'}(h_n, b_n) = o_p(h_n^{p+1}b_n)$. The conclusion follows from decomposition~\eqref{eq:decompositiontaubc} and $n\min\{h_n^{2p+2+\bar{s}},b_n^{2p+2+\bar{s}}\}\max\{h_n^2,b_n^{2}\} \to 0$.
\end{proof}

An estimator of the asymptotic variance of $\estimatorbcapp$ can be obtained as follows by plugging the following estimators
\begin{equation*}
\begin{split}
    \hat{\tilde{\Psi}}_{d,g,p,q}(h_n, b_n) = \Mplus\bm{W}_n\mathcal{M}_{d,g,q}(b_n)^T/n\\
    \hat{\tilde{\Psi}}_{d',g',p,q}(h_n, b_n) = \Mminus\bm{W}_n\mathcal{M}_{d',g',q}(b_n)^T/n\\
    \hat{\tilde{\Psi}}_{d,g,d',g',p,q}(h_n, b_n) = \mathcal{M}_{d,g,p}(h_n)\bm{W}_n\mathcal{M}_{d',g',q}(b_n)^T/n
\end{split}
\end{equation*}
as well as the estimators defined in \eqref{eq:varestimatorappendix} for the corresponding quantities in the expression for $\variancebc$.

\section{Estimation of Boundary Overall Direct Effects}\label{appendix:estimatoroverall}

We now provide the asymptotic theory for the estimator $\overallest$ defined in Eq.~\eqref{eq:overallest}.  
The outcome regression functions of interest are
\begin{equation*}
\muoverallplus = \E[Y_i \mid X_i = x_i], \quad x_i \ge 0,
\qquad
\muoverallminus = \E[Y_i \mid X_i = x_i], \quad x_i < 0,
\end{equation*}
with cutoff $c=0$ without loss of generality.  

Let $\overallestapp$ denote the generic $p$th-order local polynomial estimator of $\overall$. 
% \[
% \overall = \muoverallderivplus[v] - \muoverallderivminus[v],
% \]
% the difference in the $v$th derivative of the regression functions at the cutoff.  
Because this estimator can be viewed as a local polynomial estimator on a boundary with codimension $\bar{s}=1$, its asymptotic analysis follows similar steps as in Section~\ref{appendix:estimator}.  
For brevity, we only sketch the arguments.

\subsection{Notation}
We define the boundary overall direct effect of $p$th-order local polynomial RDD estimator:
\begin{align*}
    \overallestapp &=  e_{1}^T \betaoverallplus - e_{1}^T \betaoverallminus, \\   
    \betaoverallplus &= \argmin_{b \in \mathbb{R}^{p+1}}
      \sum_i \mathbbm{1}(X_i \geq 0)(Y_i - r(X_i)b)^2K_h(X_i), \\
    \betaoverallminus &= \argmin_{b \in \mathbb{R}^{p+1}}
      \sum_i \mathbbm{1}(X_i < 0)(Y_i - r(X_i)b)^2K_h(X_i),
\end{align*}
where $h_n>0$, $r_p(\cdot)$, $K_h(\cdot)$, and $e_{1}$ are defined as in Section~\ref{appendix:estimator}.  

We set $\mathbbm{1}(X_i \geq 0)=\Iplusov$ and $\mathbbm{1}(X_i<0)=\Iminusov$, $\bm{Y}=(Y_1,\dots,Y_n)^T$, and define  \begin{align*}
    \Xpov &= [r(X_1/h_n),\dots,r(X_n/h_n)]^T, \\
    S_p(h_n) &= [(X_1/h_n)^p,\dots,(X_n/h_n)^p]^T, \\
    \Wplusov &= \mathrm{diag}(\mathbbm{1}(X_1 \ge 0)K_h(X_1),\dots,\mathbbm{1}(X_n \ge 0)K_h(X_n)), \\
    \Wminusov &= \mathrm{diag}(\mathbbm{1}(X_1 < 0)K_h(X_1),\dots,\mathbbm{1}(X_n < 0)K_h(X_n)).
\end{align*}

Then set
\begin{align*}
    \Gammaplusov &= \Xpov^T \Wplusov \Xpov / n, & \tplusov &= \Xpov^T \Wplusov \bm{Y} / n, \\
    \Gammaminusov &= \Xpov^T \Wminusov \Xpov / n, & \tminusov &= \Xpov^T \Wminusov \bm{Y} / n, 
    % \thetaplusov &= \Xpov^T \Wplusov S_p(h_n) / n, \\
    % \thetaminusov &= \Xpov^T \Wminusov S_p(h_n) / n.
\end{align*}

We have 
\begin{equation*}
    \betaoverallplus = H(h_n)\Gammaplusov^{-1}\tplusov, \quad
    \betaoverallminus = H(h_n)\Gammaminusov^{-1}\tminusov.
\end{equation*}

Finally, we define the linear projection coefficients
\begin{equation}
\beta_{1,p}(h_n) = H(h_n)\bar{\Gamma}_{1,p}(h_n)\bar{t}_{1,p}(h_n), \qquad
\beta_{0,p}(h_n) = H(h_n)\bar{\Gamma}_{0,p}(h_n)\bar{t}_{0,p}(h_n)
\end{equation}
and define the centered quantities $\tplusov[*], \tminusov[*], \betaoverallplus[*], \betaoverallminus[*]$, and $\hat{\tau}^*_{1|0,p}(h_n)$ obtained by replacing $Y_i$ with $\nu_{i,d}= Y_i-r_p(X_i)\beta_{d,p}(h_n)$, $d \in \{0,1\}$.

%We also define the conditional variances $\sigmaplusov = \V[Y_i\,|\,X_i = x_i]$ for $x_i\geq 0$ and $\sigmaminusov = \V[Y_i\, |\,X_i = x_i]$ for $x_i < 0$; and the conditional covariances $\ccovplusov = \C[Y_i, Y_j\,|\, X_i = x_i, X_j = x_j]$ for $x_i, x_j \geq 0$, $\ccovminusov$ for $x_i, x_j < 0$ and  $\ccovplusminusov$ for $x_i\geq0$, $x_j < 0$. 
%Then $\Psiplusov$, $\Psiminusov$ and $\Psiplusminus$ are defined as $\Psiplus$, $\Psiminus$ and $\Psiplusminus$ in subsection \ref{subsec:notation} but replacing $\sigmaplus$, $\ccovplus$, $\sigmaminus$, $\ccovminus$, $\ccovplusminus$, $\density$ and $\jointdensity$ with $\sigmaplusov$, $\ccovplusov$, $\sigmaminusov$, $\ccovminusov$ and $\ccovplusminusov$, $f_i(uh_n)$ and $f_{ij}(uh_n, wh_n) $, where $f_i(uh_n)$ and $f_{ij}(uh_n, wh_n)$ are the marginal density of $X_i$ and the joint density of $X_i$ and $X_j$, respectively. 

\subsection{Asymptotic Theory}
Under Assumptions \ref{ass:consistency}-\ref{ass:identification} 
\[
\muoverallplus = \sum_{g \in \mathcal{G}_i} \int_{\mathcal{X}_{\smallN_i}(g)}\hspace{-0.5em}m_{1, g}(x_i, \bm x_{\smallN_i}) \cdot\frac{f(x_i, \bm{x}_{\smallN_i})}{f(x_i)}d\bm{x}_{\smallN_i}, \quad \muoverallminus = \sum_{g \in \mathcal{G}_i} \int_{\mathcal{X}_{\smallN_i}(g)}\hspace{-0.5em}m_{0, g}(x_i, \bm x_{\smallN_i}) \cdot\frac{f(x_i, \bm{x}_{\smallN_i})}{f(x_i)}d\bm{x}_{\smallN_i}
\]
are continuous in $x_i = 0$, where $\mathcal{X}_{\smallN_i}(g)$ is the set of elements $\bm{x}_{\smallN_i}$ such that $e(\bm x_{\smallN_i}) = g$. We further adopt the assumptions from Section~\ref{appendix:estimator}, replacing \ref{ass:smoothness} with:

\begin{assumption}\label{ass:smoothnessov} 
$\muoverallplus[x_i]$ and $\muoverallminus[x_i]$ are $S$-times continuously differentiable with $S \geq p+2$.
\end{assumption}

\noindent Under Assumption~\ref{ass:smoothnessov}, we obtain the decomposition 
\begin{equation}\label{eq:decompositiontauov}
    \begin{split}
        \overallestapp = & \overall + h_n^{p+1}\underbrace{\Big(
       \frac{\muoverallderivplus[p+1]}{(p+1)!}\biasplusov
      -\frac{\muoverallderivminus[p+1]}{(p+1)!}\biasminusov\Big)}_{\biasov(h_n)} + T_{1,0}(h_n)
    +  \hat{\tau}^*_{1|0,p}(h_n)
    \end{split}
\end{equation}
where $\biasplusov= e_1^T\bar{\Gamma}_{1,p}^{-1}(h_n)\bar{\theta}_{1,p,p+1}(h_n)$ and $\biasminusov= e_1^T\bar{\Gamma}_{0,p}^{-1}(h_n)\bar{\theta}_{0,p,p+1}(h_n)$, with 
\[
\bar{\theta}_{\bullet,p,q}(h_n) = \E\big[X_p(h_n)^TW_{\bullet}(h_n)\,S_q(h)/n\big], \quad S_q(h_n) = [(X_1/h_n)^q,...,(X_n/h_n)^q] 
\]
for $\bullet \in \{0,1\}$, and $T_{1,0}(h_n)$ depends on the Taylor reminders. 
% \begin{equation}\label{eq:decompositiontauov}
% \begin{split}
%     \overallestapp[*] 
%     &= (\overallest - \overall) 
%     - h_n^{p+1}\Bigg(
%        \frac{\muoverallderivplus[p+1]}{(p+1)!}\biasplusov
%       -\frac{\muoverallderivminus[p+1]}{(p+1)!}\biasminusov\Bigg) \\
%     &\quad - e_1^T h_n^{p+1}\Big(
%         \Gammaplusov^{-1}\Xpov^T\Wplusov T_1(h_n) 
%        -\Gammaminusov^{-1}\Xpov^T\Wminusov T_0(h_n)\Big).
% \end{split}
% \end{equation}

Because the estimator uses only observations with $|X_i|\leq h_n$, we have
\begin{align*}
    \E\Bigg[\frac{1}{nh_n}\sum_i \Iplusov K\!\left(\frac{X_i}{h_n}\right)
          \left(\frac{X_i}{h_n}\right)^k\Bigg]
    &= \frac{1}{n}\sum_i \int_0^1 K(u)u^k 
       \int_{\pscore} f(uh_n,\bm{x}_{\smallN_i})\,d\bm{x}_{\smallN_i}\,du \\
    &= \int_0^1 K(u)u^k f(uh_n)\,du,
\end{align*}
for nonnegative integer $k$, where $f(x_i)=f_{X_i}(x_i)$ is the marginal density of $X_i$, and analogously for $ \E\Bigg[\frac{1}{nh_n}\sum_i \Iminusov K\!\left(\frac{X_i}{h_n}\right)\Big(\tfrac{X_i}{h_n}\Big)^k\Bigg]$. Moreover, by similar arguments to Lemma~\ref{lemma:convergencematricesgamma}, one obtains 
\[
\V\!\left[\frac{1}{nh_n}\sum_i I_{i,\bullet}K\!\Big(\tfrac{X_i}{h_n}\Big)\Big(\tfrac{X_i}{h_n}\Big)^k\right] 
= O\!\Big(\tfrac{1}{nh_n}\Big).
\]
for $\bullet \in\{0,1\}$, from which for $nh_n \to \infty$ and $h_n \to 0$, $\Gamma_{\bullet, p}(h_n) = \limdensityov\,\Gamma_p^{1} + o_p(1)$ and 

\[
t_{\bullet, p}(h_n) =  \theta^1_{p,0} \cdot \sum_{g \in \mathcal{G}_i} \int_{\mathcal{X}_{\smallN_i}(g)}\hspace{-0.5em}m_{\bullet, g}(x_i, \bm x_{\smallN_i}) f(x_i, \bm{x}_{\smallN_i})d\bm{x}_{\smallN_i}+ o_p(1),
\]
with
\[
\Gamma_p^{1} = \int_0^1 K(u)r_p(u)\,du,
\qquad
\theta_{p,q}^{1} = \int_0^1 K(u)u^{p+q}\,du,
\]
recalling the notation in Subsection \ref{subsec:notation}. Additionally, similarly to \ref{lemma:convergencematricestheta} $    \bar{\theta}_{\bullet,p,q}  = f(0)\theta_{p,q}^{1} + o(1)$.

Finally, $nh_n\V\!\big[t_{1,0,p}^*(h_n)\big]
= \big(\limvarplusov + \limvarminusov\big)\Psi_p^1 + o(1)$
where for $\bullet\in \{0,1\}$
\[
\bar{\omega}_{\bullet}(0) = \sum_{g \in \mathcal{G}_i}\int_{\mathcal{X}_{\smallN_i}(g)}\big(\sigma_{\bullet,g}(0, \bm{x}_{\smallN_i}) + (m_{\bullet,g}(0, \bm x_{\smallN_i}) - \tilde{\mu}_{\bullet}(0))^2\big) f(0, \bm{x}_{\smallN_i})d\bm{x}_{\smallN_i}
\]

\begin{theorem}\label{th:asynormaltauov}
Suppose Assumptions~\ref{ass:consistency}--\ref{ass:localdependence},
\ref{ass:regularity}, \ref{ass:commonpieces}, and~\ref{ass:kernel} hold (with Assumption~\ref{ass:smoothness} replaced by Assumption~\ref{ass:smoothnessov}, $S \geq p+2$).  
If $nh_n \to \infty$, $h_n \to 0$, and $h_n = O(n^{-1/(2p+3)})$, then
\[
\sqrt{nh_n}
\frac{\Big(\overallestapp - \overall - h_n^{p+1}\biasov(h_n)\Big)}{\sqrt{V_{1,0,p}(h_n)}}
\xrightarrow{d} 
\mathcal{N}(0,1),
\]
where 
\[
\biasov(h_n) = \Big(\frac{\muoverallderivplus[p+1]-\muoverallderivminus[p+1]}{(p+1)!}\Big)e_1^T(\Gamma_p^{1})^{-1}\theta_{p,p+1}^{1} + o(1), 
\quad
V_{1,0,p}(h_n) =\; \frac{\limvarplusov + \limvarminusov}{\limdensityov^2}e_1^T(\Gamma_p^{1})^{-1}\Psi_p^{1}(\Gamma_p^{1})^{-1}e_1 + o(1)
\]
\end{theorem}

\begin{proof}
The proof parallels Theorem~\ref{th:asynormaltau}.  
Define
\[
\Zplusov 
=  e_1^T\bar{\Gamma}_{1,p}^{-1}(h_n)I_{1,i}
K\!\Big(\tfrac{X_i}{h_n}\Big) r_p\!\Big(\tfrac{X_i}{h_n}\Big)\nu_{i,1}/n,
\quad
\Zminusov 
=  e_1^T\bar{\Gamma}_{0,p}^{-1}(h_n)
I_{0,i}K\!\Big(\tfrac{X_i}{h_n}\Big) r_p\!\Big(\tfrac{X_i}{h_n}\Big)\nu_{i,0}/n,
\]
and set $\Zov = \Zplusov - \Zminusov$.  

Then, $nh_n\V\!\big[\sum_i \Zov\big] = V_{1,0,p}(h_n) = (\limvarplusov+\limvarminusov)\Psi_p^{1}/\limdensityov^2 + o(1)$.  Denote $\sigma_n^2 = V_{1,0,p}(h_n)/nh_n$ and $\xi_n = \sum_i \Zov/\sigma_n$.  
By Assumption~\ref{ass:localdependence} and applying Stein’s method with the bounds of \citet[Theorem~A.4]{leung20}, one obtains
$
\Delta(\xi_n,\mathcal{N}(0,1)) = O\big((nh_n)^{-1}\big) \to 0.
$
Thus $\xi_n \xrightarrow{d} \mathcal{N}(0,1)$.  

Since $\sqrt{nh_n}\tfrac{\overallestapp^*}{\sqrt{V_{1,0,p}(h_n)}} = \xi_n + o_p(1)$, the decomposition \eqref{eq:decompositiontauov} and convergence of $\bar{\Gamma}_{d,p}(h_n)$ and $\bar{\theta}_{d,p,p+1}(h_n)$, for $d \in \{0,1\}$ to $f(0)\Gamma_p^1$ and $f(0)\theta^{1}_{p, p+1}$ gives the conclusion.
\end{proof}

\subsection{Variance Estimation and Bias Correction}

Define
\begin{equation}
\begin{split}
    \mathcal{M}_{1,p}(h_n)^T 
    &= \Big[\Iplusov[1]\Kh[1]\rr[1]\hat{\xi}_{1,1}\;\cdots\; \Iplusov[n]\Kh[n]\rr[n]\hat{\xi}_{n,1}\Big], \\
    \mathcal{M}_{0,p}(h_n)^T 
    &= \Big[\Iminusov[1]\Kh[1]\rr[1]\hat{\xi}_{1,0}\;\cdots\; \Iminusov[n]\Kh[n]\rr[n]\hat{\xi}_{n,0}\Big],
\end{split}
\end{equation}
where $\hat{\xi}_{i,1}$ and $\hat{\xi}_{i,0}$ are the regression residuals to the right and left of the cutoff, respectively.  

An estimator of the asymptotic variance $\overallestapp$ denoted by $\varianceov$ is
\begin{equation}\label{eq:varestimatorov}
    \hat{\mathcal{V}}_{1,0,p}(h_n) 
    = \frac{1}{n}\, e_1^T\Big(\hat{V}_{1,p}(h_n) 
      + \hat{V}_{0,p}(h_n) 
      - 2\hat{V}_{1,0,p}(h_n)\Big)e_1,
\end{equation}
with
\begin{equation}
\begin{split}
    \hat{V}_{1,p}(h_n) 
    &= \Gammaplusov[-1]\hat{\tilde{\Psi}}_{1,p}(h_n)\Gammaplusov[-1], \\
    \hat{V}_{0,p}(h_n) 
    &= \Gammaminusov[-1]\hat{\tilde{\Psi}}_{0,p}(h_n)\Gammaminusov[-1], \\
    \hat{V}_{1,0,p}(h_n) 
    &= \Gammaplusov[-1]\hat{\tilde{\Psi}}_{1,0,p}(h_n)\Gammaminusov[-1],
\end{split}
\end{equation}
where
\begin{equation}
\begin{split}
    \hat{\tilde{\Psi}}_{1,p}(h_n) 
    &= \mathcal{M}_{1,p}(h_n)\bm{W}_n\mathcal{M}_{1,p}(h_n)^T/n, \\
    \hat{\tilde{\Psi}}_{0,p}(h_n) 
    &= \mathcal{M}_{0,p}(h_n)\bm{W}_n\mathcal{M}_{0,p}(h_n)^T/n, \\
    \hat{\tilde{\Psi}}_{1,0,p}(h_n) 
    &= \mathcal{M}_{1,p}(h_n)\bm{W}_n\mathcal{M}_{0,p}(h_n)^T/n.
\end{split}
\end{equation}

\noindent Finally, we give the expression for the bias-corrected estimator of $\overallapp$:
\begin{equation*}
    \overallestbcapp = \overallestapp - \biasbcappov
\end{equation*}
where $\biasbcappov$ uses $e_{p+1}^T\betaplusbcov$ and $e_{p+1}^T\betaminusbcov$, where $\betaplusbcov$ and $\betaminusbcov$ are the $(p+1)$-order local polynomial estimators to the right amd to the left of the cutoff with bandwidth $b_n$.
%Then the analysis of the estimator can be carried using similar arguments as in section \ref{appendix:estimator}, \emph{mutatis mutandis}.

\section{Proof of Results in Online Appendix}\label{appendix:online}

\subsection{Heterogeneous Effects}\label{appendix:heterogeneous}

In this section, we show the convergence properties allowing for heterogeneous interference sets, effective treatment boundaries and outcome and score distributions. Hence, notable quantities including, $|\mathcal{S}_{i,n}|$ and $\bar{\mathcal{X}}_{i\mathcal{S}_{i,n}}(d,g,\,|\,d,g')$ are i-specific and indexed by $n$ through their dependence on the network. 

Let
\[f_{i,n,d,g,d',g'}(0) = \int_{\bar{\mathcal{X}}_{i\mathcal{S}_{i,n}}(d,g,\,|\,d,g')} f_i\ppointhet d\mathcal{H}^{|\mathcal{S}_i| + 1 - \bar{s}}
\]
be the boundary density, and denote for short $m_{i,n,\bullet}(0) = \E_i[Y_i(\bullet)\,|\,(X_i, \bm X_{\smallN_{i,n}}) \in \bar{\mathcal{X}}_{i\mathcal{S}_{i,n}}(d,g,\,|\,d,g') ]$  for $\bullet \in \{(d,g), (d',g')\}$. We require the following assumptions to establish convergence of the estimator under heterogeneity.

\begin{assumption}\label{ass:boundaryhet}
The interference sets satisfy $\sup_{i,n}|\mathcal{S}_{i,n}| < \infty$. Moreover, for some integer $\bar{n}$, $\bar{s}_{n} = \bar{s}$ for $n \ge \bar n$, where $\bar{s}_{n} = \inf_{i} \bar{s}_{i,n}$.
\end{assumption}

\begin{assumption}\label{ass:regularityhet}
For some $\kappa >0$ the following holds for $\ppoint \in \mathcal{B}_{\kappa}(\bar{\mathcal{X}}_{i\mathcal{S}_{i,n}}(d,g,\,|\,d,g'))$:

\begin{enumerate}[label= \alph*), ref={\theassumption.\alph*}]
    % \item $\CE{Y_i^4}{ X_i = x_i, \bm X_{\smallN_i} = \bm{x}_{\smallN_{i,n}}}$ is bounded uniformly over $i$ and $n$.\label{ass:fourthmomenthet}
    \item $f_i\ppointhet$ is bounded away from zero and continuous (and thus uniformly continuous) with  common modulus of continuity over $i$ and $n$. Moreover, as $n \to \infty$
    \begin{equation*}
    \frac{1}{n}\sum_{i:\bar{s}_i = \bar s}f_{i,n,d,g,d',g'}(0) \to \limdensitys[\bar s].
    \end{equation*}\label{ass:densitieshet}
         \vspace{-1em}

    \item $\V_i\!\big[Y_i(d,g)\mid X_i=x_i,\bm X_{\smallN_{i,n}}=\bm x_{\smallN_{i,n}}\big]$ and 
    $\V_i\!\big[Y_i(d',g')\mid X_i=x_i,\bm X_{\smallN_{i,n}}=\bm x_{\smallN_{i,n}}\big]$ 
    are uniformly bounded and bounded away from zero over $i,n$. \label{ass:varianceshet}
  
    \item $m_{i,d,g}\ppointhet$ and $m_{i,d'g'}\ppointhet$ are continuous (and thus uniformly continuous) with common modulus of continuity over $i$ and $n$. Moreover, as $n \to \infty$
    \[
    \frac{1}{n}\sum_{i:\bar{s}_i = \bar s}m_{i,\bullet}(0) \to \bar{m}^{\bar{s}}_{\bullet}(0).
    \]\label{ass:smoothnesshet} 
\end{enumerate}
\end{assumption}

\vspace{-2em}
\begin{theorem}\label{th:heterogeneousconvergence}
Suppose Assumptions~\ref{ass:consistency}--\ref{ass:indrule}, 
\ref{ass:dependencyneighborhood}--\ref{ass:localdependence}, 
\ref{ass:kernel}, and\ref{ass:boundaryhet}~\ref{ass:regularityhet} hold. 
If $n h_n^{\bar s}\to\infty$ and $h_n\to 0$, then
\[
\estimator
\;\xrightarrow{p}\;
\frac{\bar m_{d,g}^{\bar s}(0)-\bar m_{d',g'}^{\bar s}(0)}{\bar f_{d,g,d',g'}^{\bar s}(0)}.
\]
\end{theorem}

\begin{proof}
\noindent\textbf{Expectation of $\Gammaplus$.}
For $n\ge \bar n$,
\begin{equation*}
\begin{split}
&= \frac{1}{nh_n^{\bar s}} \sum_{i \in V_{g}} \sum_{\curve[i,n]}  h_n^{s_{\curve[i,n]} - \bar s}\int_{\mathcal{R}_{\curve[i,n]}}\int_{N^{s_{\curve[i,n]}}}
   K(\|\bm u\|)r_p(\|\bm u\|)r_p(\|\bm u\|)^T f(h_n\bm u,\bm x_{\findex})\,
   d\bm u\, d\bm x_{\findex}
   + \frac{1}{nh_n^{\bar{s}}}I_{ih_n}
\end{split}
\end{equation*}
where we recall $V_g$ is the set of units for which $g$ is achievable. For brevity, we will just use the subscript $i$ in summation and leave the belonging in this set implicit.

Partition the sample into $i\in \mathcal I_{\bar s}:=\{i:\bar s_{i,n} = \bar s\}$ and $i\in \mathcal I_{>\bar{s}} :=\{i:\bar s_{i,n}>\bar s\}$. 
\begin{equation*}
\begin{split}
\E[\Gammaplus]
& = \frac{1}{n}\sum_{\mathcal{I}_{\bar{s}}}  \sum_{\curve[i,n]}  h_n^{s_{\curve[i,n]} - \bar s}\int_{\mathcal{R}_{\curve[i,n]}}\int_{N^{s_{\curve[i,n]}}}
   K(\|\bm u\|)r_p(\|\bm u\|)r_p(\|\bm u\|)^T f(\bm u h_n,\bm x_{\findex})\,
   d\bm u\, d\bm x_{\findex} + \frac{1}{n h_n^{\bar{s}}}I_{ih_n} \\
& + \frac{1}{n}\sum_{\mathcal{I}_{>\bar{s}}}  \sum_{\curve[i,n]}  h_n^{s_{\curve[i,n]} - \bar s}\int_{\mathcal{R}_{\curve[i,n]}}\int_{N^{s_{\curve[i,n]}}}   K(\|\bm u\|)r_p(\|\bm u\|)r_p(\|\bm u\|)^T f(\bm u h_n,\bm x_{\findex})\,
   d\bm u\, d\bm x_{\findex} + \frac{1}{n h_n^{\bar{s}}}I_{ih_n}   
\end{split}
\end{equation*}
The terms in the summation over $\mathcal I_{>\bar{s}}$ are $O(h_n)$ by Assumption \ref{ass:densitieshet}, \ref{ass:kernel}, and
because $h_n^{s_{\curve[i,n]}-\bar s}=O(h_n)$ and $\sum_{\curve[i,n]}\operatorname{Vol}(\mathcal R_{\curve[i,n]})$ is uniformly bounded
(Assumption~\ref{ass:boundaryhet}). Hence, it suffices to study the first summation over $\mathcal{I}_{\bar{s}}$. By an analogous decomposition as in Lemma \ref{lemma:convergencematricesgamma}
\begin{equation*}
\begin{split}
\frac{1}{n}\sum_{\mathcal{I}_{\bar{s}}}  \sum_{\curve[i,n] : s_{\curve[i,n] = \bar{s}}} \int_{\mathcal{R}_{\curve[i,n]}}\int_{N^{\bar s}}
   K(\|\bm u\|)r_p(\|\bm u\|)r_p(\|\bm u\|)^T f(\bm u h_n,\bm x_{\findex})\,
   d\bm u\, d\bm x_{\findex} + \frac{1}{n h_n^{\bar s}}I_{ih_n} + I(s_{\curve[i,n]} > \bar s)
\end{split}
\end{equation*}
where $I(s_{\curve[i,n]}>\bar s)$ collects terms depending on higher-codimension pieces, each $O(h_n)$ uniformly in $i$ and $n$.

By Assumption~\ref{ass:densitieshet}, there exists a common modulus of continuity $\omega : [0, \infty] \to [0,\infty]$ such that, uniformly over $i$, over pieces $\curve$ and over $\bm x_{\mathcal{R}_{\curve[i,n]}}$, 
\[
\big| f_i(h_n \bm u,\bm x_{\mathcal{R}_{\curve[i,n]}}) - f_i(\bm 0,\bm x_{\mathcal{R}_{\curve[i,n]}}) \big| \le \omega(\, h_n \|\bm u\|\,).
\]
Hence,
\[
\begin{aligned}
&
\frac{1}{n}\sum_{\mathcal{I}_{\bar{s}}}  \sum_{\curve[i,n] : s_{\curve[i,n]} = \bar{s}} \int_{\mathcal{R}_{\curve[i,n]}}\int_{N^{\bar s}}
K(\|\bm u\|)\,r_p(\|\bm u\|)r_p(\|\bm u\|)^T\,\big| f_i(h_n \bm u,\bm x_{\mathcal{R}_{\curve[i,n]}}) - f_i(\bm 0,\bm x_{\mathcal{R}_{\curve[i,n]}}) \big|\,
d\bm u\, d\bm x_{\mathcal{R}_{\curve[i,n]}} \\
&\qquad \le\;
\frac{\omega(\, h_n \|\bm u\|\,)}{n}\sum_{\mathcal{I}_{\bar{s}}} \operatorname{Vol}(\bar{\mathcal{X}}_{i\smallN_{i,n}}(d,g\,|\,d',g'))
\int_{\unitdisc[\bar s]} K(\|\bm u\|)\,\|\bm u\|^{k}\, d\bm u \;\to\;0,
\end{aligned}
\]
as $n \to \infty$ and $h_n \to 0$ since $\operatorname{Vol}(\bar{\mathcal{X}}_{i\smallN_{i,n}}(d,g\,|\,d',g')) = \sum_{\curve[i,n] : s_{\curve[i,n]} = \bar{s}}
\operatorname{Vol}(\mathcal{R}_{\curve[i,n]})$ is bounded uniformly over $i,n$ by Assumption \ref{ass:boundaryhet}. 
Moreover,
\[
\frac{1}{n}\sum_{\mathcal{I}_{\bar{s}}}  \sum_{\curve[i,n] : s_{\curve[i,n]} = \bar{s}} \int_{\mathcal{R}_{\curve[i,n]}} f(\bm 0,\bm x_{\mathcal{R}_{\curve[i,n]}})\, d\bm x_{\findex}
\;\longrightarrow\; \limdensitys[\bar{s}]
\quad\text{by Assumption \ref{ass:densitieshet}.}
\]
Therefore,
\begin{align*}
\frac{1}{n}\sum_{\mathcal{I}_{\bar{s}}}  \sum_{\curve[i,n] : s_{\curve[i,n]} = \bar{s}} \int_{\mathcal{R}_{\curve[i,n]}}&\int_{N^{\bar s}}
K(\|\bm u\|)\,r_p(\|\bm u\|)r_p(\|\bm u\|)^T\, f_i(h_n \bm u,\bm x_{\mathcal{R}_{\curve[i,n]}})\,
d\bm u\, d\bm x_{\mathcal{R}_{\curve[i,n]}}\\
\quad \;\rightarrow\;
&\limdensitys[\bar{s}] \int_{\unitdisc[\bar{s}]} K(\|\bm u\|)\,\|\bm u\|^k\, d\bm u.
\end{align*}
Hence, $\E[\Gammaplus]  = \limdensitys[\bar s] \Gamma_p^{\bar{s}} + o(1)$.

\medskip
\noindent\textbf{Expectation of $\tplus$}. We expand $\E[\tplus]$
\[
=\frac{1}{nh_n^{\bar s}} \sum_{i \in V_{g}} \sum_{\curve[i,n]}  h_n^{s_{\curve[i,n]} - \bar s}\int_{\mathcal{R}_{\curve[i,n]}}\int_{N^{s_{\curve[i,n]}}}
   K(\|\bm u\|)r_p(\|\bm u\|) m_{d,g}(h_n\bm u,\bm x_{\findex}) f(h_n\bm u,\bm x_{\findex})\,
   d\bm u\, d\bm x_{\findex}
   + \frac{1}{nh_n^{\bar{s}}}I_{ih_n}
\]
Dividing and multiplying by $f_{i,n,d,g,d',g'}(0)$, which is positive by Assumption~\ref{ass:densitieshet},  and using  common modulus of continuity of $m_{i,d,g}\ppointhet$ and $f_i\ppointhet$ yields
\begin{equation*}
\begin{split}
\E[\tplus]  
 \to & \quad \theta_{p,0}^{\bar{s}} \cdot \bar{m}^{\bar{s}}_{d,g}(0)
 \end{split}
\end{equation*}

\medskip
\noindent\textbf{Convergence in probability}
Under Assumptions~\ref{ass:dependencyneighborhood}--\ref{ass:localdependence}
and bounded conditional variances (Assumption~\ref{ass:varianceshet}) the element-wise variance of $\Gammaplus$ and $\tplus$ is $O((nh_n^{\bar{s}})^{-1})$ by analgous arguments as in Lemma \ref{lemma:convergencematricesgamma}) and \ref{lemma:convergencematricest} 
\[
\Gamma_{d,g,p}(h_n)
\;=\;
\limdensitys[\bar s] \Gamma_p^{\bar{s}}\;+\; o_p(1),
\qquad
\tplus
\;=\;
\theta^{\bar s}_{p,0}
\;+\; o_p(1),
\]
\medskip
\noindent\textbf{Limit of the estimator.}
By continuous mapping and the identity
$e_1^\top(\Gamma_p^{\bar s})^{-1}\theta_{p,0}^{\bar s}=1$,
\[
e_1^T\hat{\beta}_{d,g,p}(h_n) =  e_1^\top\Gamma_{d,g,p}(h_n)^{-1} \tplus 
\;\stackrel{p}{\longrightarrow}\;
\frac{\bar{m}_{d,g}^{\bar{s}}(0)}{\bar{f}_{d,g,d',g'}(0)}\]

Repeating the argument for $(d',g')$ and taking the difference gives the stated probability limit for $\hat{\tau}_{d,g,d',g',p}(h_n)$.
\end{proof}

\end{document}
