# Supplementary material for: Regression Discontinuity Designs Under Interference
Source: arXiv:2410.02727 source file (2026-09-09)
Supplement: Supplementary file 2 [file onlineappendix.tex]

\documentclass[main.tex]{subfiles}
\myexternaldocument{main}

% \ifcsname preamble@file\endcsname
%   \externaldocument[main-]{main}
%   \setcounter{page}{\getpagerefnumber{main-sec:conclusion}}
% \fi

\begin{document}
\emptythanks
\title{Supplemental Appendix to \qq Regression Discontinuity Designs Under Interference"}

\date{}
\maketitle

\begin{appendices}
\numberwithin{table}{section}
\numberwithin{theorem}{section}
\numberwithin{equation}{section}
\setcounter{page}{1}

\section{Heterogeneous Effects}\label{onlineappendix:irregular}
We extend the analysis to scenarios where units can have heterogeneous cardinality of the interference sets and, thus, heterogeneous effective treatment boundaries, as well as  heterogeneous outcome and score distributions. In general, both outcomes and score distributions can depend on network characteristics,such as the number of neighbors,  and other fixed covariates,  \citep[e.g.][]{ogburn22}. In addition, the dimension of the multiscore space, and the geometry of the effective treatment boundaries may vary across units. When such heterogeneity arise, boundary causal effects must be defined as finite ample averages of the outcome expectations across the network nodes:
% Let $\mathcal{N}_s = \{i \in \mathcal{N}\, : \, |\mathcal{S}_i| = s\}$ be the set of all units having exactly $s$ neighbors. We redefine the boundary point causal effects as 
% \begin{equation}\label{def:boundpointhet}
%     \tau_{s,d,g|d',g'}(\bar{x}_i, \bar{\bm{x}}_{\smallN_i}) = \frac{1}{|\mathcal{N}_s|}\sum\limits_{i \in \mathcal{N}_s}\E_i[Y_i(d,g) - Y_i(d',g')\,|\,(X_i, \pscore) = (\bar{x}_i, \bar{\bm{x}}_{\smallN_i})]
% \end{equation}
% %
% The definition of $\mathcal{N}_s$ is necessary with unequally-sized interference, as boundary point effects are dimension-specific: by conditioning on $(X_i, \pscore)$, they also condition on the dimension of the interference set (and the multiscore space).
%We define boundary causal effects as follows:
%can be defined for the entire sample as follows  
\begin{equation}\label{def:boundhet}
    \boundeff = \frac{1}{|V_g|}\sum_{i \in V_g}\tau_{i,d,g|d',g'}(\Frontier)
    %tau_{d,g,d',g'}(\Frontier)
\end{equation}
where $\tau_{i,d,g|d',g'}(\Frontier) = \E_i[Y_i(d,g) - Y_i(d',g')\,|(X_i , \pscore) \in \Frontier]$ is the $i-$specific boundary causal effect, and $V_g = \{i \in \mathcal{N} : g \in \mathcal{G}_i\}$ the set of units whose neighborhood treatment $G_i$ can attain the value $g$, and for which then potential outcomes $Y_i(d,g)$ are well-defined. Here, the effective treatment boundary has potentially different dimension and codimension for each $i$,  given by $|\mathcal{S}_i| + 1 - \bar{s}_i$ and $\bar{s}_i$.

% \tau_{i,d,g,d',g'}(\Frontier)= \E_i[Y_i(d,g) - Y_i(d',g')\,|(X_i , \pscore) \in \Frontier]$ is the unit-specific expected difference in potential outcomes at their effective treatment boundary, which have potentially different dimensions.

%the average of unit-specific boundary overall direct effects.

Identification of boundary average causal effects is achieved under Assumptions \ref{ass:consistency}-\ref{ass:identification} as
%Identification of the boundary point and boundary average causal effects is achieved under Assumption \ref{ass:identification}, as well as Assumptions \ref{ass:consistency}-\ref{eq:indrule}.
% %
% \begin{equation*}
% \begin{split}
% \tau_{s,d,g|d',g'}(\bar{x}_i, \bar{\bm{x}}_{\smallN_i}) = \frac{1}{|\mathcal{N}_s|}\sum\limits_{i \in \mathcal{N}_s} &\lim\limits_{\varepsilon \to0} \E_{i}[Y_i \,|\,(X_i,\pscore) \in \eballright] \\
% - & \lim_{\varepsilon \to 0}\E_{i}[Y_i \,|\, (X_i, \pscore) \in \eballleft]
% \end{split}
% \end{equation*}
%and 
\begin{equation*}
\begin{split}
\boundeff = \frac{1}{|V_g|}\sum_{i \in V_g} &\lim\limits_{\varepsilon \to0} \E_i[Y_i \,|\,(X_i,\pscore) \in \eballboundright] \\
-& \lim_{\varepsilon \to 0}\E_i[Y_i \,|\, (X_i, \pscore) \in \eballboundleft]  \\
\end{split}
\end{equation*}
by analogous arguments as in Theorem \ref{th:cont}. 

Under such heterogeneity, the estimator $\estimator$ defined in Section~\ref{sec:estimation} is, in general, no longer consistent to \eqref{def:boundhet}. Instead, it converges to a weighted average of unit-specific boundary causal effects. Moreover, when the codimension of the effective treatment boundary $\bar{s}_i$ is heterogeneous, 
%the estimator converges to a weighted average of boundary effects for units whose boundary has the lowest codimension in the network. Indeed, 
assuming that for $n$ large enough $\inf_i \bar{s}_i = \bar{s}$, independent of $n$, only observations with $\bar{s}_i=\bar{s}$ contribute in the limit, because the number of observations within distance $h_n$ of $\Frontier_i$ scales as $n h_n^{\bar{s}_i}$. Hence, the contribution of higher-codimension observations ($\bar{s}_i>\bar{s}$) vanishes, and the estimator converges to a weighted average of boundary effects for units whose boundary has the lowest codimension in the network.

% In section \ref{sec:estimation}, we derived the analytical properties of the estimators for $\estimator$ and $\hat{\tau}_{1|0}(h_n)$, assuming homogeneity of the target outcome regression functions. However, if these functions differ across units, our estimation strategy no longer estimates the estimands defined in \eqref{def:boundhet} and \eqref{def:overallhet}. Instead, it consistently estimates the limit of a weighted average of unit-specific effects.

% Moreover, since the codimension $\bar{s_i}$ is heterogeneous, the distance-based estimator converges to the weighted average of boundary effects for those units that whose boundary achieves the lowest codimension.

% and consider the observed outcome 
%  \begin{equation*}
%      Y_i = \tilde{\mu}_i(X_i) + \varepsilon_i
%  \end{equation*}
%  %
% where $\tilde{\mu}_i(X_i)$ is now $i$-specific. Suppose further that the boundary overall direct effect $\tau_{1|0}$ defined in \eqref{def:overallhet} has a finite limit as $n$ becomes large. The cutoff is $c = 0$. 
Formally, in Theorem \ref{th:heterogeneousconvergence} we show that under similar assumptions to Theorem \ref{th:asynormal}:
\begin{equation}\label{eq:weigthed}
    \estimator \overset{p}\to \frac{\sum_{i:\,\bar s_i=\bar s} \tau_{i,d,g|d',g'}(\Frontier) \, f_{i,d,g,d',g'}(0)}
     {\sum_{i:\,\bar s_i=\bar s}f_{i,d,g,d',g'}(0)}
\end{equation}
as $nh_n^{\bar{s}}\to\infty$ and $h_n \to 0$, where the summation is implicitly taken over units in the feasibility set $V_g$, and  
$$f_{i,d,g,d',g'}(0) = \int\limits_{\Frontier} f_i\ppoint d\mathcal{H}^{|\mathcal{S}_i| + 1 - \bar{s}} $$
%where $\tilde{\mu}_{i,1}(0) = \lim\limits_{x_i \downarrow0}\tilde{\mu}_i(x_i)$, $\tilde{\mu}_{i,0}(0) = \lim\limits_{x_i \uparrow0}\tilde{\mu}_i(x_i)$. Under Assumption \ref{ass:identification} the RHS of \eqref{eq:weigthed} corresponds to the weighted average of unit-specific overall direct effects, weighted by individual score densities at the cutoff. 
The RHS of \eqref{eq:weigthed} corresponds to the weighted average of unit-specific boundary effects, with weights depending on the integrals of the score densities at the effective treatment boundary. 

Depending  on the source of heterogeneity, we distinguish two notable cases:
\begin{enumerate}
    \item Homogeneous $|\mathcal{S}_i|$ and $\Frontier$, and heterogeneous $\E_{i}[Y_i(d,g) |X_i = x_i, \pscore= \bm x_{\smallN_i}]$ and $f_i \ppoint$: the estimator converges to the weighted average in \eqref{eq:weigthed} but defined for the entire network. If, in addition, the score distributions are homogeneous, then $\estimator$ converges to the network average defined in \eqref{def:boundhet}.
    \item Heterogeneous $|\mathcal{S}_i|$ and $\Frontier$, and homogeneous $\E[Y_i(d,g)\mid X_i = x_i, \pscore = \bm{x}_{\smallN_i}]$: when $\tau_{i,d,g|d',g'}\ppoint = \kappa$ is constant across all $i$, $x_i$, and $\bm{x}_{\smallN_i}$, the estimator converges to the network average in \eqref{def:boundhet}, equal to $\kappa$, regardless of the score density. This corresponds to a limiting case where causal effects are invariant to individual and neighborhood scores, and network characteristics, which we view as an unlikely scenario in practice.
    %Heterogeneous $|\mathcal{S}_i|$ and $\Frontier$, and homogeneous $\E[Y_i(d,g) |X_i = x_i, \pscore= \bm x_{\smallN_i}]$: $\tau_{i,d,g|d',g'}(\Frontier) = \kappa$ is constant for all $i$, $x_i$, $\bm{x}_{\smallN_i}$, and the estimator converges to the network average defined in \eqref{def:boundhet}, which is equal $\kappa$, regardless of the score density. This is the case where the causal effects do not depend on the individual and neighborhood values and the network. We view this case as a limiting case that will not hold often in practice.
\end{enumerate}

Finally, we note that one method to recover the estimand \eqref{def:boundhet} under heterogeneous $|\mathcal{S}_i|$ is to estimate boundary effects separately via distance-based local linear estimation for units with the same interference set cardinality, and then average the estimated effects across the sample units. However, this procedure may yield high variance, as it aggregates potentially noisy estimates. 

%we note that boundary causal effects are aggregate effects and therefore might be homogeneous across units with different interference sets. In that case, $\estimator$ converges to the homogeneous boundary effect. Such homogeneity is plausible, for instance, if units have interference sets with similar cardinality. When interference sets' sizes vary widely, a practical approach is to restrict estimation to strata with similar neighborhood sizes, as in Section~\ref{sec:empirical}. 

\section{Additional Estimations Results}

\subsection{MSE-optimal Bandwidth, Bias Correction and Robust Confidence Intervals}
\label{sec:biascorrection}

As remarked in Section \ref{sec:estimation}, the proposed estimator requires selecting a bandwidth $h_n$. The standard approach in RDDs for bandwidth selection minimizes the asymptotic Mean Squared Error (MSE) \citep{imbenskalyanaraman12}. In our setting, the MSE-optimal bandwidth is easily derived based on Theorem \ref{th:asynormal}:
 \begin{equation}
     h_{n}^{opt} = \left(\frac{\bar{s}V}{4B^2}\right)^{\frac{1}{\bar s + 4}} n^{-\frac{1}{\bar s + 4}}
\end{equation}
where
\[
B = \Big(\frac{\muplusderiv[2]-\muminusderiv[2]}{2!}\Big)e_1^\top (\Gamma^{\bar{s}})^{-1}\theta^{\bar{s}},
\quad
V = \Big(\frac{\omegaplus + \omegaminus}{\limdensity}\Big)e_1^\top (\Gamma^{\bar{s}})^{-1}\Psi^{\bar{s}}(\Gamma^{\bar{s}})^{-1} e_1.
\]
The optimal bandwidth can be estimated using the plug-in selection procedure proposed by \citet{cct14}, which employs preliminary estimates of bias and variance with pilot bandwidths, or using plug-in estimators of the unknown quantities entering the asymptotic bias and variance \citep{imbenskalyanaraman12}.

In principle, as discussed in Section \ref{subsec:asy}, the contribution of the asymptotic bias of our RDD estimator, shown in Theorem \ref{th:asynormal}, would go to zero if the condition $nh_n^{\bar{s} + 4} \to 0$ is met \citep{fan}. However, the MSE-optimal bandwidth does not meet this requirement, analogously to no-interference RDDs \citep{cct14}. In RDD applications, bias-corrected estimators are then commonly employed.
The standard method proposed by \citet{cct14} recenters the RDD estimator by subtracting an estimate of the leading bias and rescales it with a variance estimator that accounts for the additional variability introduced by the bias-correction term. This approach yields confidence intervals that are robust to large bandwidths. We also consider bias correction in our setting.
Following \citet{cct14}, an estimator of the term ${B}_{d,g,d',g'}(h_n)$ in Theorem~\ref{th:asynormal} can be obtained by using the local-quadratic estimators of the second derivatives $\frac{\muplusderiv[(2)]}{2!}$ and $\frac{\muminusderiv[(2)]}{2!}$ with bandwidth $b_n$. Let us denote this estimator as $\hat{{B}}_{d,g,d',g'}(h_n, b_n)$.
The bias-corrected estimator of $\tau_{d,g|d',g'}(0)$ is given by 
\begin{equation}\label{eq:estimatorbc}
 \estimatorbc = \estimator - \hat{{B}}_{d,g,d',g'}(h_n, b_n) 
\end{equation}
The estimator $\estimatorbc$ is asymptotically normal with zero mean and asymptotic variance coincident with the independent data case under a similar asymptotic regime to \citet{cct14}, (Theorem \ref{th:asybiascorretiontau}, Supplementary Material \ref{appendix:estimator}). This is unsurprising given that $\estimatorbc$ differs from $\estimator$ by a term depending on local quadratic estimators, to which all previous considerations, \emph{mutatis mutandis}, apply. 
Finally, the variance of $\estimatorbc$ can be estimated similarly as for $\estimator$, but with an extension to incorporate the additional variability induced by the bias correction term (see Supplementary Material \ref{appendix3:biascorrection} for details).

\subsection{Estimation of Boundary Overall Direct Effects}\label{subsec:overallestapp}

The boundary overall direct effect $\overall$ is identified as the difference between the right and left limit of the observed outcome regression functions conditional on the individual score $X_i$ as $X_i$ approaches the cutoff under continuity assumptions (Theorem \ref{th:overall}). 
Letting $\muoverall = \CE{Y_i}{X_i}$, Theorem \ref{th:overall} yields $\overall = \lim_{x_i \downarrow 0}\muoverall[x_i] - \lim_{x_i \uparrow 0}\muoverall[x_i]$, with $c = 0$.
A natural choice is then to estimate the limits $\muoverallplus[0] = \lim\limits_{x_i\downarrow 0}\muoverall[x_i]$ and $\muoverallminus[0] = \lim\limits_{x_i\uparrow 0}\muoverall[x_i]$  by local linear regression using the individual score variable as the univariate regressor and without considering $\pscore$, as in the standard no-interference RDD. To do so, we solve 
\begin{equation*}
    \begin{split}
    &\hat{\beta}_{1}(h_n) = \argmin\limits_{b0,b1 \in \mathbbm{R}}\sum_i\mathbbm{1}(X_i \geq 0)(Y_i - b_0 - b_1X_i)^2K_{h_n}(X_i), \\
    &\hat{\beta}_{0}(h_n) = \argmin\limits_{b_0,b_1 \in \mathbbm{R}}\sum_i\mathbbm{1}(X_i < 0)(Y_i - b_0 - b_1X_i)^2K_{h_n}(X_i),
    \end{split}
\end{equation*}
The final estimator of $\overall$ is given by
\begin{equation}\label{eq:overallest}
    \overallest = e_1^T\hat{\beta}_{1}(h_n) - e_1^T\hat{\beta}_{0}(h_n)
\end{equation}
The following results establish consistency and asymptotic normality of $\overallest$.

\begin{theorem}\label{th:overallnormalapp}
Suppose Assumptions~\ref{ass:consistency}--\ref{ass:localdependence}, and Assumptions 
\ref{ass:regularity}, \ref{ass:commonpieces}, and~\ref{ass:kernel} in Supplementary Material~\ref{appendix:estimatoroverall} hold (with Assumption~\ref{ass:smoothness} replaced by Assumption~\ref{ass:smoothnessov}).  
If $nh_n \to \infty$, $h_n \to 0$, and $h_n = O(n^{-1/5})$, then
\[
\sqrt{nh_n}
\frac{\big(\overallest - \overall\big) - h_n^{2}B_{1,0}(h_n)}{\sqrt{V(h_n)}}
\xrightarrow{d} 
\mathcal{N}(0,1),
\]
where 
\[
B_{1,0}(h_n) = \Big(\frac{\muoverallderivplus[2]-\muoverallderivminus[2]}{2}\Big)e_1^T(\Gamma^{1})^{-1}\theta^{1} + o(1), 
\quad
V(h_n) =\; \frac{\limvarplusov + \limvarminusov}{\limdensityov^2}e_1^T(\Gamma^{1})^{-1}\Psi^{1}(\Gamma^{1})^{-1}e_1 + o(1)
\]
The exact form of $\Gamma^{1}$, $\theta^{1}$ and $\Psi^{1}$ is given in Supplementary Material \ref{appendix:estimator}.\\
Proof. \textup{See Supplementary Material~\ref{appendix:estimatoroverall}.}
\end{theorem}

\noindent The asymptotic distribution of $\overallest$ matches that under independent data in no-interference RDDs, with a bias depending on the second-order derivatives of $\muoverallplus$ and $\muoverallminus$ at $x_i = 0$, and an asymptotic variance depending on $\limvarplusov$ and $\limvarminusov$, which are the right and left limits of the variance of $Y_i$ conditional on $X_i=x_i$, and the marginal density $f(0)= f_{X_i}(0)$. Notably, this estimator achieves the $nh_n^5$ rate since the overall direct effects is defined on a subset of the multiscore space with codimension 1. 

A variance estimator can be constructed analogously to the estimator in Eq. \eqref{eq:varianceest}, replacing the distance measure with $X_i$ and using the corresponding regression residuals. This estimator accounts for the dependence among observations on each side and across the cutoff using the dependency graph. The difference between this estimator and the typical RDD heteroskedasticity-robust variance estimator \citep[e.g.][]{cct14} increases with the level of dependence in the data. These estimators coincide when $\bm{W}$ is diagonal (independent data).

Finally, a bias-corrected version of $\overallest$, denoted by $\overallestbc$, can be obtained using local quadratic estimators of the second-order derivatives of $\muoverall$, as described in \citet{cct14}.

\section{Additional Causal Estimands and Results}
\subsection{Boundary Point Average Causal Effects}\label{app:pointeff}

In Section \ref{sec:identification}, we have introduced boundary average causal effects as our main estimands of interest. These effects can be rewritten as averages of point effects, defined as the difference of potential outcome expectation conditional on specific points of the effective treatment boundary. Formally, we define boundary point average effect as follows: 
\begin{equation}\label{def:ace}
   \pointeff =  \CE{Y_i(d,g) - Y_i(d',g')}{(X_i, \pscore) = (\bar{x}_i, \bar{\bm{x}}_{\smallN_i})}
\end{equation}
with $d$, $d' \in \{0,1\}$, $g$, $g' \in \mathcal{G}_i,\, (\bar{x_i}, \bar{\bm{x}}_{\smallN_i}) \in \Frontier$, where the expectation is taken with respect to the distribution of potential outcomes conditional on the individual and neighborhood score, and the observed network under our model-based perspective. While boundary effects are informative about treatment effects on larger subpopulations than point effects, they aggregate over potentially heterogeneous individuals. Therefore, boundary point effects can be of interest to uncover individual treatment heterogeneity. 

Boundary point effects can be identified by a similar strategy as in Theorem \ref{th:cont} for boundary effects, by taking the difference of the observed outcome expectations conditional on the neighborhood around specific points of decreasing radius.
Specifically, let $\eball$ be a neighborhood of radius $\varepsilon$ around $(\bar{x_i}, \bar{\bm{x}}_{\smallN_i})$, for $(\bar{x_i}, \bar{\bm{x}}_{\smallN_i}) \in \Frontier$, containing all points within distance $\varepsilon$ around $(\bar{x_i}, \bar{\bm{x}}_{\smallN_i})$.

Further let $\eballright = \eball \cap \scorespace(d,g)$ and $\eballleft) = \eball \cap \mathcal{X}_{i\smallN_i}(d',g')$. Then if assumptions \ref{ass:pos} and \ref{ass:cont} hold, as well as assumptions \ref{ass:consistency} and \ref{ass:interfence}, it can be shown that boundary point effects are identified as:

\begin{equation}\label{eq:limitpointeffects}
\begin{split}
\pointeff =& 
    \lim_{\varepsilon \to 0} \CE{Y_i}{(X_i, \pscore) \in \eballright} \\
    -& \lim_{\varepsilon \to 0 } \CE{Y_i}{(X_i, \pscore) \in \eballleft}
\end{split}
\end{equation}
for all $d$, $d'\in \{0,1\}$, $g$, $g'\in \mathcal{G}_i$, and for all $(\bar{x}_i, \bar{\bm{x}}_{\smallN_i}) \in \Frontier$.

Finally, estimation can be conducted by local polynomial regression using the distance from the point of interest as the one-dimensional forcing variable. We refer to \cite{cattaneo2025} for the analysis of such point effects estimators in multivariate RDDs. The variance can be estimated using our network-robust variance estimator using the one-dimensional distance measure to the point of interest.

\subsection{Overall Indirect Effect}\label{appendix:overallindirect}

In Section \ref{sec:framework}, we have defined the boundary overall indirect effect as  
\begin{equation*}
    \begin{aligned}
 \tau_{indirect} = \sum_{d_i} 
 \sum_{\bm d_{\smallN_i}}
\!\!\!\! \;\sum_{\substack{ \: \:\bm{d}_{\smallN_i}^{\prime}:\\\, d_j'\ge d_j \, \forall j\in \smallN_i, \\ 
\sum_{j\in \smallN_i} |d_j^{\prime} - d_j| = 1}}
&\CE{Y_i(d_i, g(\bm{d}^{\prime}_{\smallN_i}))-Y_i(d_i, g(\bm{d}_{\smallN_i}))}{(X_i, \pscore) \in \ell\big((d_i,\bm{d}_{\smallN_i}'),(d_i, \bm{d}_{\smallN_i})\big)}\\[-2em]
&\quad \cdot \CPrr{D_i=d_i, \bm{D}_{\smallN_i}'=\bm{d}_{\smallN_i}'}{\exists j \in \mathcal{S}_i: X_j=c}
    \end{aligned}
\end{equation*}
%
%where $\mathbf{d}_{\smallN_i,-k}$ denotes the vector of neighbors' treatments excluding neighbor $k$.  

To clarify the interpretation of this estimand, consider the case of the \emph{sum-of-treated} exposure mapping such that $G_i = \sum_{j \in \mathcal{S}_i} D_j$. Under this mapping, the estimand simplifies to
\begin{equation}
\tau_{indirect}=
\sum_{\substack{d\in \{0,1\}\\ g \in \{0,..., |\smallN_i| - 1\}}} \kern-1em\tau\big(\bar{\mathcal{X}}_{i\smallN_i}(d,\, g+ 1| d,\, g)\big)\cdot \CPrr{(X_i , \pscore) \in \bar{\mathcal{X}}_{i\smallN_i}(d,\, g+ 1| d,\, g)}{\exists j \in \mathcal{S}_i : X_j = c}
\end{equation}
which represents the weighted average of the boundary indirect effects 
$\tau\big(\bar{\mathcal{X}}_{i\smallN_i}(d, g+1 \mid d, g)\big)$—that is, the effect of increasing the neighborhood treatment level from $g$ to $g+1$ for units lying on the corresponding effective treatment boundary—weighted by the probability of being at such boundary conditional on having at least one neighbor at the cutoff.  

Under \emph{one-treated} exposure mapping, the estimand becomes:
\begin{equation}
\tau_{indirect}=
\sum_{d \in \{0,1\}} \tau\big(\bar{\mathcal{X}}_{i\smallN_i}(d,\, 1\,|\, d,\, 0)\big)\cdot \CPrr{(X_i , \pscore) \in \bar{\mathcal{X}}_{i\smallN_i}(d,\, 1| d,\, 0)}{\exists j \in \mathcal{S}_i : X_j = c},
\end{equation}
i.e., the weighted average of the boundary indirect effects of having at least one treated neighbor versus none, for both treated and untreated units.

Let $X_{\smallN_i}^{min} = X_{j^*}$, where $j^* = \argmin_{j \in \smallN_i} |X_j - c|$ denote the score of the neighbor closest to the cutoff. We denote its generic value by $x_{\smallN_i}^{\min}$.
Geometrically, $|X_{\smallN_i}^{\min} - c|$ represents the orthogonal distance from the point $\bm{X}_{\smallN_i}$ to the subspace of $\scorespace$ where at least one component of $\bm{x}_{\smallN_i}$ equals $c$.

The overall indirect effect is identified by 
\[\lim_{x_{\smallN_i}^{min} \downarrow c}\CE{Y_i}{X_{\smallN_i}^{min} = x_{\smallN_i}^{min}} - \lim_{x_{\smallN_i}^{min} \uparrow c}\CE{Y_i}{X_{\smallN_i}^{min} = x_{\smallN_i}^{min}}
\]
under Assumptions~\ref{ass:consistency}–\ref{ass:identification}. This result follows easily from arguments analogous to those in Theorem~\ref{th:cont} and Theorem~\ref{th:overall}, and is thus omitted.   
Based on this identification, $\tau_{indirect}$ can be estimated via univariate local linear regression using $X_{\smallN_i}^{min}$ as the one-dimensional regressor:
\begin{equation}
    \hat{\tau}_{indirect}(h_n) = e_1^T\hat{\beta}_{1,indirect}(h_n) - e_1^T\hat{\beta}_{0,indirect}(h_n)
\end{equation}
where 
\begin{equation*}
    \begin{split}
    &\hat{\beta}_{1,indirect}(h_n) = \argmin\limits_{b0,b1 \in \mathbbm{R}}\sum_i\mathbbm{1}(X^{min}_{\smallN_i} \ge 0)(Y_i - b_0 - b_1X^{min}_{\smallN_i})^2K_{h_n}(X^{min}_{\smallN_i}), \\
    &\hat{\beta}_{0,indirect}(h_n) = \argmin\limits_{b0,b1 \in \mathbbm{R}}\sum_i\mathbbm{1}(X^{min}_{\smallN_i} < 0)(Y_i - b_0 - b_1X^{min}_{\smallN_i})^2K_{h_n}(X^{min}_{\smallN_i}),
    \end{split}
\end{equation*}
letting $c = 0$.

Let $\mu_{1, indirect}(x^{min}_{\smallN_i}) = \CE{Y_i}{X_{\smallN_i}^{min} = x^{min}_{\smallN_i}}$ for $x^{min}_{\smallN_i} \ge 0$, and $\mu_{0, indirect}(x^{min}_{\smallN_i}) = \CE{Y_i}{X_{\smallN_i}^{min} = x^{min}_{\smallN_i}}$ for $x^{min}_{\smallN_i} \le 0$. 
\begin{theorem}
Suppose Assumptions~\ref{ass:consistency}--\ref{ass:localdependence} hold. Further, suppose that Assumptions 
\ref{ass:regularity}, \ref{ass:commonpieces}, and~\ref{ass:kernel} in Supplementary Material~\ref{appendix:estimatoroverall} hold, but replacing Assumption~\ref{ass:smoothness} with: $\mu_1(x^{min}_{\smallN_i})$ and $\mu_0(x^{min}_{\smallN_i})$ are $3$-times continuously differentiable.  
If $nh_n \to \infty$, $h_n \to 0$, and $h_n = O(n^{-1/5})$, then
\[
\sqrt{nh_n}
\frac{\big(\hat{\tau}_{indirect}(h_n) - \tau_{indirect}\big) - h_n^{2}B_{indirect}(h_n)}{\sqrt{V_{indirect}(h_n)}}
\xrightarrow{d} 
\mathcal{N}(0,1),
\]
where $B_{indirect}(h_n) = O(1)$ and $V_{indirect}(h_n) = O(1)$.\\
% \[
% B_{indirect}(h_n) = \Big(\frac{\mu_{1, indirect}^{(2)}(0)-\mu_{0, indirect}^{(2)}(0)}{2}\Big)e_1^T(\Gamma^{1})^{-1}\theta^{1} + o(1), 
% \]
%and
% \[V_{indirect}(h_n) =\; \frac{\bar{\omega}_{1,indirect}(0) + \bar{\omega}_{0,indirect}(0)}{f_{indirect}(0)^2}e_1^T(\Gamma^{1})^{-1}\Psi^{1}(\Gamma^{1})^{-1}e_1 + o(1)
% \]
%
% The exact form of $\Gamma^{1}$, $\theta^{1}$ and $\Psi^{1}$ is given in Supplementary Material \ref{appendix:estimator}.\\
Proof. \textup{The proof follows analogous arguments as those in Theorem \ref{th:asynormal} and \ref{th:overallnormalapp}, and thus, is omitted for brevity.}
\end{theorem}

% Similarly as in Theorem \ref{th:asynormaltauov}, the estimator $\hat{\tau}_{indirect}(h_n)$ is asymptotically normal, with a bias depending on the second-order derivatives of the outcome regression functions conditional on $X^{min}_{\smallN_i}$ at $x^{min}_{\smallN_i} = 0$, and an asymptotic variance depending on $\bar{\omega}_{1,indirect}(0)$ $\bar{\omega}_{0,indirect}(0)$, which include the limits of the variance of $Y_i$ conditional on $X_{\smallN_i}^{min}$ integrated over the space where at least one neighbor has the score at the cutoff, and the density $f_{indirect}(0)$, the integral of $f\ppoint$ on that space. 

Importantly, this estimator achieves the $nh_n^5$ rate. Specifically, $\hat{\tau}_{indirect}(h_n)$ averages observations in a neighborhood of the subset of $\scorespace$ where at least one component of $\pscore$ equals $c$. Since this subset is itself a boundary formed by a union of linear pieces, its properties follow from arguments analogous to those used for estimating boundary and overall direct effects.  
The codimension of this subset is one, implying an asymptotic variance of order $O\big((nh_n)^{-1}\big)$ and the usual RDD convergence rate. Thus, while estimators of boundary indirect effects $\boundeff$ comparing specific values $g$ and $g'$ may converge more slowly, this aggregate measure attains the canonical fast rate of standard RDDs.

\section{Additional Simulation Results}\label{appendix:simulations}

\subsection{Network Data}

In this subsection, we present a simulation study to evaluate the finite-sample performance of $\hat{\tau}^{bc}_{1|0}(h_n, b_n)$ and $\estimatorbc$ under network interference with overlapping interference sets. Specifically, we consider scenarios where each unit's interference set coincides with its network neighborhood—that is, the set of nodes directly linked to it. The neighborhood treatment $G_i$ is defined via the one-treated exposure mapping.

For sample sizes $n = \{750, 1500, 3000\}$, we simulate small-world networks \citep{wattstrogatz} using the \texttt{sample\_smallworld()} function from the R package \texttt{igraph}. Small-world networks are characterized by high clustering, meaning that two nodes sharing a neighbor tend to be connected. We fix the average node degree at 4 by setting the argument \texttt{nei = 2}, and vary the rewiring probability to generate networks with different levels of clustering, as measured by the global and average local clustering coefficients.
The global clustering coefficient is defined as the ratio of the number of closed triplets (triangles) to the number of connected triplets in the network. The average local clustering coefficient averages the local clustering coefficients for each node, which is the ratio of the triangles connected to the node and the triples centered on the node.

This simulation design allows us to assess the performance of the proposed estimators in network settings and to investigate how network clustering affects performance—particularly through the induced clustering in the distance variable.

We consider two scenarios:

\begin{itemize}
\item[] \textbf{Scenario A}: Rewiring probability $p = 0.15$, resulting in a global clustering coefficient of approximately $0.16$ and an average local clustering coefficient of about $0.20$.
\item[] \textbf{Scenario B}: Rewiring probability $p = 0.05$, resulting in a global clustering coefficient of approximately $0.35$ and an average local clustering coefficient of about $0.37$.
\end{itemize}
Outcomes are simulated from the model 
\begin{equation}\label{mod:simappendix}
        Y_i = 0.5 + 1.5D_i + G_i + 0.5X_i + 4.3D_iX_i^2 - 1.5(1 - D_i)X_i^2 + 0.3\bar{\bm{X}}_{\smallN_i}  + \varepsilon_i
\end{equation}

\noindent
where $X_i$ is i.i.d. a truncated normal with mean -0.5 and variance 1, and upper and lower bound -5 and 5, while the error terms are given by $\varepsilon_i = D_i\big(2\frac{\sum_{j\in\smallN_i}u_j}{|\mathcal{S}_i|} + u_i\big) - 1.4(1 -D_i)\cdot \big(2\frac{\sum_{j\in\smallN_i}u_j}{|\mathcal{S}_i|} + u_i\big)$ with $u_i \overset{i.i.d.}{\sim} \mathcal{N}(0,1)$. Observations are thus dependent up to second-order network neighbors (second-order dependence), and the boundary average effects are
homogeneous across units.

Simulation results are reported in Tables \ref{tab:net_lowclus} (Scenario A) and \ref{tab:net_highclust} (Scenario B). Each table reports the empirical bias, empirical standard deviation, estimated standard error (using both our proposed variance estimator and the standard i.i.d. estimator), and the associated confidence interval coverage rates. We also report the average effective sample sizes ($N_{d,g}$ and $N_{d',g'}$) and the proportion of units with unique score variables and minimum distance values (column \qq\% Unique"). Values less than one in this column indicate overlapping distance variables among units.

According to the results, the proposed estimators are virtually unbiased across all sample sizes and scenarios. The standard deviation decreases substantially with sample size in both settings. Notably, $\hat{\tau}^{bc}_{1|0}(h_n, b_n)$ consistently has the lowest standard deviation, due to a larger average effective sample size. In contrast, $\hat{\tau}_{10|00}(h_n, b_n)$ exhibits the highest standard deviation, driven by a smaller fraction of units with $(D_i = 1, G_i = 0)$.

The estimator $\hat{\tau}_{01|00}(h_n, b_n)$ has a relatively large effective sample size but still exhibits high variance. This is explained by the clustering structure of the distance variable: in Scenario A, approximately 80\% of units have unique distance values, while in Scenario B only 74\% do. This increase in overlap leads to higher standard deviation in Scenario B.

Our proposed variance estimator performs well, approaching the empirical standard deviation in large samples. Coverage rates using this estimator converge to the nominal level. In comparison, the i.i.d. confidence intervals tend to undercover the true value, especially for smaller samples, although the coverage improves with larger sample sizes. For $\hat{\tau}_{01|00}(h_n, b_n)$, however, the coverage does not improve in large samples and it is substantially worse in Scenario B, with higher clustering in the network. 
Overall, our variance estimator appears more accurate than the one relying on the i.i.d. assumption, especially in Scenario B with higher clustering.  

In conclusion, this simulation study demonstrates an overall good performance of the proposed distance-based estimators and the associated variance estimator. The study also highlights how increased clustering in the network can induce higher clustering in the distance variable. When this occurs, relying on the i.i.d. variance estimator leads to consistently poor coverage, whereas accounting for dependence significantly improves coverage.

\begin{table}[H]
    \centering
    \caption*{{\textbf{Scenario A}}}
    \resizebox{0.8\textwidth}{!}{
    \begin{tabular}{llcccccccccc}

              \hline

    & & Bias & S.D. & S.E. & S.E.$_{i.i.d.}$ & C.R. & C.R.$_{i.i.d.}$ & $\bar{N}_{d,g}$ & $\bar{N}_{d',g'}$ & \% Unique  \\ 

    \midrule 
 
     \multirow{3}{*}{n = 750}& $ \hat{\tau}^{bc}_{1|0}(h_n, b_n)$  &   0.027  &   1.156  &   1.053  &   0.960  &   0.933  &   0.910  & 134.551  & 183.500  &   1.000  \\
~&$ \hat{\tau}^{bc}_{10|00}(h_n, b_n)$  &   0.027  &   2.539  &   2.060  &   2.054  &   0.880  &   0.877  &  30.739  &  41.192  &   1.000  \\
~&$ \hat{\tau}^{bc}_{01|00}(h_n, b_n)$  &  -0.027  &   2.313  &   1.974  &   1.893  &   0.902  &   0.900  & 113.716  &  76.904  &   0.795  \\
\midrule 
\multirow{3}{*}{n = 1500}& $ \hat{\tau}^{bc}_{1|0}(h_n, b_n)$  &   0.047  &   0.787  &   0.756  &   0.680  &   0.944  &   0.906  & 263.448  & 357.809  &   1.000  \\
~&$ \hat{\tau}^{bc}_{10|00}(h_n, b_n)$  &   0.038  &   1.674  &   1.474  &   1.441  &   0.920  &   0.913  &  64.333  &  87.464  &   1.000  \\
~&$ \hat{\tau}^{bc}_{01|00}(h_n, b_n)$  &  -0.039  &   1.588  &   1.414  &   1.317  &   0.927  &   0.915  & 234.410  & 159.957  &   0.798  \\
\midrule 
\multirow{3}{*}{n = 3000}& $ \hat{\tau}^{bc}_{1|0}(h_n, b_n)$  &   0.038  &   0.571  &   0.541  &   0.487  &   0.941  &   0.913  & 500.205  & 662.241  &   1.000  \\
~&$ \hat{\tau}^{bc}_{10|00}(h_n, b_n)$  &   0.032  &   1.149  &   1.050  &   1.024  &   0.934  &   0.929  & 129.772  & 175.393  &   1.000  \\
~&$ \hat{\tau}^{bc}_{01|00}(h_n, b_n)$  &   0.038  &   1.059  &   0.982  &   0.900  &   0.948  &   0.925  & 504.572  & 334.086  &   0.797  \\
 \midrule 
 \end{tabular} 
  }
 \caption{Simulation results using bias correction with small-world network and one treated exposure mapping with rewiring probability $p = 0.15$. One thousand replications. 
 S.D. = empirical standard error. S.E. = estimated standard error.
 S.E.$_{i.i.d.}$ = estimated standard error with $i.i.d.$ heteroskedasticity-robust HC0 plug-in residuals variance estimator.
 C.R. = coverage rate. C.R.$_{i.i.d.}$ = coverage rate corresponding to the $i.i.d.$ heteroskedasticity-robust HC0 plug-in residuals variance estimator.
 $N_{d,g}$ and $N_{d',g'}$ = effective sample size on each side of the treatment boundary.
 \% Unique = percentage of unique distance variables.}
    \label{tab:net_lowclus}
\end{table}

% Table with high clusterization
\begin{table}[H]
\caption*{{\textbf{Scenario B}}}
    \centering
    \resizebox{0.8\textwidth}{!}{
 \begin{tabular}{llcccccccccc}

              \hline

    & & Bias & S.D. & S.E. & S.E.$_{i.i.d.}$ & C.R. & C.R.$_{i.i.d.}$ & $\bar{N}_{d,g}$ & $\bar{N}_{d',g'}$ & \% Unique  \\ 

    \midrule 
 
     \multirow{3}{*}{n = 750}& $ \hat{\tau}^{bc}_{1|0}(h_n, b_n)$  &  -0.019  &   1.077  &   1.036  &   0.943  &   0.930  &   0.906  & 134.216  & 184.242  &   1.000  \\
~&$ \hat{\tau}^{bc}_{10|00}(h_n, b_n)$  &   0.036  &   2.461  &   2.005  &   1.992  &   0.901  &   0.904  &  29.272  &  39.542  &   1.000  \\
~&$ \hat{\tau}^{bc}_{01|00}(h_n, b_n)$  &   0.046  &   2.609  &   2.133  &   1.942  &   0.897  &   0.875  & 102.775  &  73.005  &   0.741  \\
\midrule 
\multirow{3}{*}{n = 1500}& $ \hat{\tau}^{bc}_{1|0}(h_n, b_n)$  &  -0.031  &   0.792  &   0.739  &   0.667  &   0.928  &   0.899  & 263.827  & 355.330  &   1.000  \\
~&$ \hat{\tau}^{bc}_{10|00}(h_n, b_n)$  &  -0.103  &   1.627  &   1.427  &   1.399  &   0.903  &   0.897  &  61.228  &  83.298  &   1.000  \\
~&$ \hat{\tau}^{bc}_{01|00}(h_n, b_n)$  &  -0.070  &   1.722  &   1.531  &   1.355  &   0.922  &   0.888  & 213.644  & 149.110  &   0.741  \\
\midrule 
\multirow{3}{*}{n = 3000}& $ \hat{\tau}^{bc}_{1|0}(h_n, b_n)$  &   0.002  &   0.555  &   0.532  &   0.477  &   0.943  &   0.909  & 501.494  & 663.855  &   1.000  \\
~&$ \hat{\tau}^{bc}_{10|00}(h_n, b_n)$  &  -0.028  &   1.068  &   1.015  &   0.985  &   0.941  &   0.934  & 123.655  & 168.285  &   1.000  \\
~&$ \hat{\tau}^{bc}_{01|00}(h_n, b_n)$  &   0.016  &   1.198  &   1.083  &   0.942  &   0.937  &   0.887  & 445.984  & 305.441  &   0.738  \\
 \midrule 
 \end{tabular}}
 \caption{Simulation results using bias correction with small-world network and one treated exposure mapping with rewiring probability $p = 0.05$. One thousand replications. 
 S.D. = empirical standard error. S.E. = estimated standard error.
 S.E.$_{i.i.d.}$ = estimated standard error with $i.i.d.$ heteroskedasticity-robust HC0 plug-in residuals variance estimator.
 C.R. = coverage rate. C.R.$_{i.i.d.}$ = coverage rate corresponding to the $i.i.d.$ heteroskedasticity-robust HC0 plug-in residuals variance estimator.
 $N_{d,g}$ and $N_{d',g'}$ = effective sample size on each side of the treatment boundary.
 \% Unique = percentage of unique distance variables.}
    \label{tab:net_highclust}
\end{table}

\subsection{Varying Group Size}

In this simulation study, we consider a scenario with equally sized groups. 
We keep the total sample size fixed at $n = 3000$ and vary the cluster size, denoted by $M$. 
Data are generated as Section \ref{sec:simulation}, but using the one-treated exposure mapping.

The objective is to assess the performance of our proposed bias-corrected estimators in settings with larger group sizes, which correspond to higher-dimensional multiscore spaces and effective treatment boundaries than those considered in Section~\ref{sec:simulation}. The dimension of the multiscore space for each unit is, in fact, given by $M$. Under this data generating process, although the total sample size remains constant, the probability of observing certain neighborhood-treatment configurations (e.g., $G_i=0$) decreases with $M$, reducing the effective sample size available for estimation near each boundary.

We simulate 1,000 datasets with group sizes $M \in \{3,4,5,6\}$ and total sample size $n = 3000$, corresponding to $\{1000, 750, 600, 500\}$ groups, respectively. 

We consider, for brevity, the estimators $\hat{\tau}^{bc}_{1|0}(h_n, b_n)$, $\hat{\tau}^{bc}_{10|00}(h_n, b_n)$, and $\hat{\tau}^{bc}_{01|00}(h_n, b_n)$,\footnote{The bandwidths $h_n$ and $b_n$ are computed using the plug-in procedure by \citet{cct14}.} and report the results in Table~\ref{tab:mc_one_fixednumber}. 
All estimators are approximately unbiased across different group sizes. 
The estimators $\hat{\tau}_{10|00}^{bc}(h_n, b_n)$ and $\hat{\tau}^{bc}_{01|00}(h_n, b_n)$ remain approximately unbiased for $M = \{3,4,5,6\}$ but exhibit increasing standard deviations as the group size grows. 
The increase in the empirical standard deviation is more pronounced for $\hat{\tau}_{01|00}^{bc}(h_n, b_n)$, due to the high percentage of observations sharing the same distance measure, as indicated in column ``\% Unique.'' 
Our variance estimator for $\hat{\tau}_{10|00}^{bc}(h_n, b_n)$ and $\hat{\tau}^{bc}_{01|00}(h_n, b_n)$ is accurate for smaller group sizes ($M = \{3,4\}$) but worsens in performance for larger groups, resulting in lower coverage rates. 
In contrast, the variance estimator for $\hat{\tau}^{bc}_{1|0}(h_n, b_n)$ remains relatively accurate across group sizes.

The high standard deviation of $\hat{\tau}_{10|00}^{bc}(h_n, b_n)$ and $\hat{\tau}^{bc}_{01|00}(h_n, b_n)$, together with the worsening performance of their variance estimators, arises from the reduced effective sample size. 
In our data generating process, larger groups lead to lower observed probabilities for some neighborhood treatment configurations. 
In particular, the observed probabilities $\Pr(G_i = 0)$ equal approximately $\{0.38, 0.23, 0.14, 0.09\}$ as group size increases.

To illustrate the impact of the effective sample size, we repeat the simulation focusing on $\hat{\tau}^{bc}_{01|00}(h_n, b_n)$ but choose the cutoff
\[
    c = -0.3 + \Phi^{-1}\!\big(0.35^{1/(M-1)}\big),
\]
which ensures that the observed probability $\Pr(G_i = 0) \approx 0.35$ for each group size $M$. 
This adjustment keeps a larger effective sample size for estimation. 
As shown in Table~D.4, this modification substantially reduces the estimator's standard error relative to Table~D.3. 
Moreover, our variance estimator provides more accurate variance estimates and improved coverage, even in the presence of substantial clustering at the distance-measure level.

Overall, the results show that while our estimation method yields accurate inference when the effective sample size is sufficient, large groups may lead to sparse data within each effective treatment arm and thus less precise inference.
Nevertheless, our results indicate that even if specific boundary effects cannot be precisely estimated due to limited observations, the boundary overall direct effect can still be estimated accurately when the total sample size is large, as in this setting.

\begin{table}[H]
\centering
\resizebox{0.8\textwidth}{!}{
\begin{tabular}{llcccccccc}

            \hline

  & & Bias & S.D. & S.E. & C.R. & $\bar{N}_{d,g}$ & $\bar{N}_{d',g'}$ & \% Unique  \\ 

  \midrule 
 
   \multirow{3}{*}{M = 3}& $ \hat{\tau}^{bc}_{1|0}(h_n, b_n)$  &  -0.013  &   0.651  &   0.639  &   0.950  & 603.549  & 723.666  &   1.000  \\
~&$ \hat{\tau}^{bc}_{10|00}(h_n, b_n)$  &   0.009  &   1.032  &   0.987  &   0.950  & 243.326  & 294.503  &   1.000  \\
~&$ \hat{\tau}^{bc}_{01|00}(h_n, b_n)$  &   0.039  &   1.402  &   1.280  &   0.929  & 481.672  & 411.999  &   0.637  \\
\midrule 
\multirow{3}{*}{M = 4}& $ \hat{\tau}^{bc}_{1|0}(h_n, b_n)$  &   0.010  &   0.552  &   0.552  &   0.944  & 585.236  & 695.398  &   1.000  \\
~&$ \hat{\tau}^{bc}_{10|00}(h_n, b_n)$  &   0.036  &   1.104  &   1.069  &   0.946  & 150.242  & 181.642  &   1.000  \\
~&$ \hat{\tau}^{bc}_{01|00}(h_n, b_n)$  &  -0.065  &   1.638  &   1.568  &   0.931  & 393.081  & 271.343  &   0.455  \\
\midrule 
\multirow{3}{*}{M = 5}& $ \hat{\tau}^{bc}_{1|0}(h_n, b_n)$  &  -0.026  &   0.509  &   0.504  &   0.958  & 575.230  & 681.489  &   1.000  \\
~&$ \hat{\tau}^{bc}_{10|00}(h_n, b_n)$  &  -0.034  &   1.324  &   1.221  &   0.928  &  92.785  & 111.590  &   1.000  \\
~&$ \hat{\tau}^{bc}_{01|00}(h_n, b_n)$  &   0.094  &   2.375  &   1.952  &   0.885  & 281.102  & 169.292  &   0.350  \\
\midrule 
\multirow{3}{*}{M = 6}& $ \hat{\tau}^{bc}_{1|0}(h_n, b_n)$  &  -0.018  &   0.482  &   0.473  &   0.938  & 565.136  & 668.042  &   1.000  \\
~&$ \hat{\tau}^{bc}_{10|00}(h_n, b_n)$  &  -0.020  &   1.507  &   1.408  &   0.929  &  56.543  &  68.610  &   1.000  \\
~&$ \hat{\tau}^{bc}_{01|00}(h_n, b_n)$  &  -0.016  &   2.939  &   2.388  &   0.888  & 188.998  & 105.040  &   0.284  \\
 \midrule 
 \end{tabular}  }
 \caption{Simulation results over one thousand replications.
 S.D. = empirical standard error. S.E. = estimated standard error.
 C.R. = coverage rate.  $N_{d,g}$ and $N_{d',g'}$ = effective sample size on each side of the treatment boundary.}
\label{tab:mc_one_fixednumber}
 \end{table}

 \begin{table}[H]
\centering
\resizebox{0.8\textwidth}{!}{
\begin{tabular}{llcccccccc}

            \hline

  & & Bias & S.D. & S.E. & C.R. & $\bar{N}_{d,g}$ & $\bar{N}_{d',g'}$ & \% Unique  \\ 

  \midrule 
 
   \multirow{1}{*}{M = 3}& $ \hat{\tau}^{bc}_{01|00}(h_n, b_n)$  &   0.018  &   1.438  &   1.344  &   0.942  & 448.701  & 368.789  &   0.642  \\
\midrule 
\multirow{1}{*}{M = 4}& $ \hat{\tau}^{bc}_{01|00}(h_n, b_n)$  &   0.041  &   1.382  &   1.280  &   0.942  & 526.895  & 436.620  &   0.439  \\
\midrule 
\multirow{1}{*}{M = 5}& $ \hat{\tau}^{bc}_{01|00}(h_n, b_n)$  &  -0.015  &   1.327  &   1.252  &   0.941  & 562.791  & 474.355  &   0.330  \\
\midrule 
\multirow{1}{*}{M = 6}& $ \hat{\tau}^{bc}_{01|00}(h_n, b_n)$  &   0.010  &   1.369  &   1.243  &   0.935  & 580.149  & 498.828  &   0.264  \\
 \midrule 
 \end{tabular}}
 \caption{Simulation results over one thousand replications. S.D. = empirical standard error. S.E. = estimated standard error.
 C.R. = coverage rate.  $N_{d,g}$ and $N_{d',g'}$ = effective sample size on each side of the treatment boundary.}
\label{tab:mc_one_fixedn}
 \end{table}

\end{appendices}

\end{document}
